# Supplementary material for: A comparison of Leja- and Krylov-based iterative schemes for Exponential Integrators
Source: arXiv:2211.08948 source file (2022-11-16)
Supplement: Supplementary file 1 [file supplement.pdf]

## Supplementary Material

This is a supplement to the paper “A comparison of Leja- and Krylov-based iterative schemes for Exponential Integrators” by P. J. Deka, M. Tokman, and L. Einkemmer. This supplement consists of the simulations results for the various integrators and problems that are not included in, but cited in the main manuscript. This is to adhere to the page limitations of the journal.

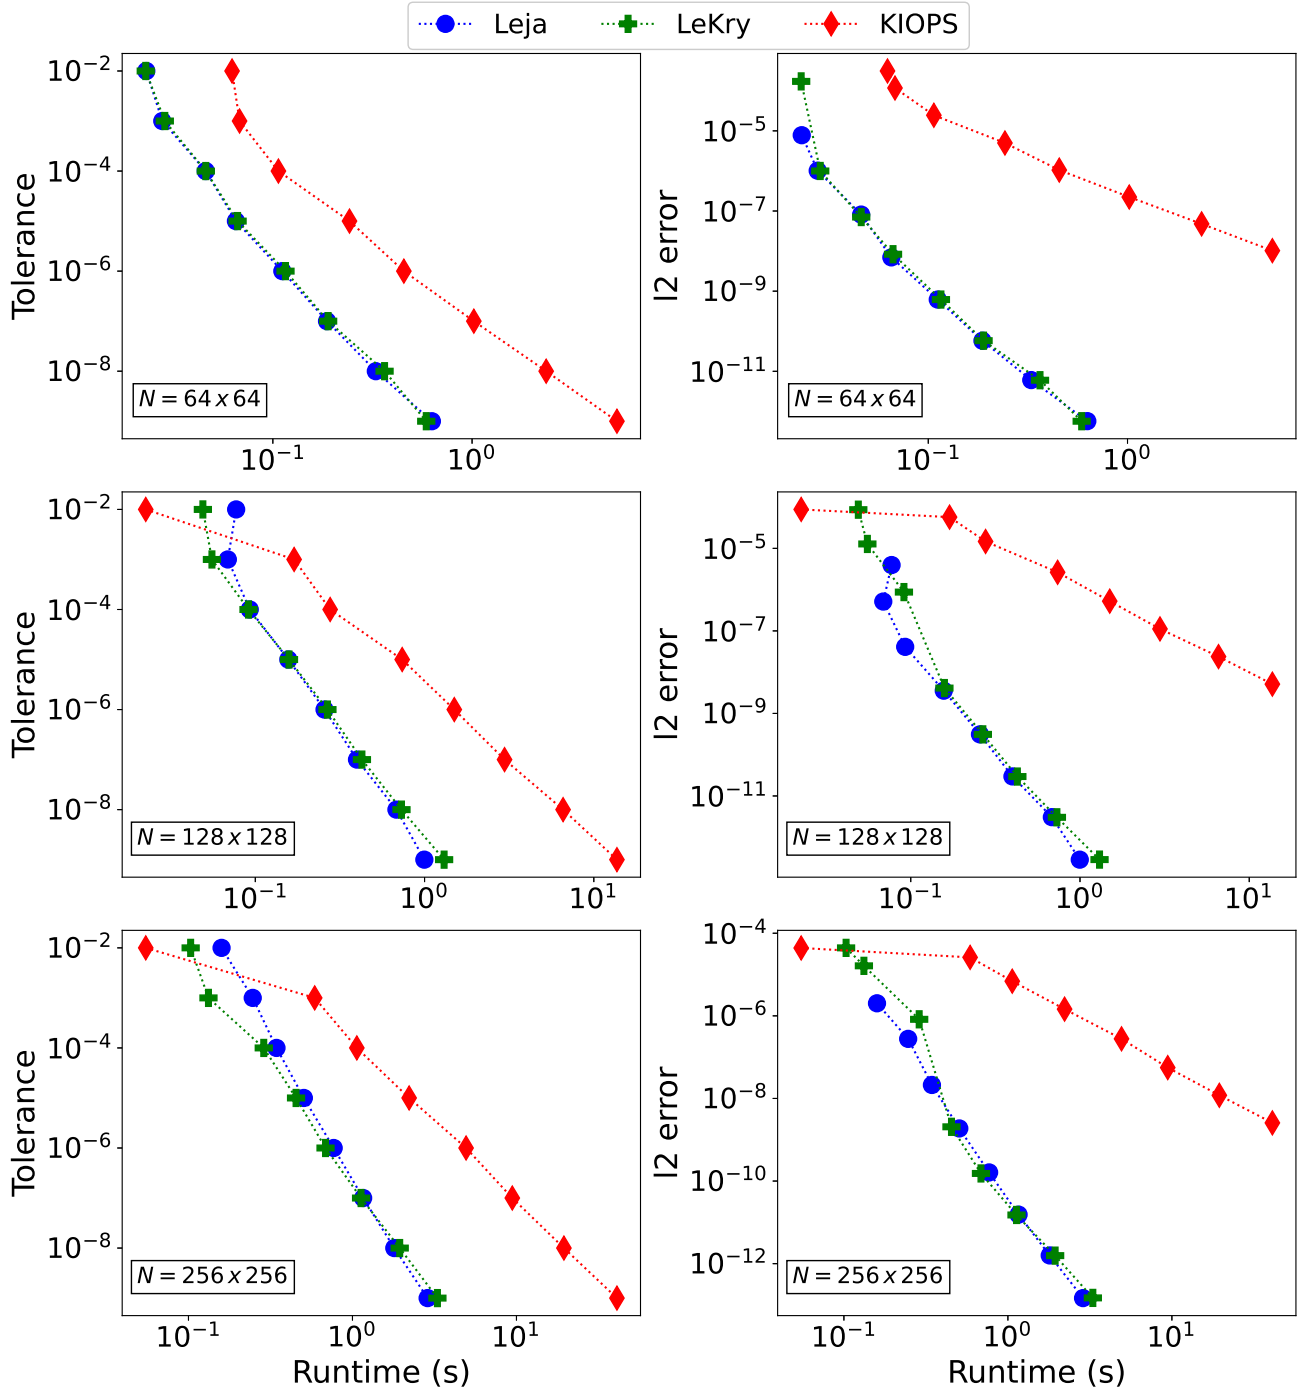

Figure 1: Comparison of the runtimes for a given value of tolerance (left panel) and the l2 norm of the global error incurred (right panel) for Leja (blue circles), LeKry (green pluses), and KIOPS (red diamonds) with the EPIRK4s3 integrator for the Allen–Cahn equation ( $\alpha = 0.001$ ).

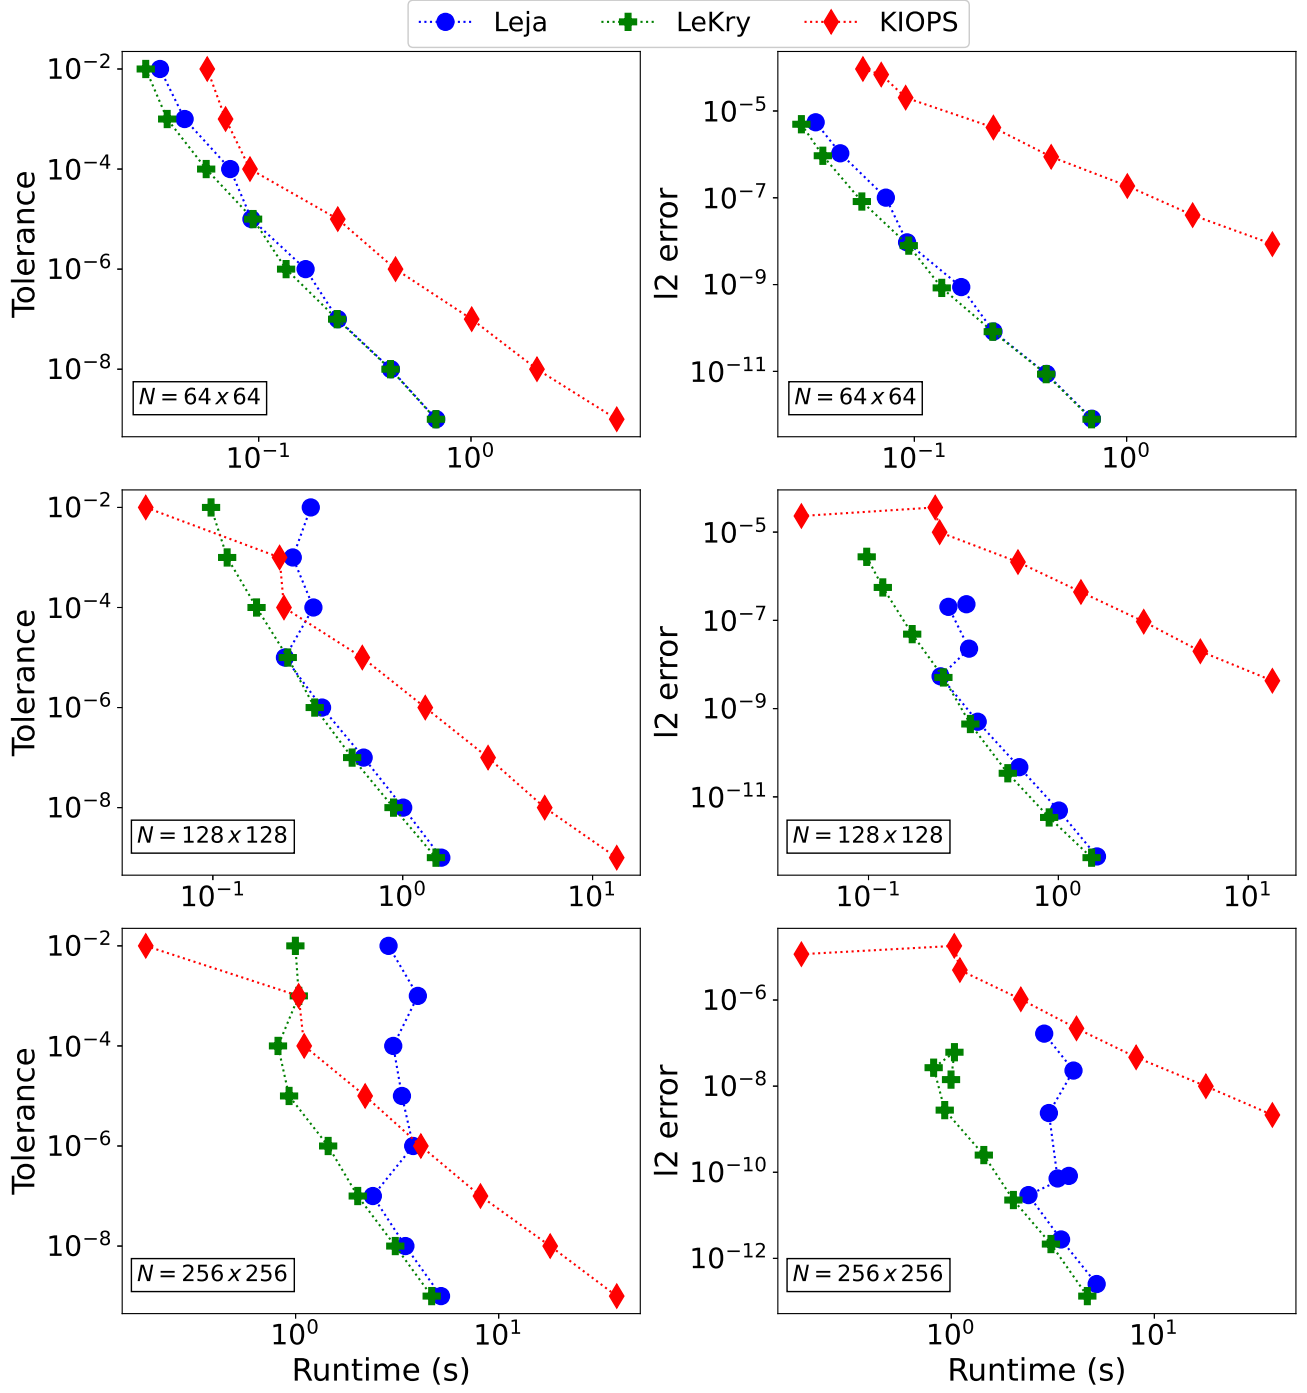

Figure 2: Comparison of the runtimes for a given value of tolerance (left panel) and the  $l_2$  norm of the global error incurred (right panel) for Leja (blue circles), LeKry (green pluses), and KIOPS (red diamonds) with the EPIRK4s3 integrator for the Allen-Cahn equation ( $\alpha = 0.01$ ).

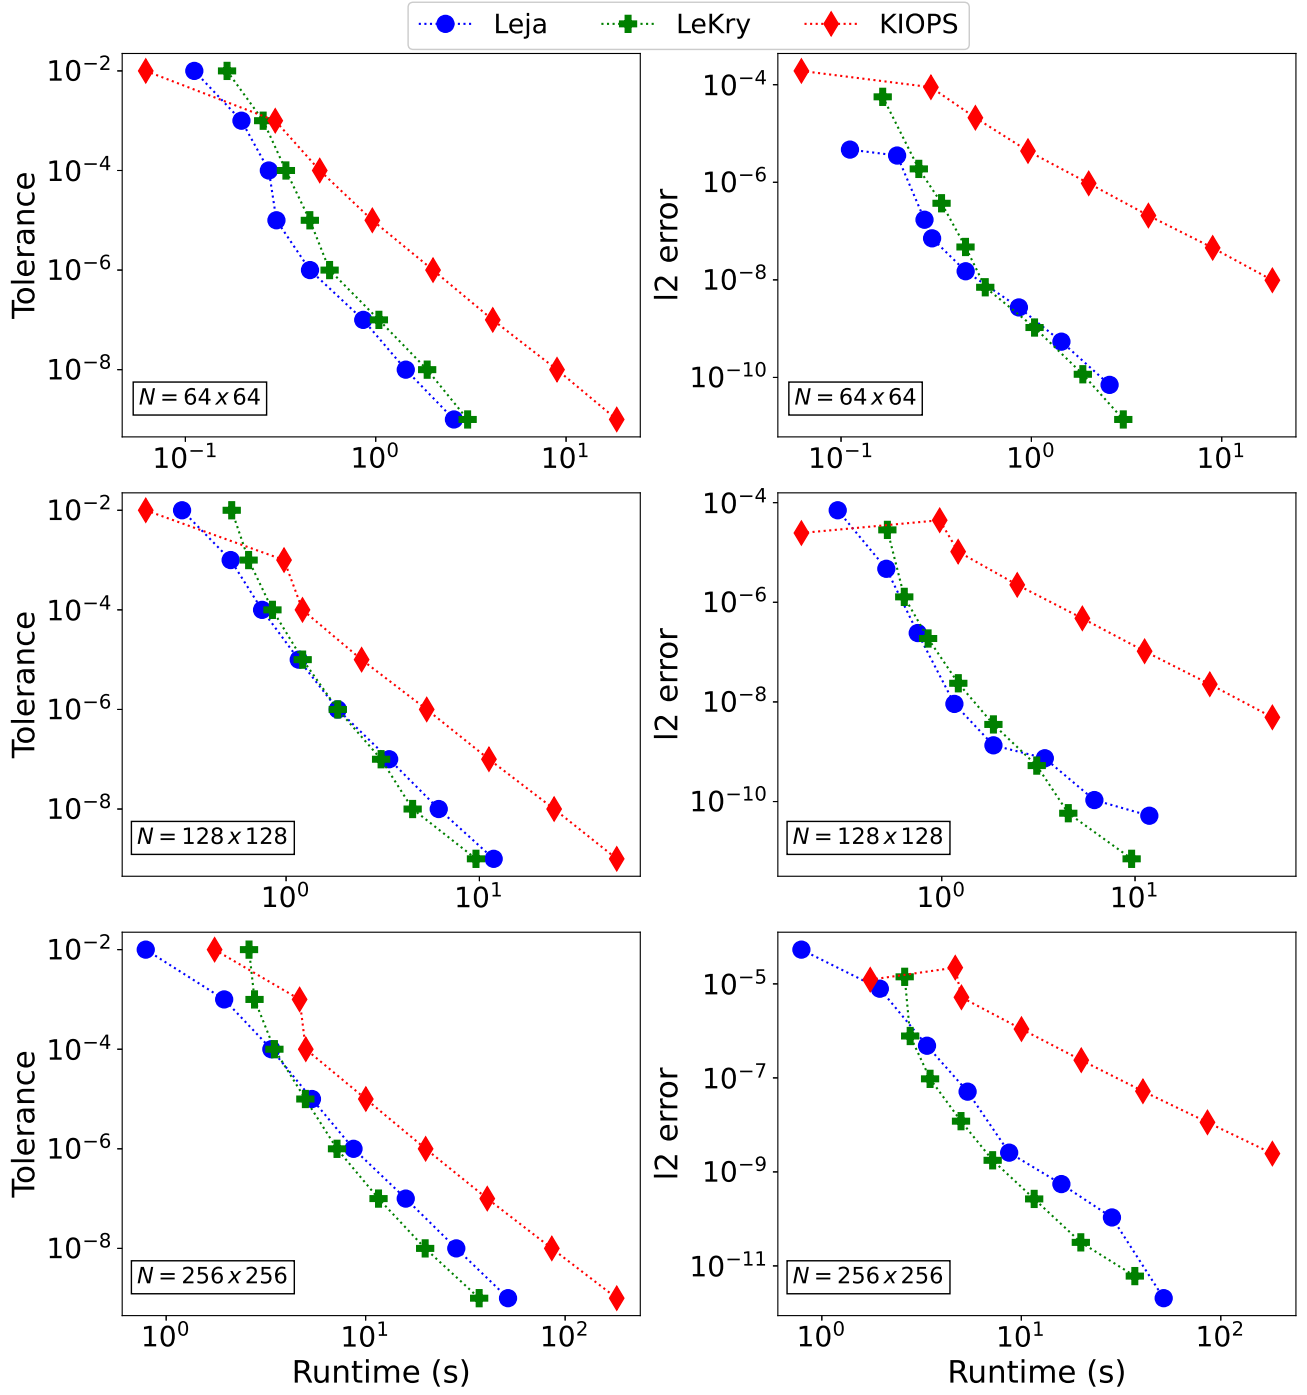

Figure 3: Comparison of the runtimes for a given value of tolerance (left panel) and the l2 norm of the global error incurred (right panel) for Leja (blue circles), LeKry (green pluses), and KIOPS (red diamonds) with the EPIRK4s3 integrator for the Allen–Cahn equation ( $\alpha = 0.1$ ).

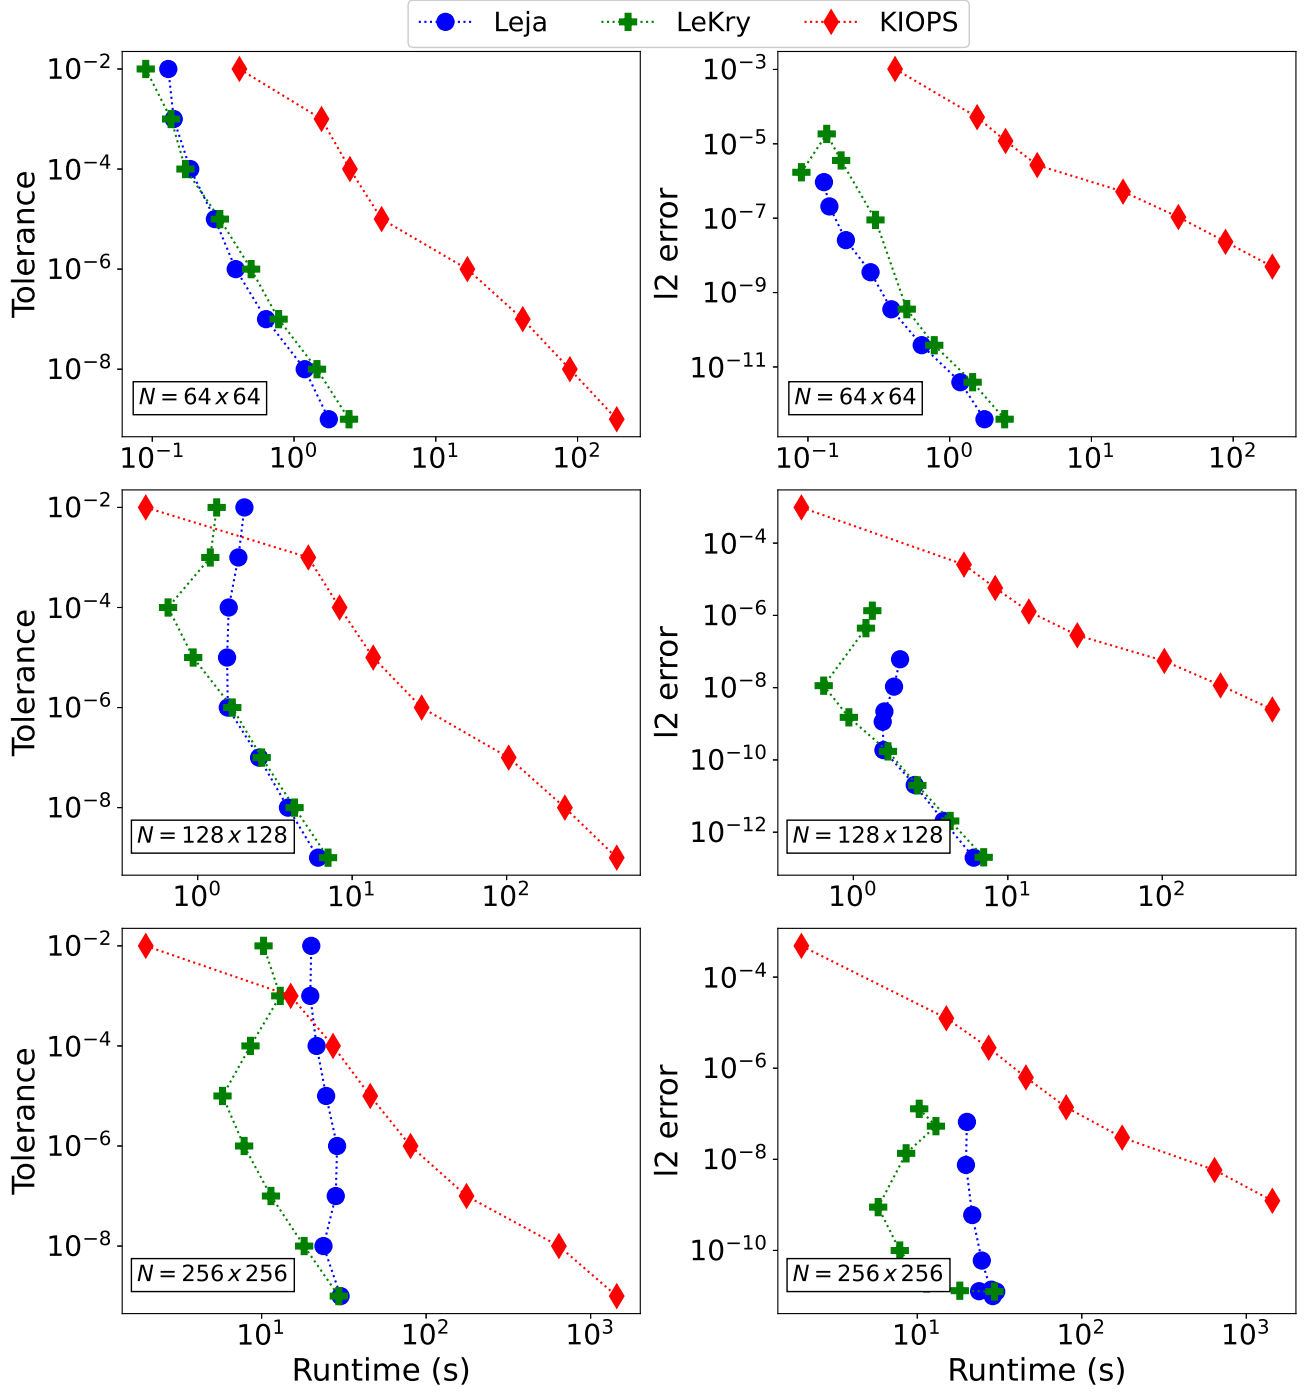

Figure 4: Comparison of the runtimes for a given value of tolerance (left panel) and the l2 norm of the global error incurred (right panel) for Leja (blue circles), LeKry (green pluses), and KIOPS (red diamonds) with the EPIRK4s3 integrator for the Brusselator equation ( $\alpha = 0.01$ ).

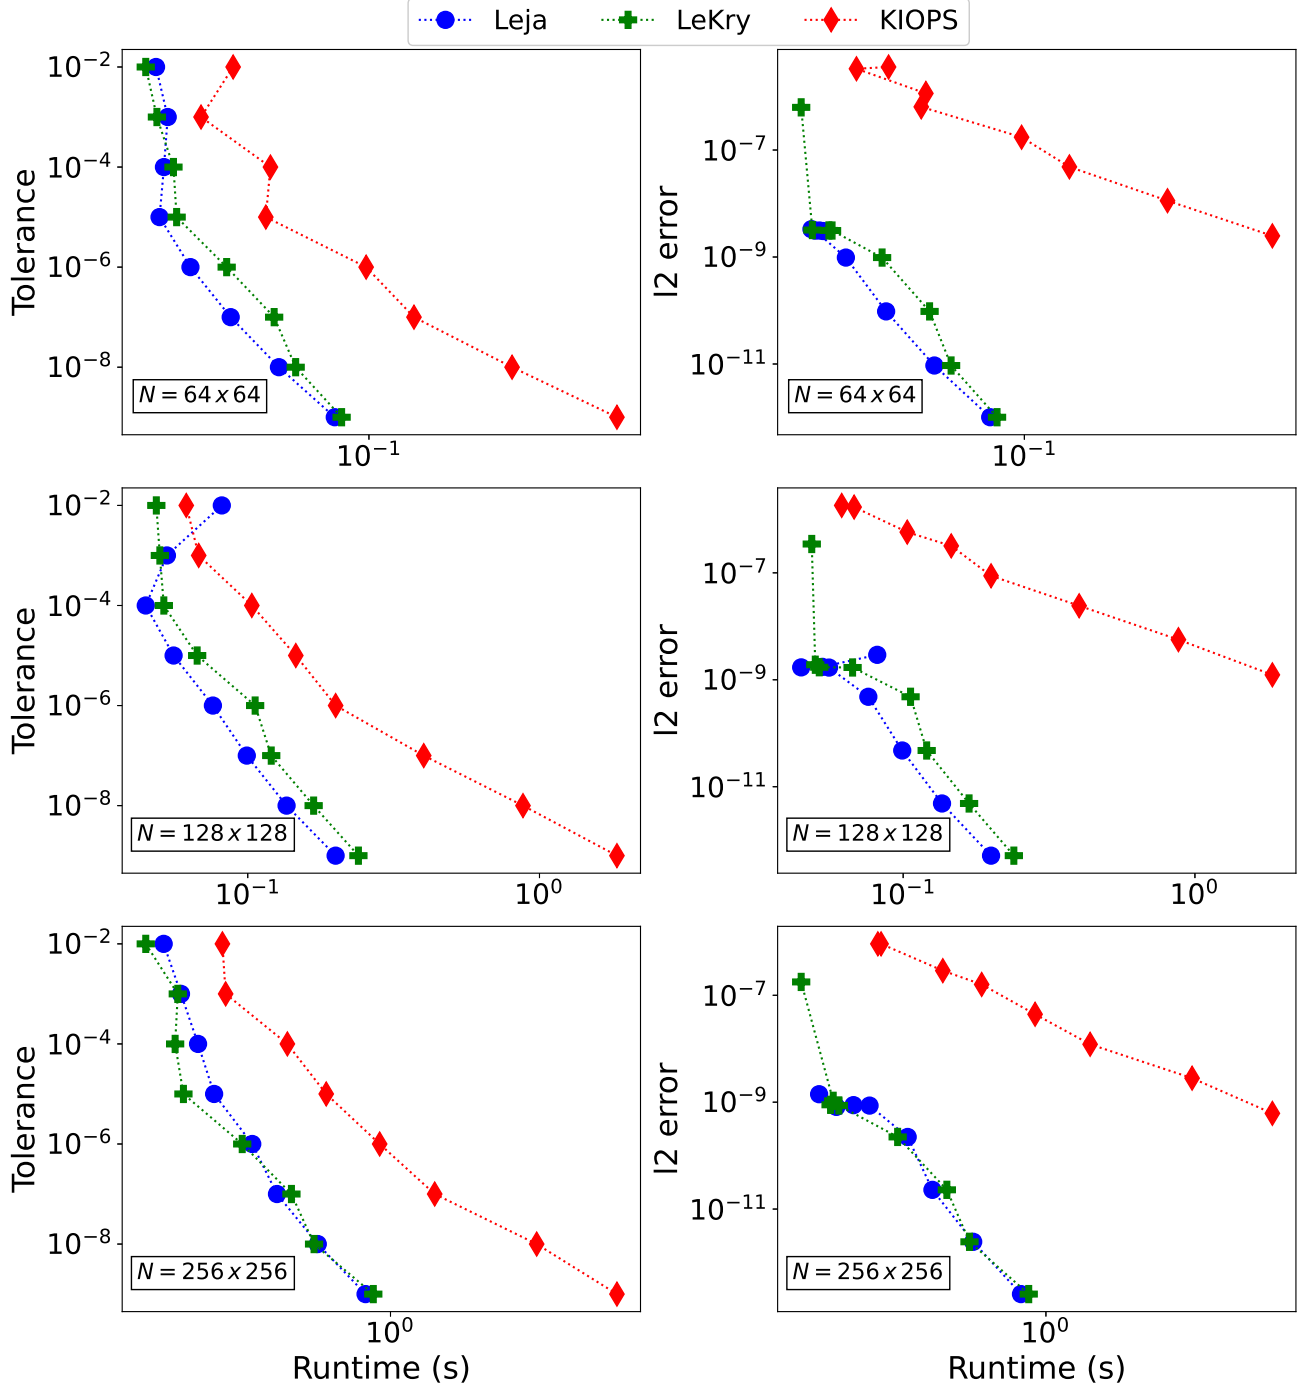

Figure 5: Comparison of the runtimes for a given value of tolerance (left panel) and the l2 norm of the global error incurred (right panel) for Leja (blue circles), LeKry (green pluses), and KIOPS (red diamonds) with the EPIRK4s3 integrator for the Gray-Scott equation ( $\alpha = 0.001$ ).

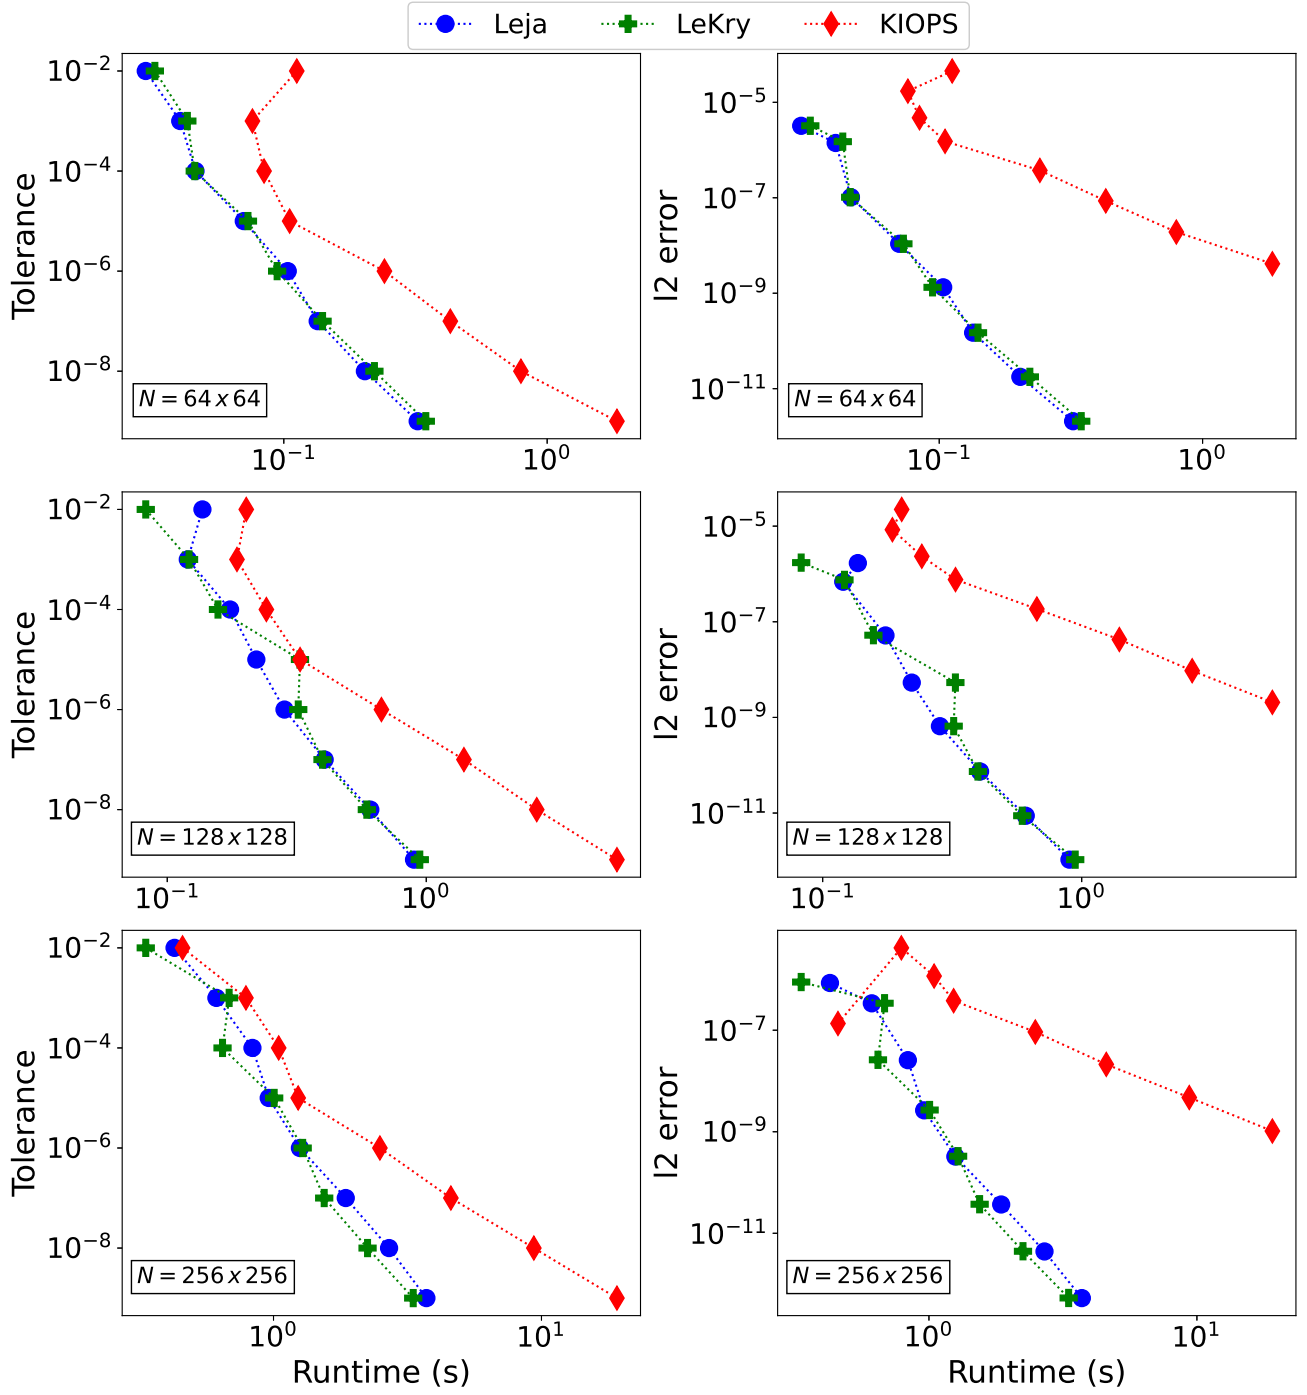

Figure 6: Comparison of the runtimes for a given value of tolerance (left panel) and the l2 norm of the global error incurred (right panel) for Leja (blue circles), LeKry (green pluses), and KIOPS (red diamonds) with the EPIRK4s3 integrator for the Gray-Scott equation ( $\alpha = 0.01$ ).

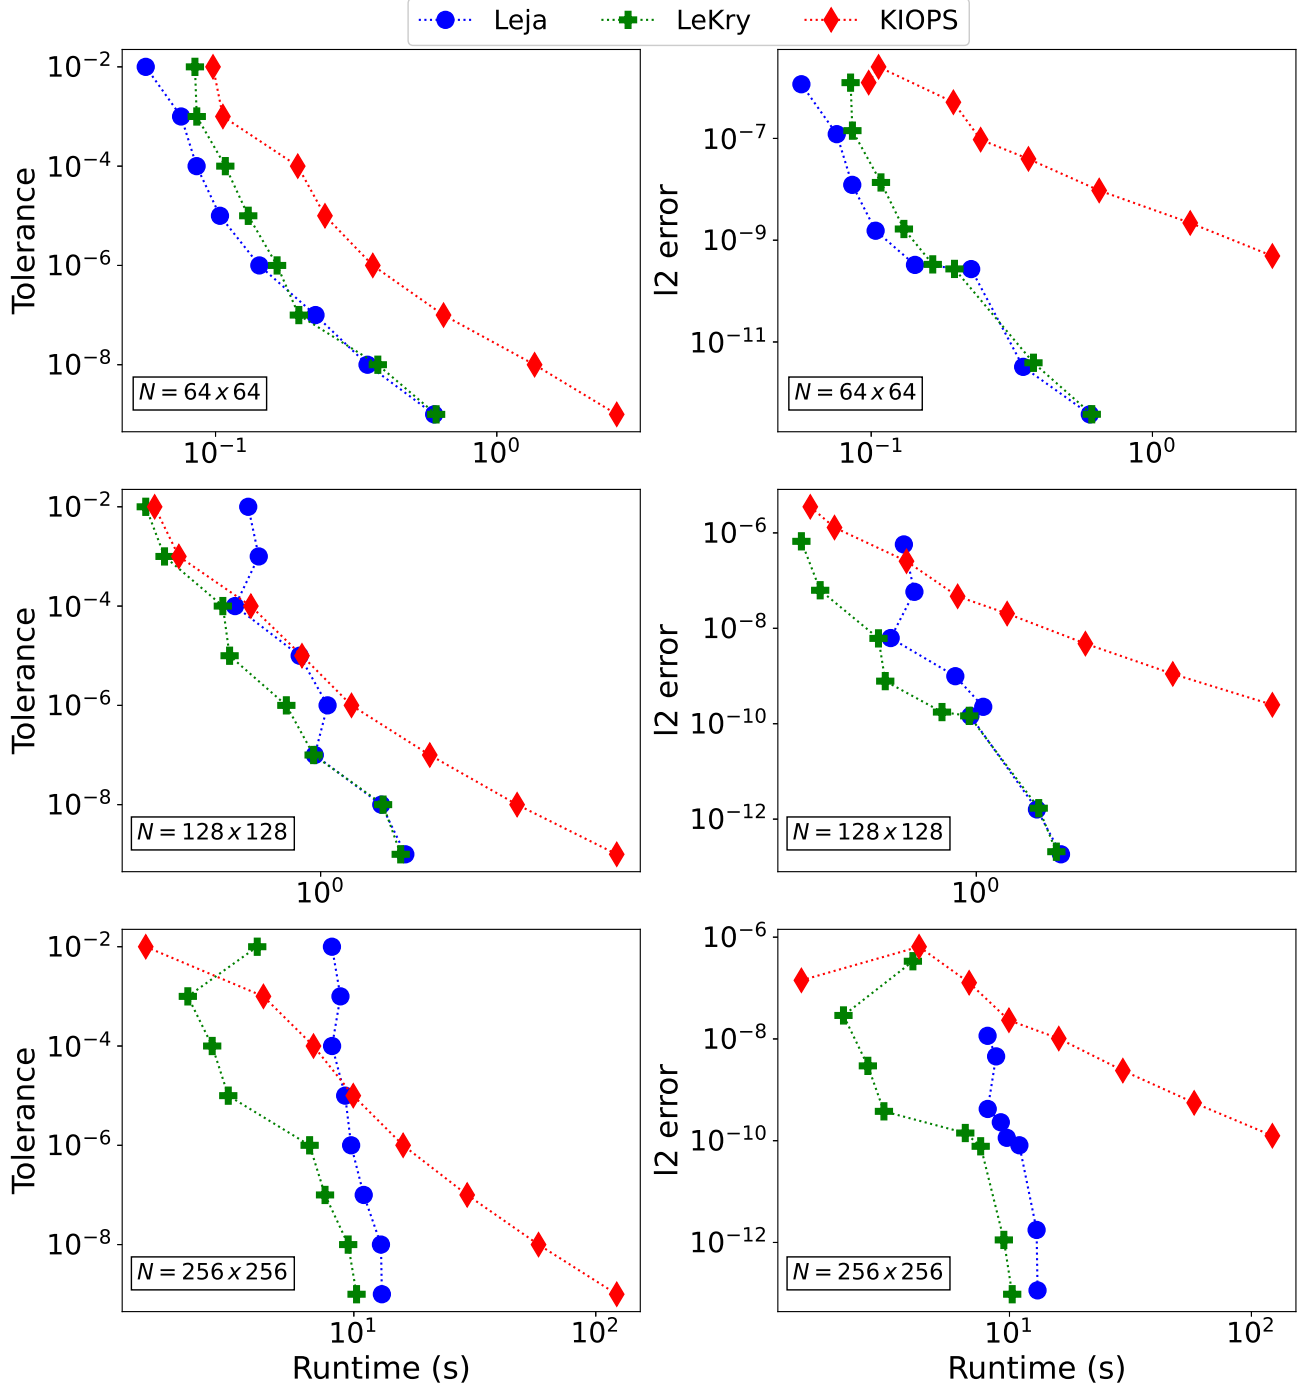

Figure 7: Comparison of the runtimes for a given value of tolerance (left panel) and the  $l_2$  norm of the global error incurred (right panel) for Leja (blue circles), LeKry (green pluses), and KIOPS (red diamonds) with the EPIRK4s3 integrator for the Gray-Scott equation ( $\alpha = 0.1$ ).



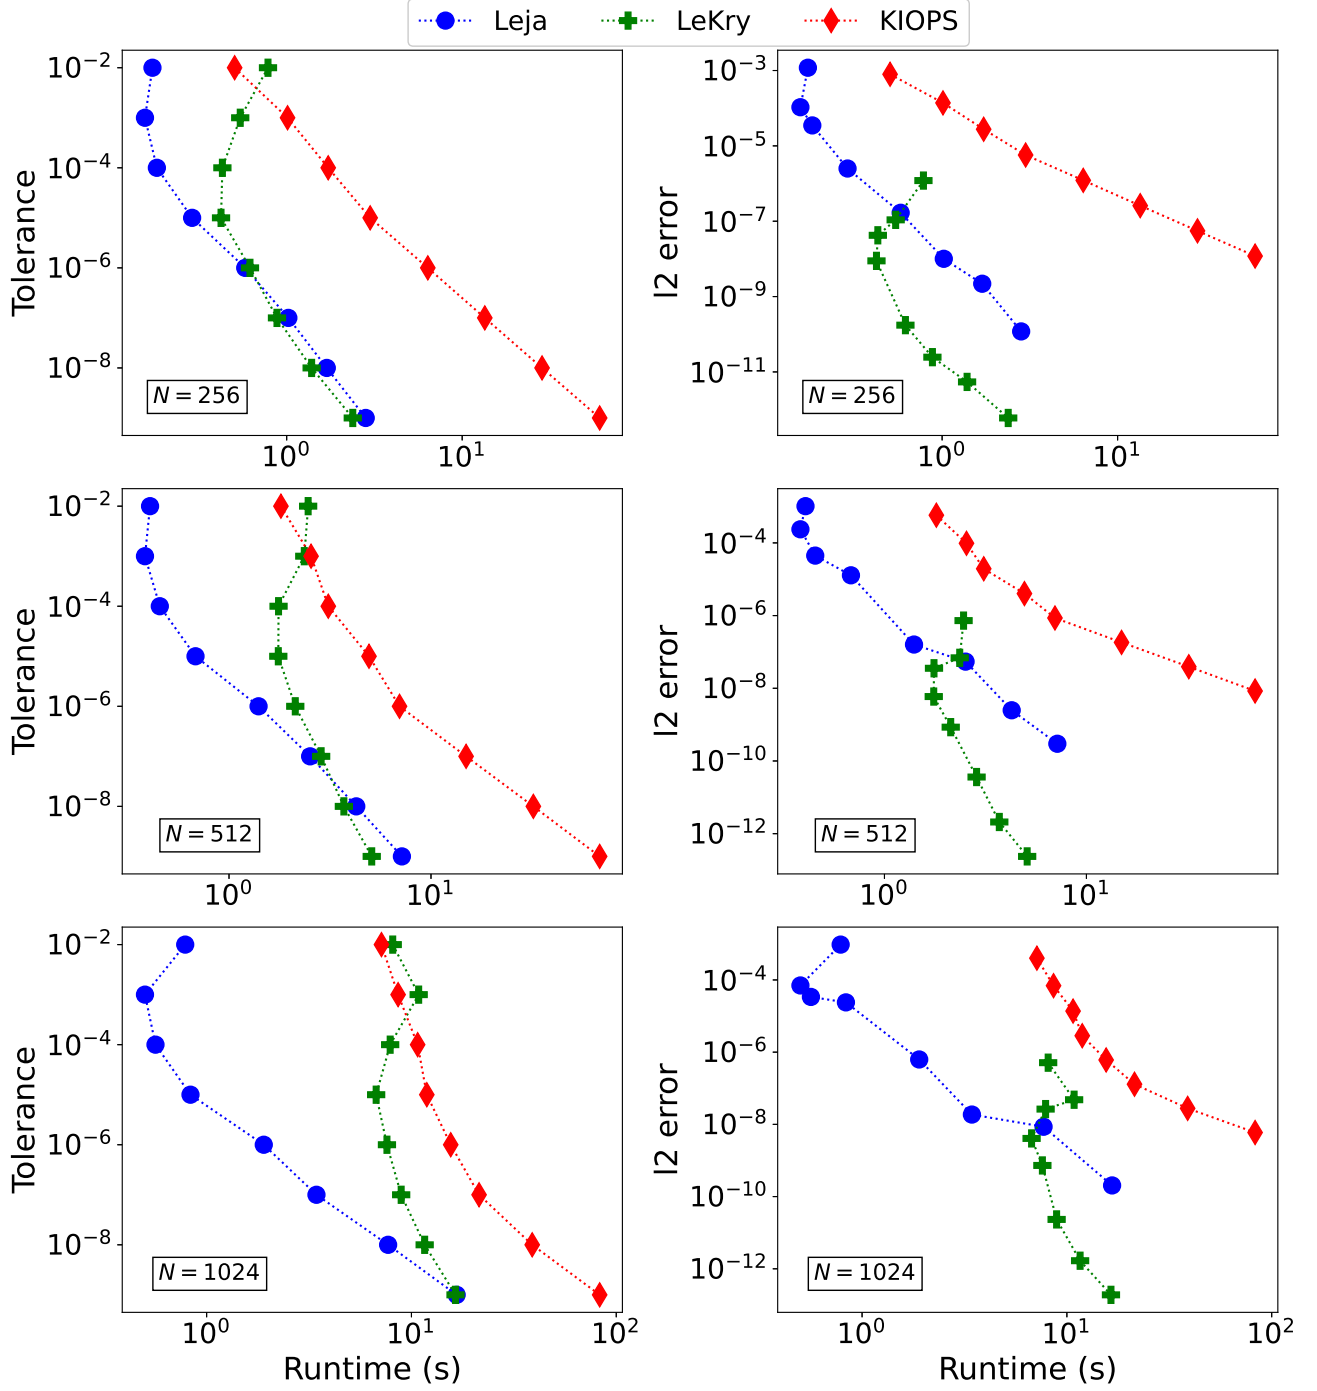

Figure 8: Comparison of the runtimes for a given value of tolerance (left panel) and the  $l_2$  norm of the global error incurred (right panel) for Leja (blue circles), LeKry (green pluses), and KIOPS (red diamonds) with the EPIRK4s3 integrator for the semilinear equation.

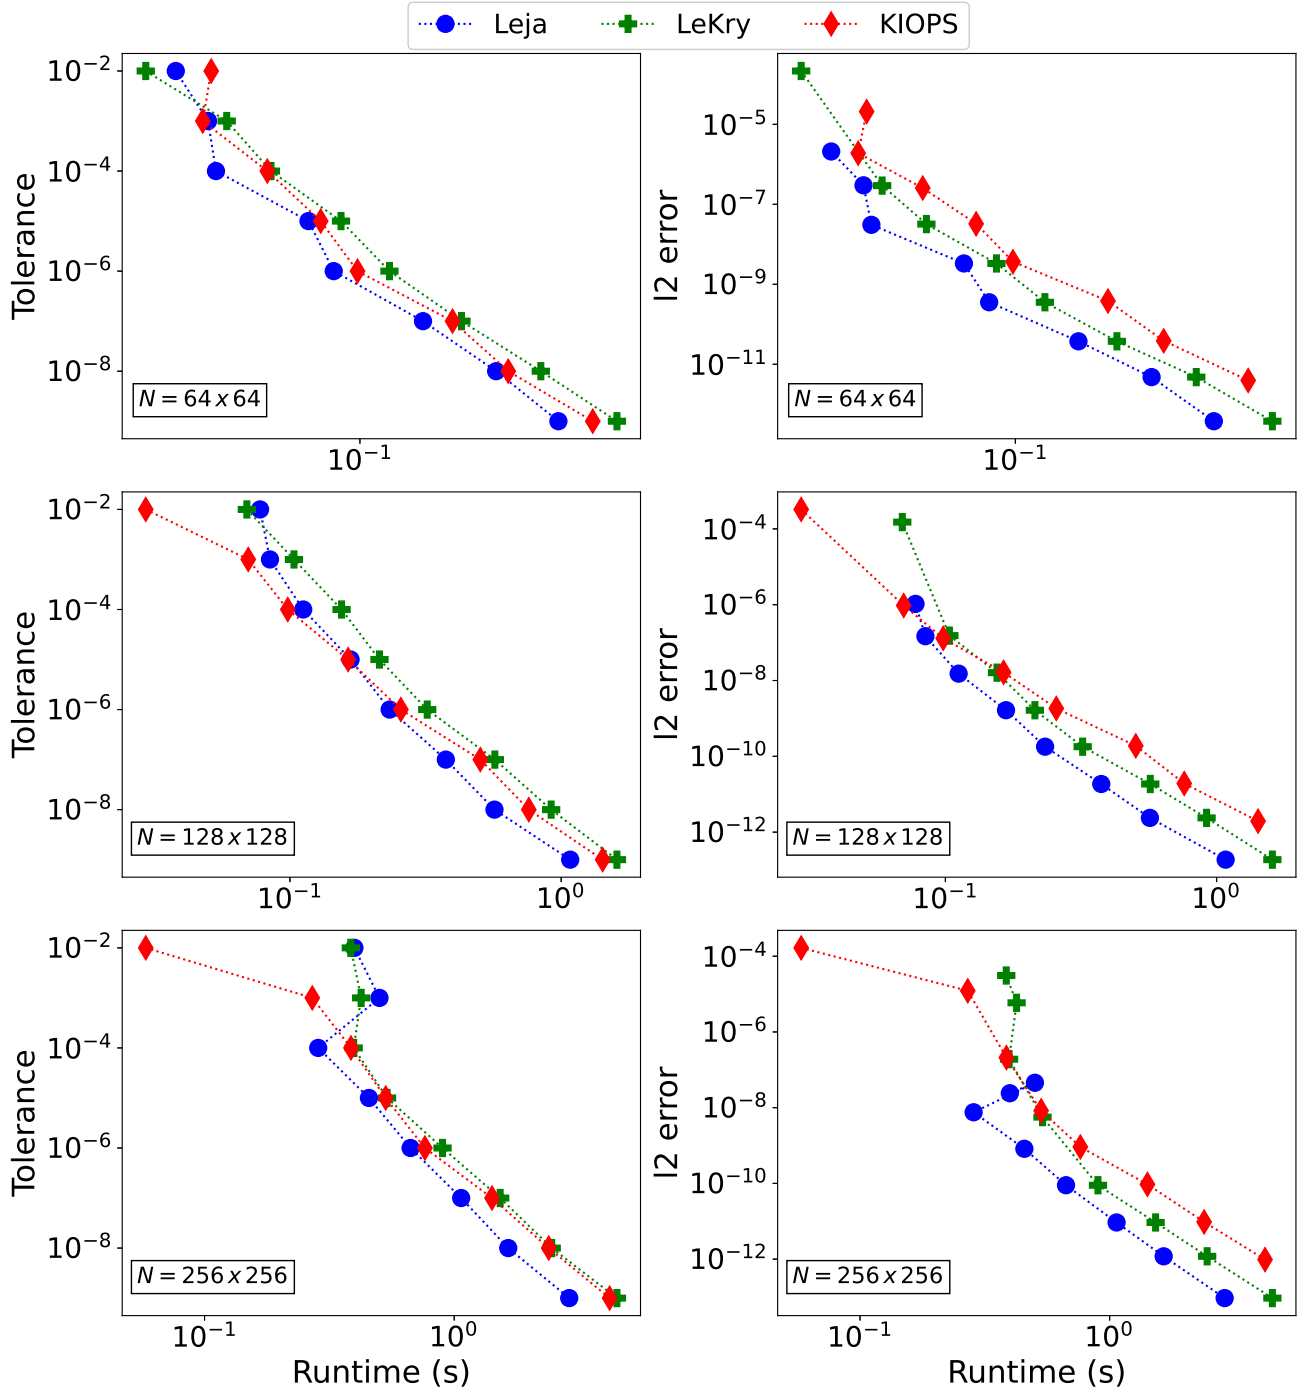

Figure 9: Comparison of the runtimes for a given value of tolerance (left panel) and the l2 norm of the global error incurred (right panel) for Leja (blue circles), LeKry (green pluses), and KIOPS (red diamonds) with the EPIRK4s3A integrator for the ADR equation ( $\alpha = 0.01$ ).

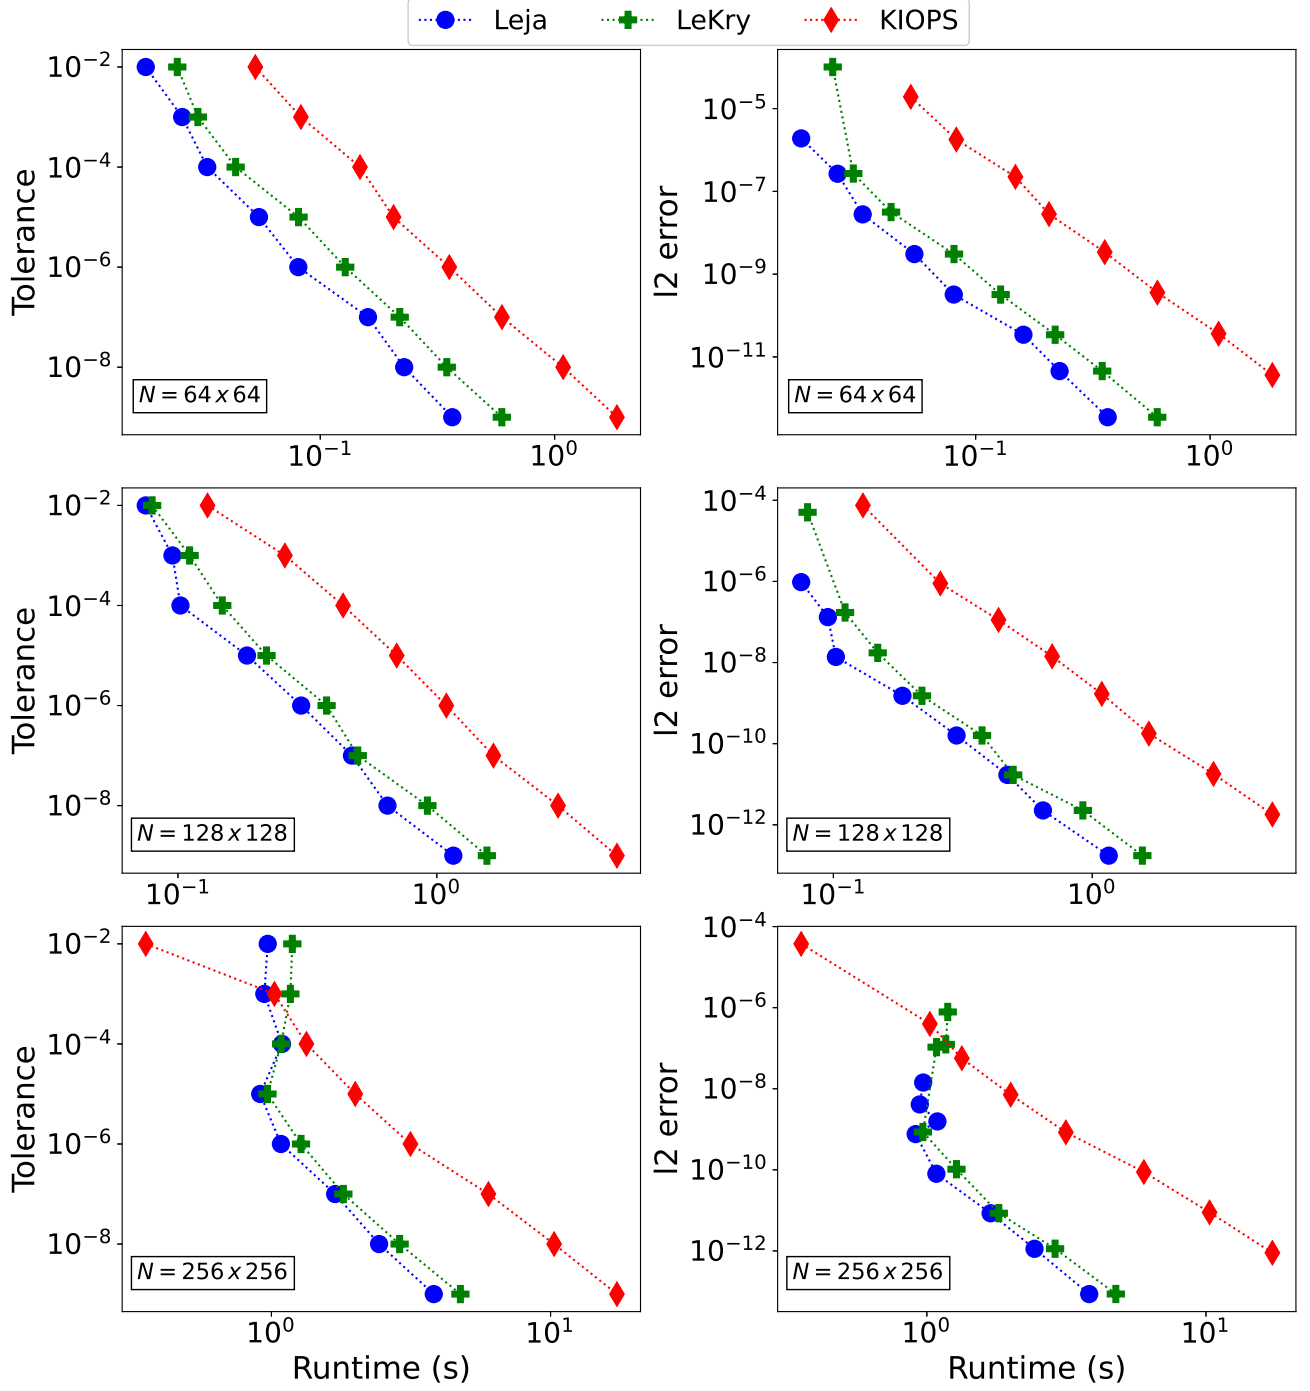

Figure 10: Comparison of the runtimes for a given value of tolerance (left panel) and the l2 norm of the global error incurred (right panel) for Leja (blue circles), LeKry (green pluses), and KIOPS (red diamonds) with the EPIRK4s3A integrator for the ADR equation ( $\alpha = 0.1$ ).

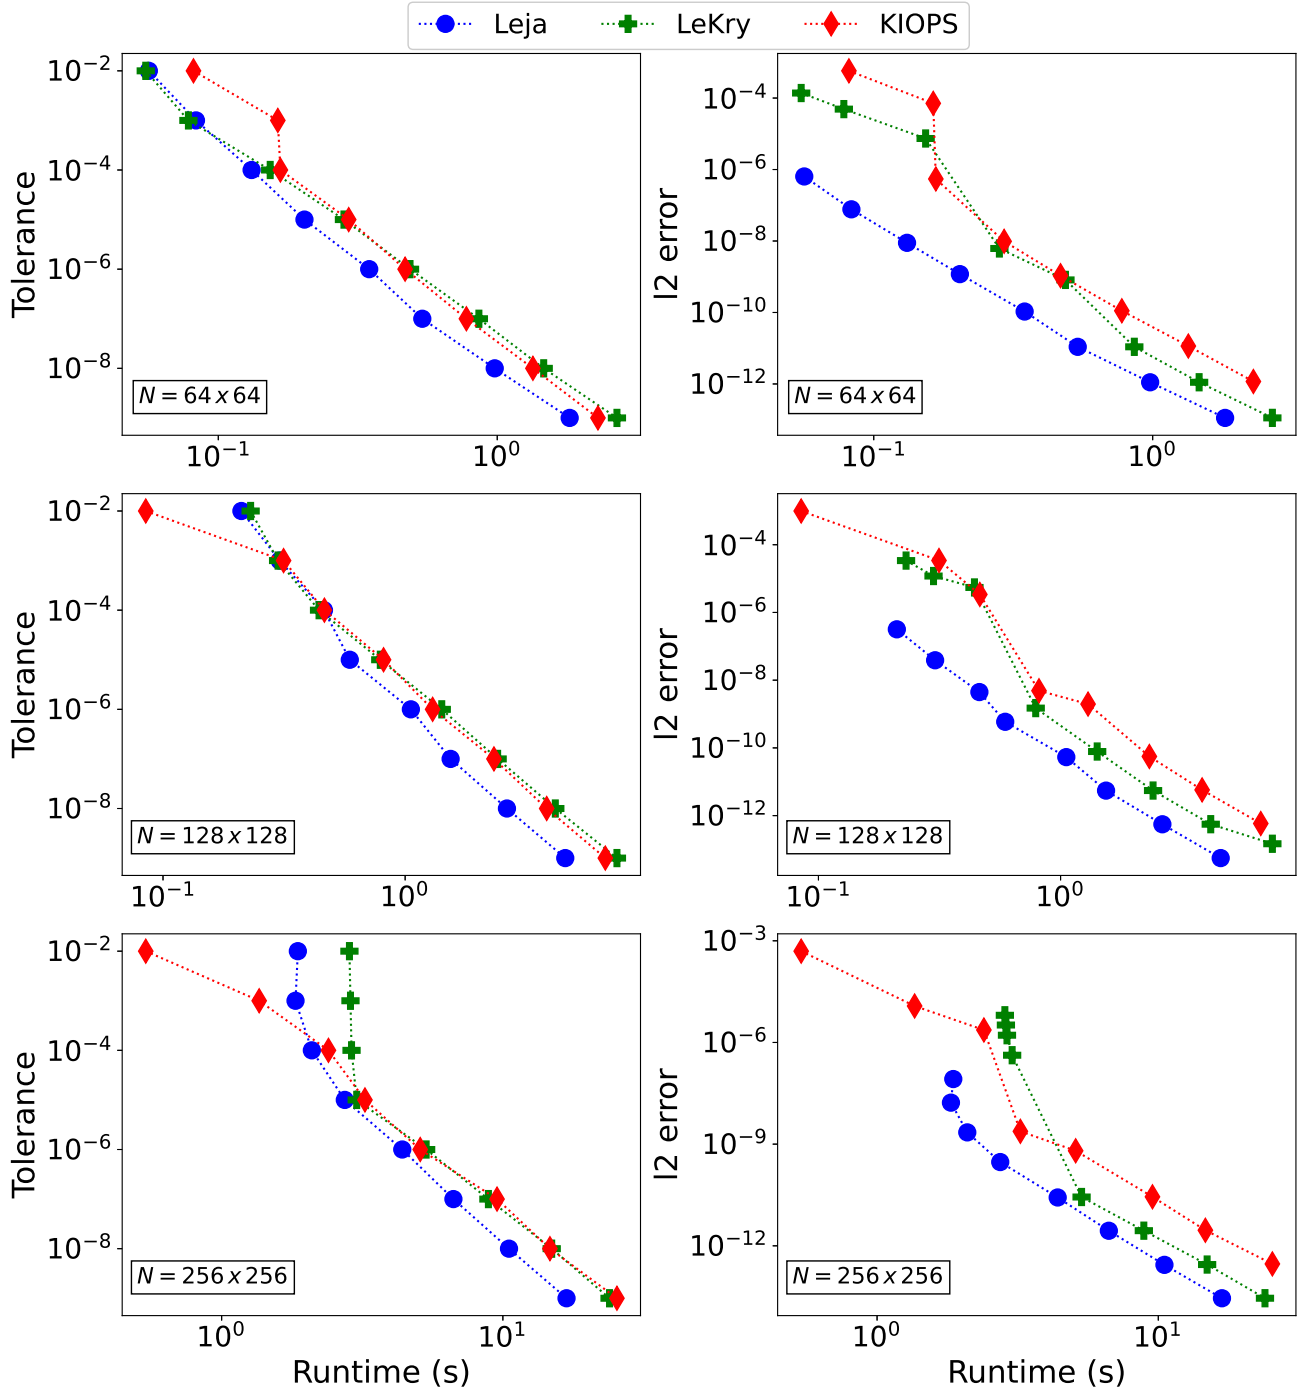

Figure 11: Comparison of the runtimes for a given value of tolerance (left panel) and the l2 norm of the global error incurred (right panel) for Leja (blue circles), LeKry (green pluses), and KIOPS (red diamonds) with the EPIRK4s3A integrator for the Brusselator equation ( $\alpha = 0.001$ ).

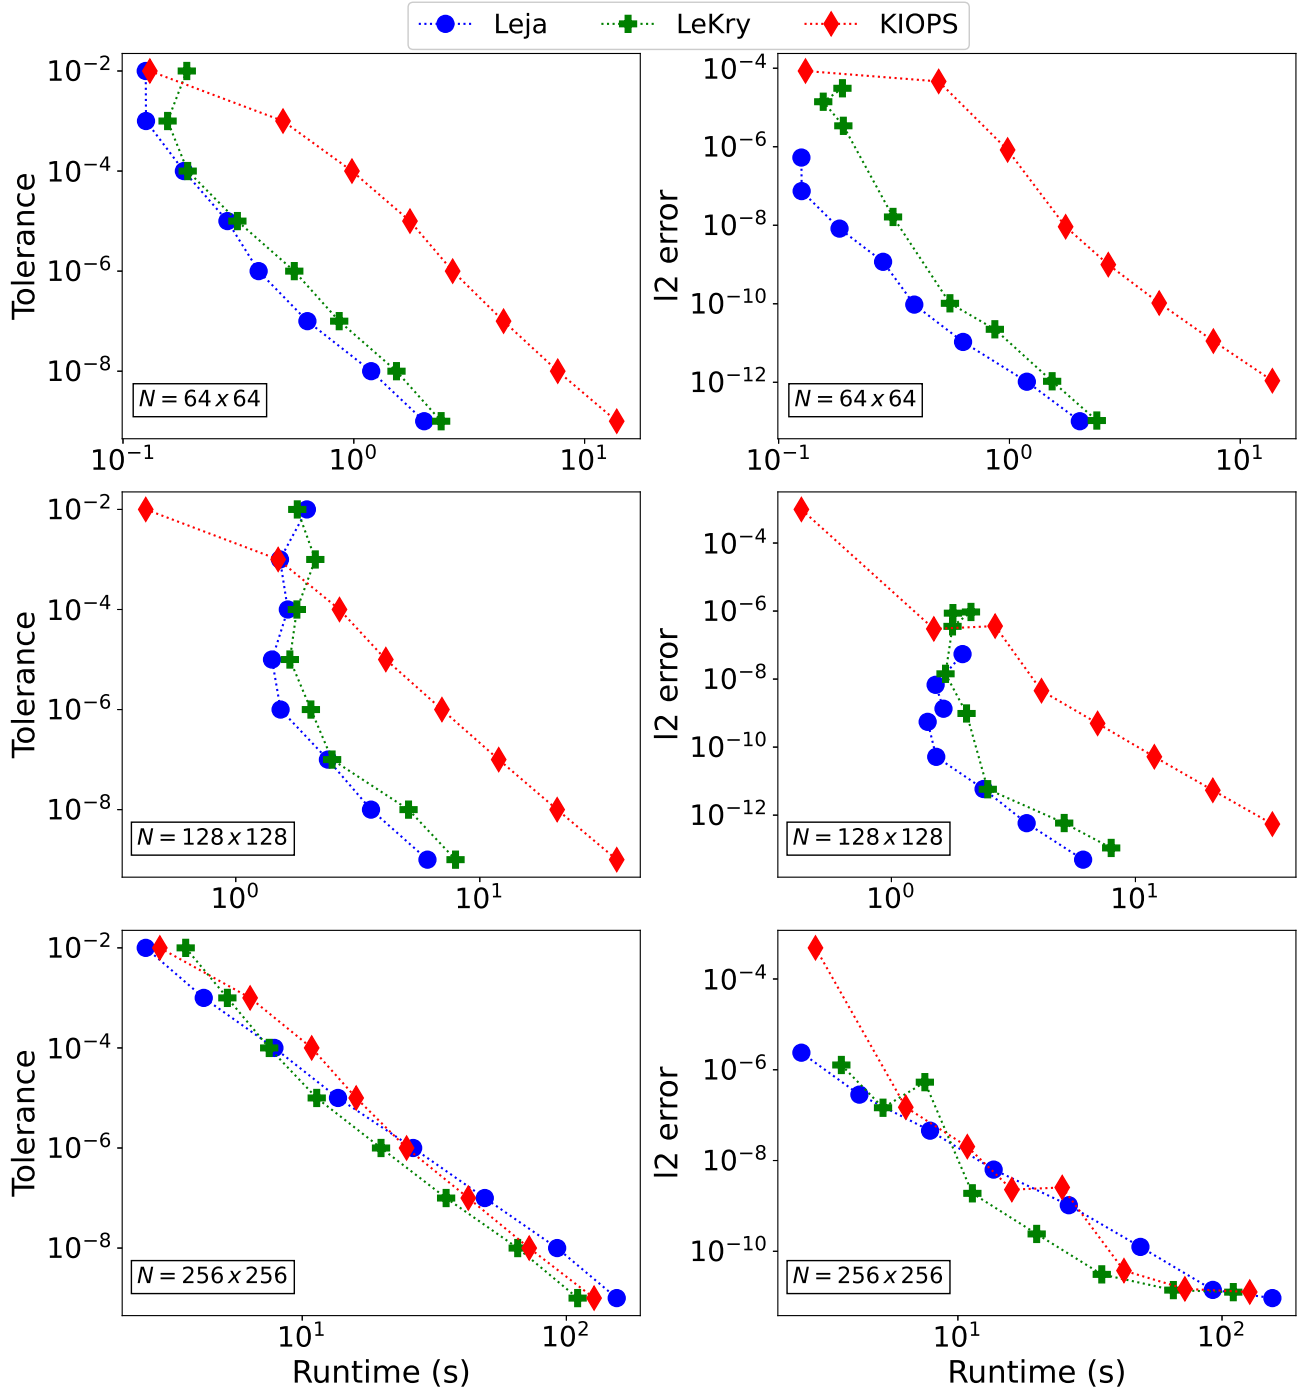

Figure 12: Comparison of the runtimes for a given value of tolerance (left panel) and the l2 norm of the global error incurred (right panel) for Leja (blue circles), LeKry (green pluses), and KIOPS (red diamonds) with the EPIRK4s3A integrator for the Brusselator equation ( $\alpha = 0.01$ ).

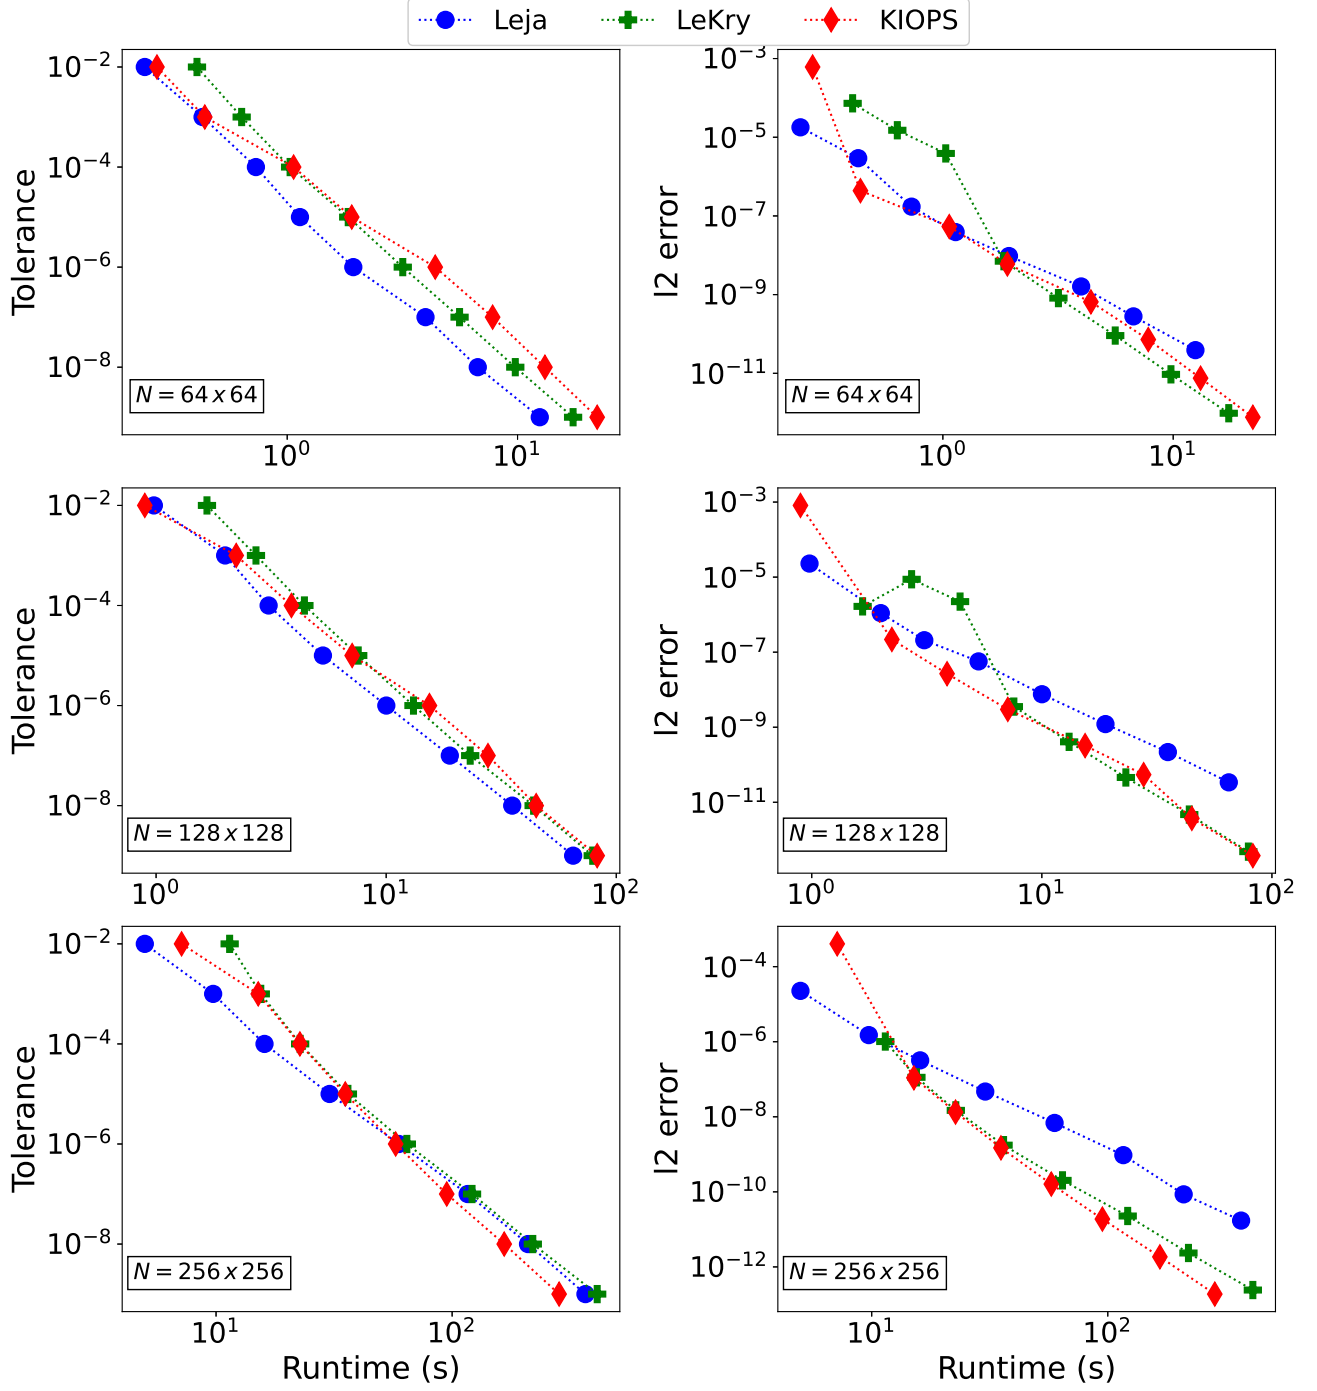

Figure 13: Comparison of the runtimes for a given value of tolerance (left panel) and the l2 norm of the global error incurred (right panel) for Leja (blue circles), LeKry (green pluses), and KIOPS (red diamonds) with the EPIRK4s3A integrator for the Brusselator equation ( $\alpha = 0.1$ ).

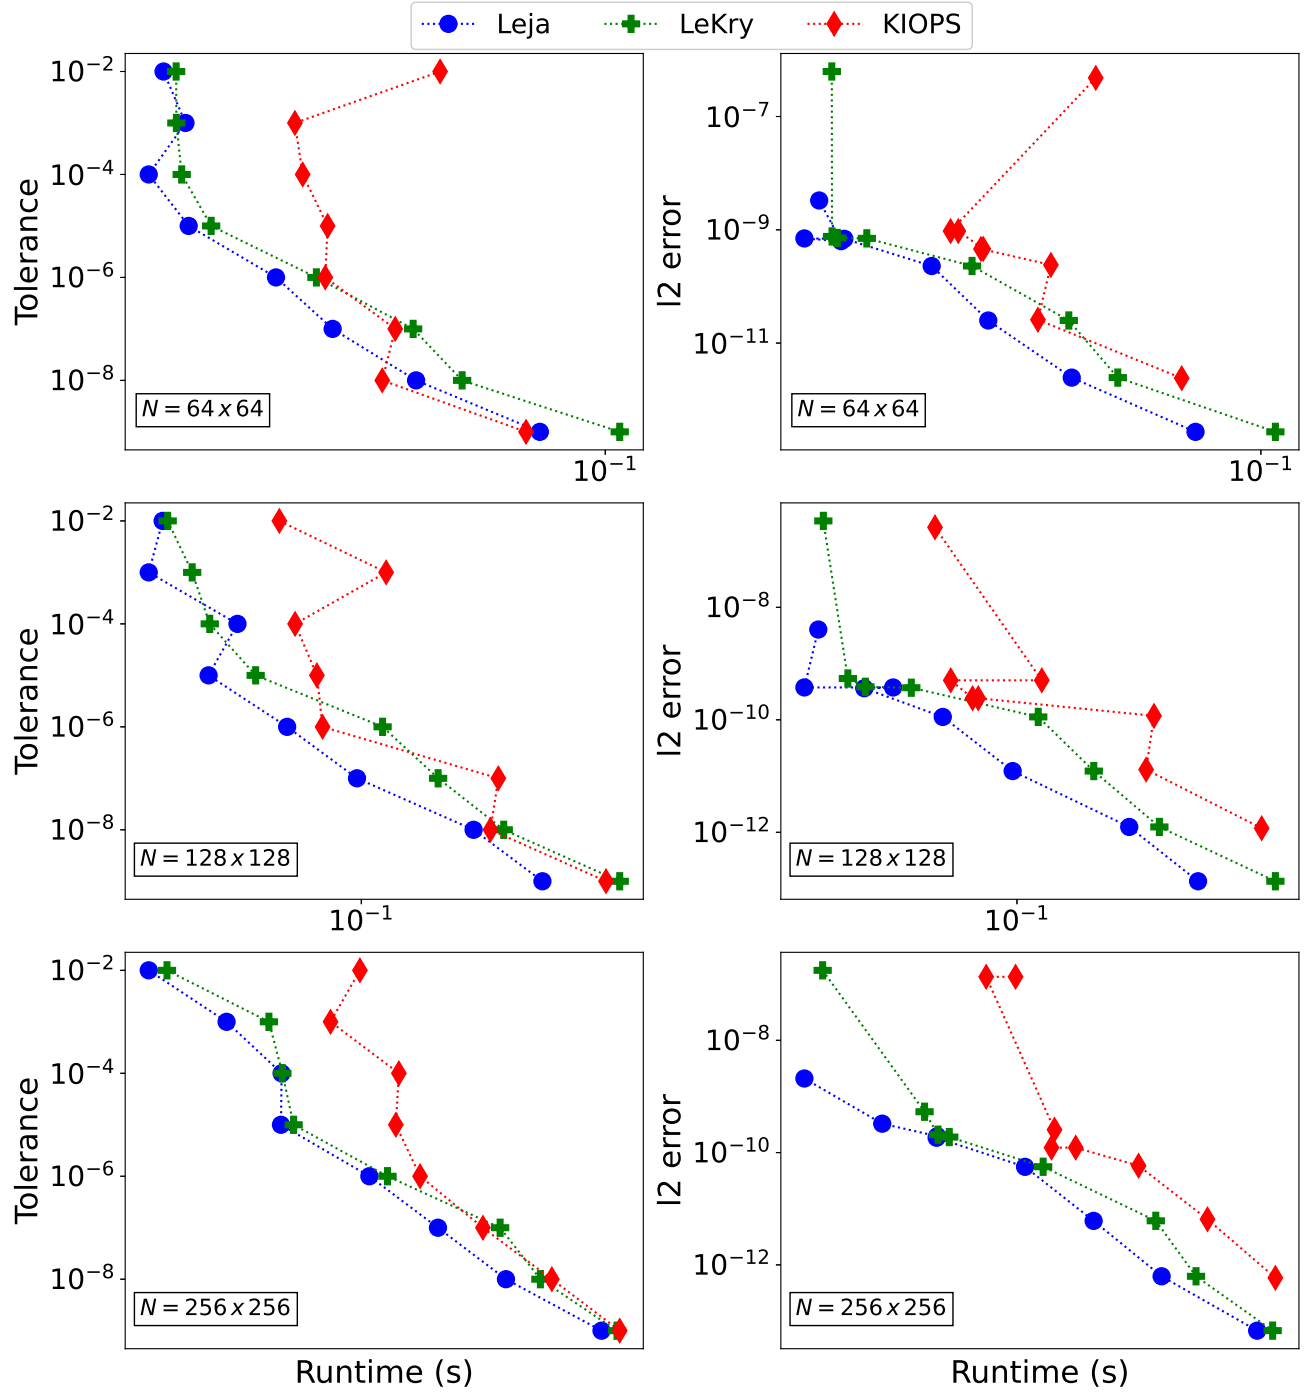

Figure 14: Comparison of the runtimes for a given value of tolerance (left panel) and the l2 norm of the global error incurred (right panel) for Leja (blue circles), LeKry (green pluses), and KIOPS (red diamonds) with the EPIRK4s3A integrator for the Gray-Scott equation ( $\alpha = 0.001$ ).

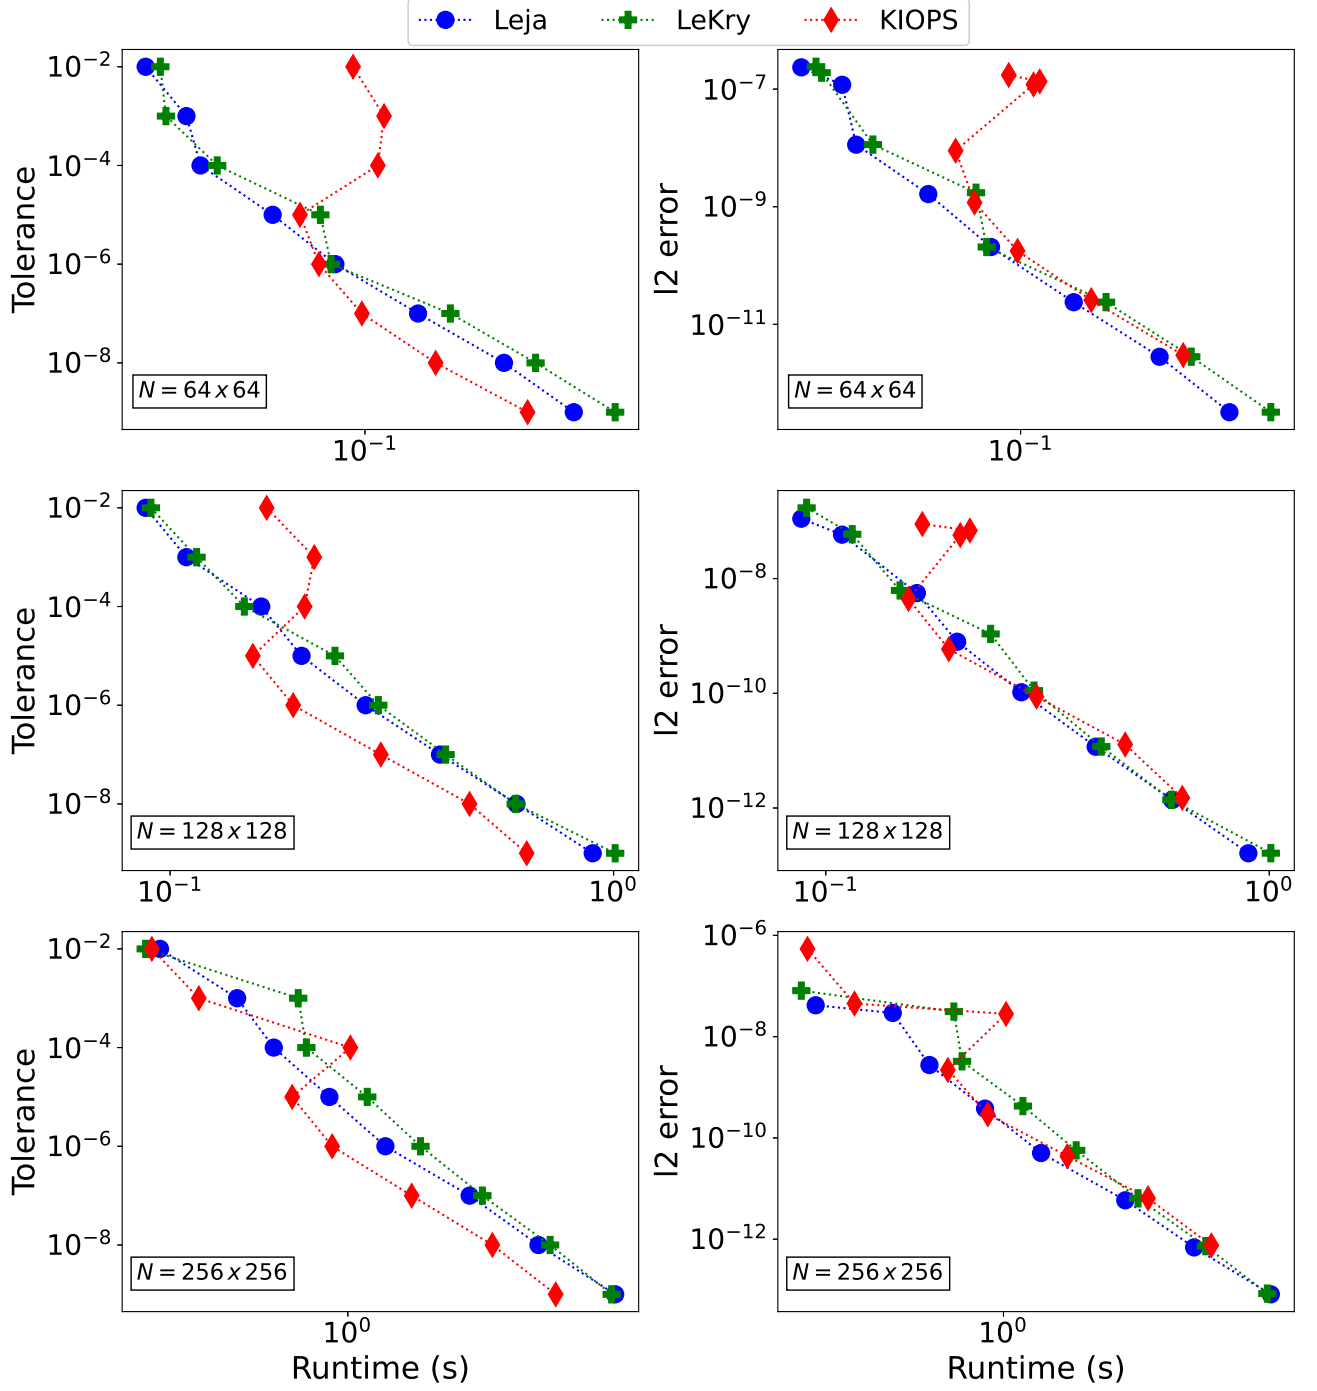

Figure 15: Comparison of the runtimes for a given value of tolerance (left panel) and the l2 norm of the global error incurred (right panel) for Leja (blue circles), LeKry (green pluses), and KIOPS (red diamonds) with the EPIRK4s3A integrator for the Gray-Scott equation ( $\alpha = 0.01$ ).



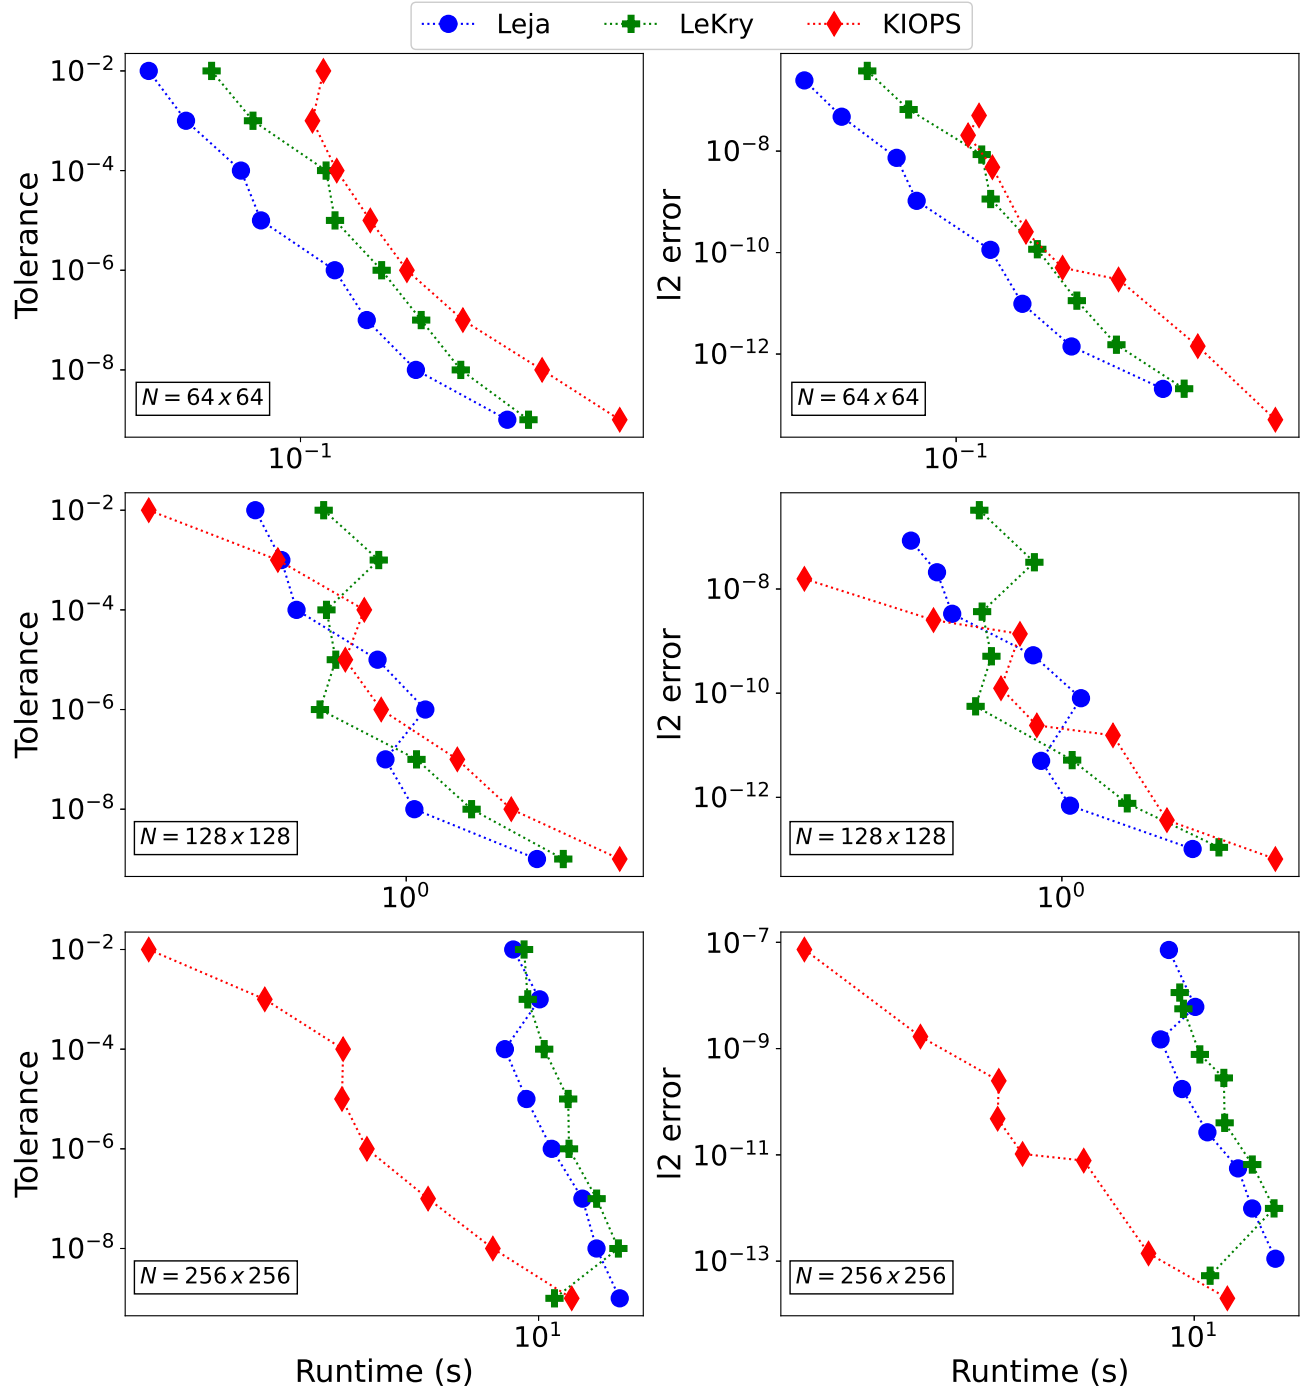

Figure 16: Comparison of the runtimes for a given value of tolerance (left panel) and the l2 norm of the global error incurred (right panel) for Leja (blue circles), LeKry (green pluses), and KIOPS (red diamonds) with the EPIRK4s3A integrator for the Gray-Scott equation ( $\alpha = 0.01$ ).

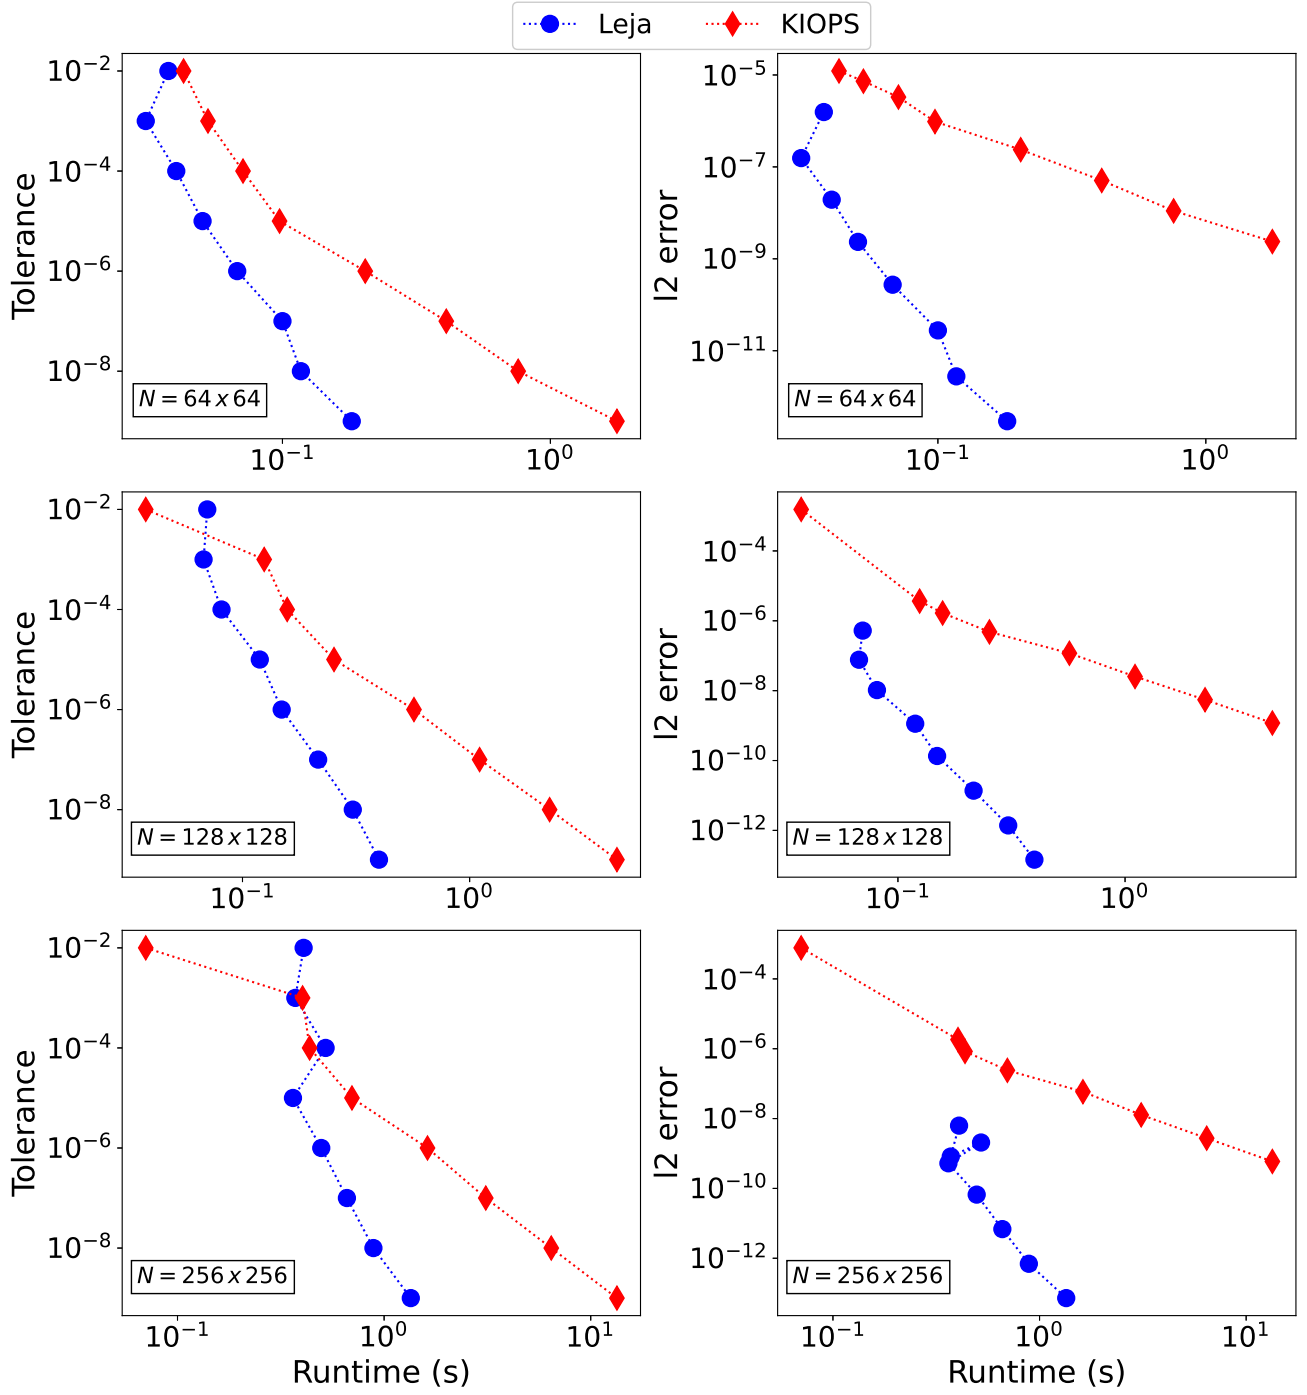

Figure 17: Comparison of the runtimes for a given value of tolerance (left panel) and the l2 norm of the global error incurred (right panel) for Leja (blue circles), LeKry (green pluses), and KIOPS (red diamonds) with the EPIRK5P1 integrator for the ADR equation ( $\alpha = 0.01$ ).

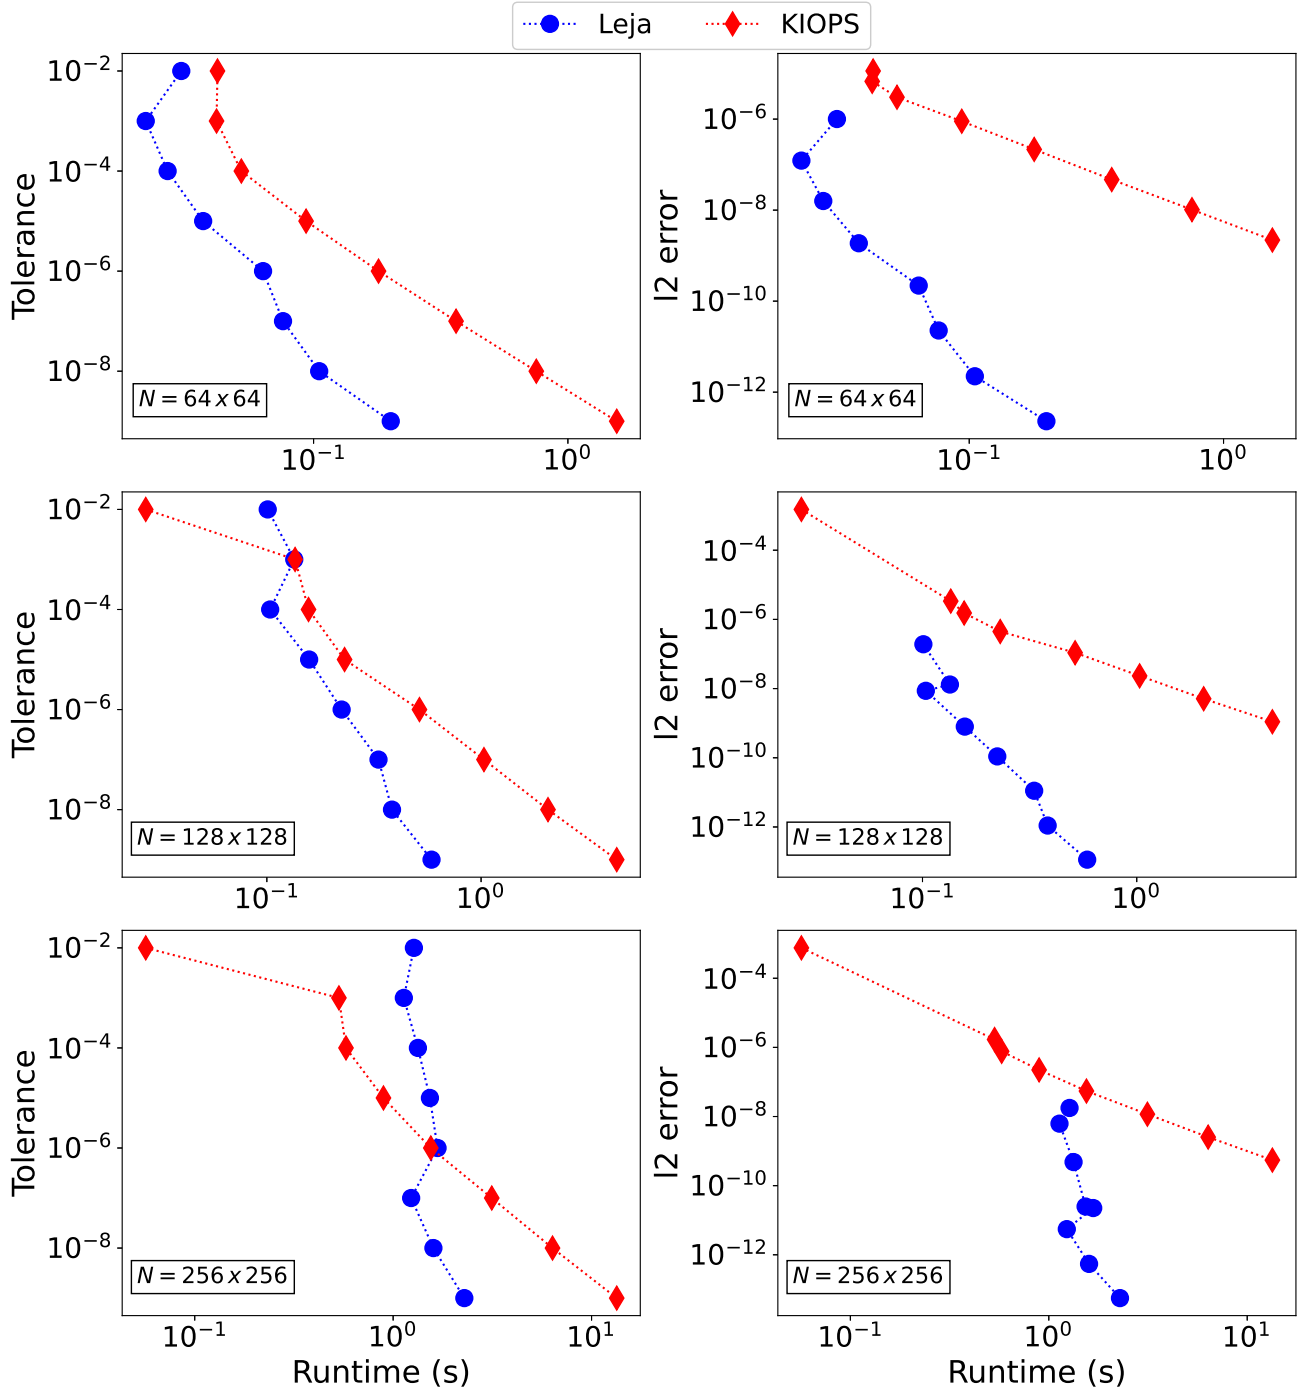

Figure 18: Comparison of the runtimes for a given value of tolerance (left panel) and the l2 norm of the global error incurred (right panel) for Leja (blue circles), LeKry (green pluses), and KIOPS (red diamonds) with the EPIRK5P1 integrator for the ADR equation ( $\alpha = 0.1$ ).

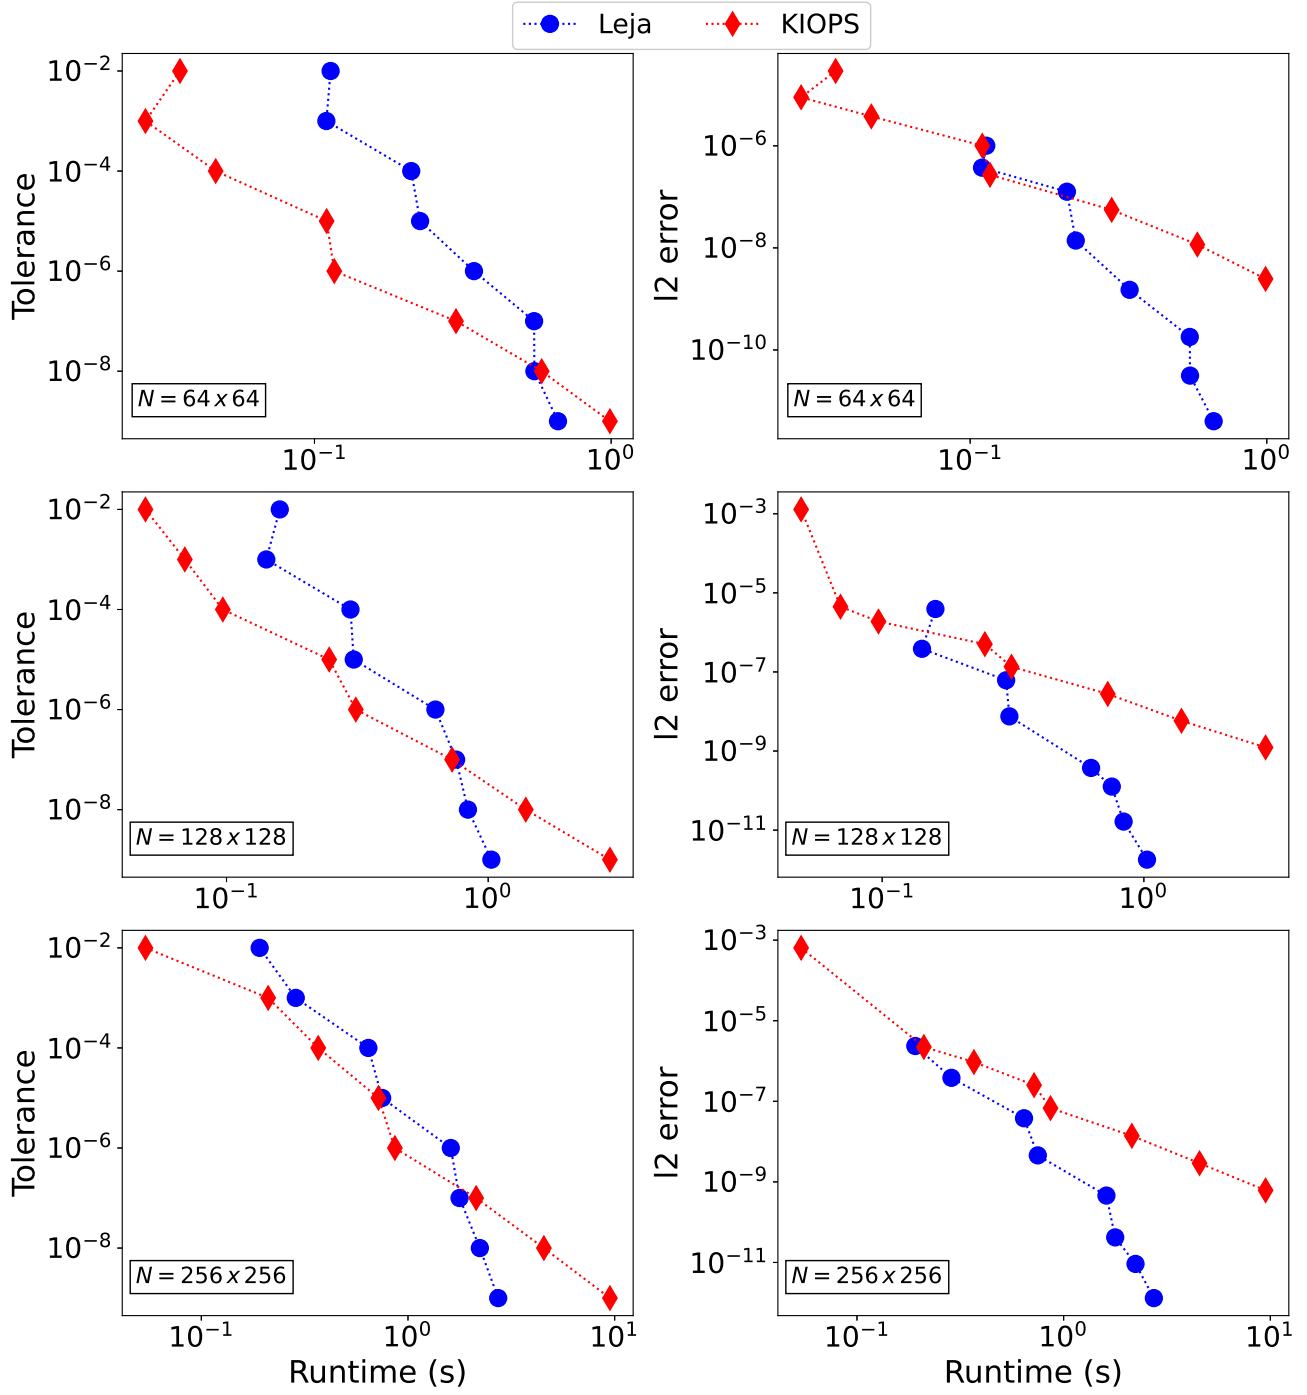

Figure 19: Comparison of the runtimes for a given value of tolerance (left panel) and the  $l_2$  norm of the global error incurred (right panel) for Leja (blue circles), LeKry (green pluses), and KIOPS (red diamonds) with the EPIRK5P1 integrator for the Allen-Cahn equation ( $\alpha = 0.001$ ).

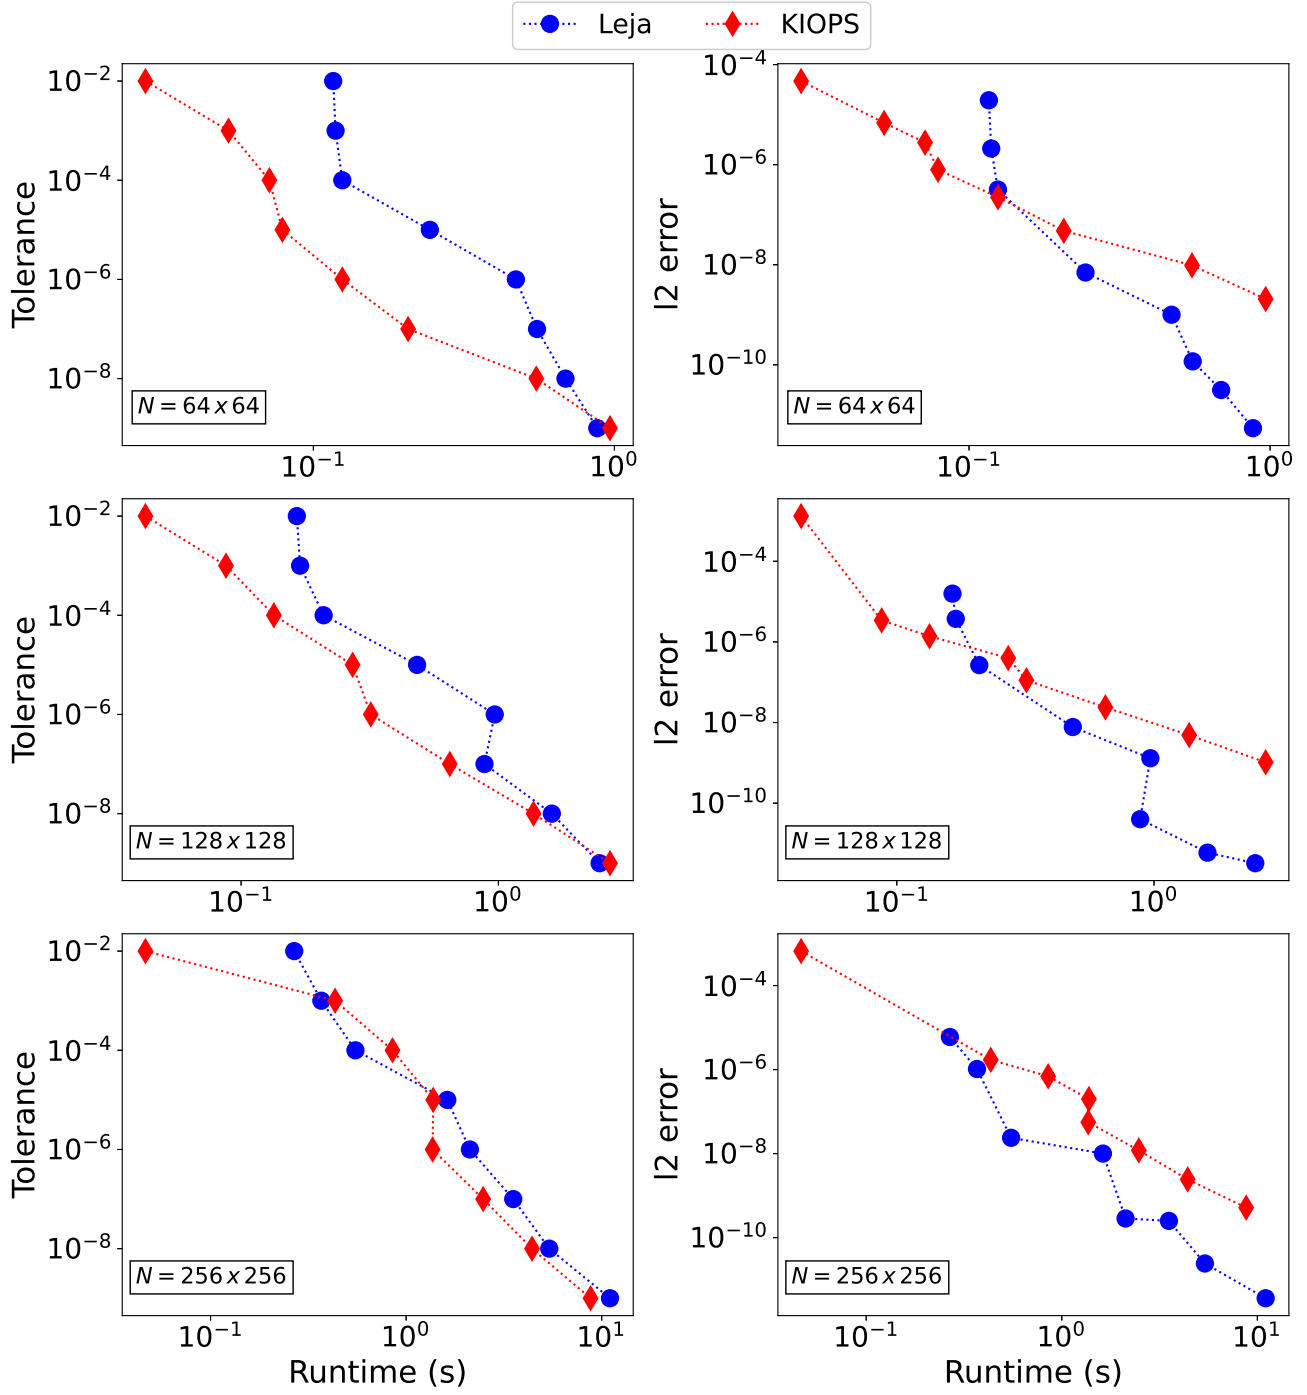

Figure 20: Comparison of the runtimes for a given value of tolerance (left panel) and the  $l_2$  norm of the global error incurred (right panel) for Leja (blue circles), LeKry (green pluses), and KIOPS (red diamonds) with the EPIRK5P1 integrator for the Allen-Cahn equation ( $\alpha = 0.01$ ).

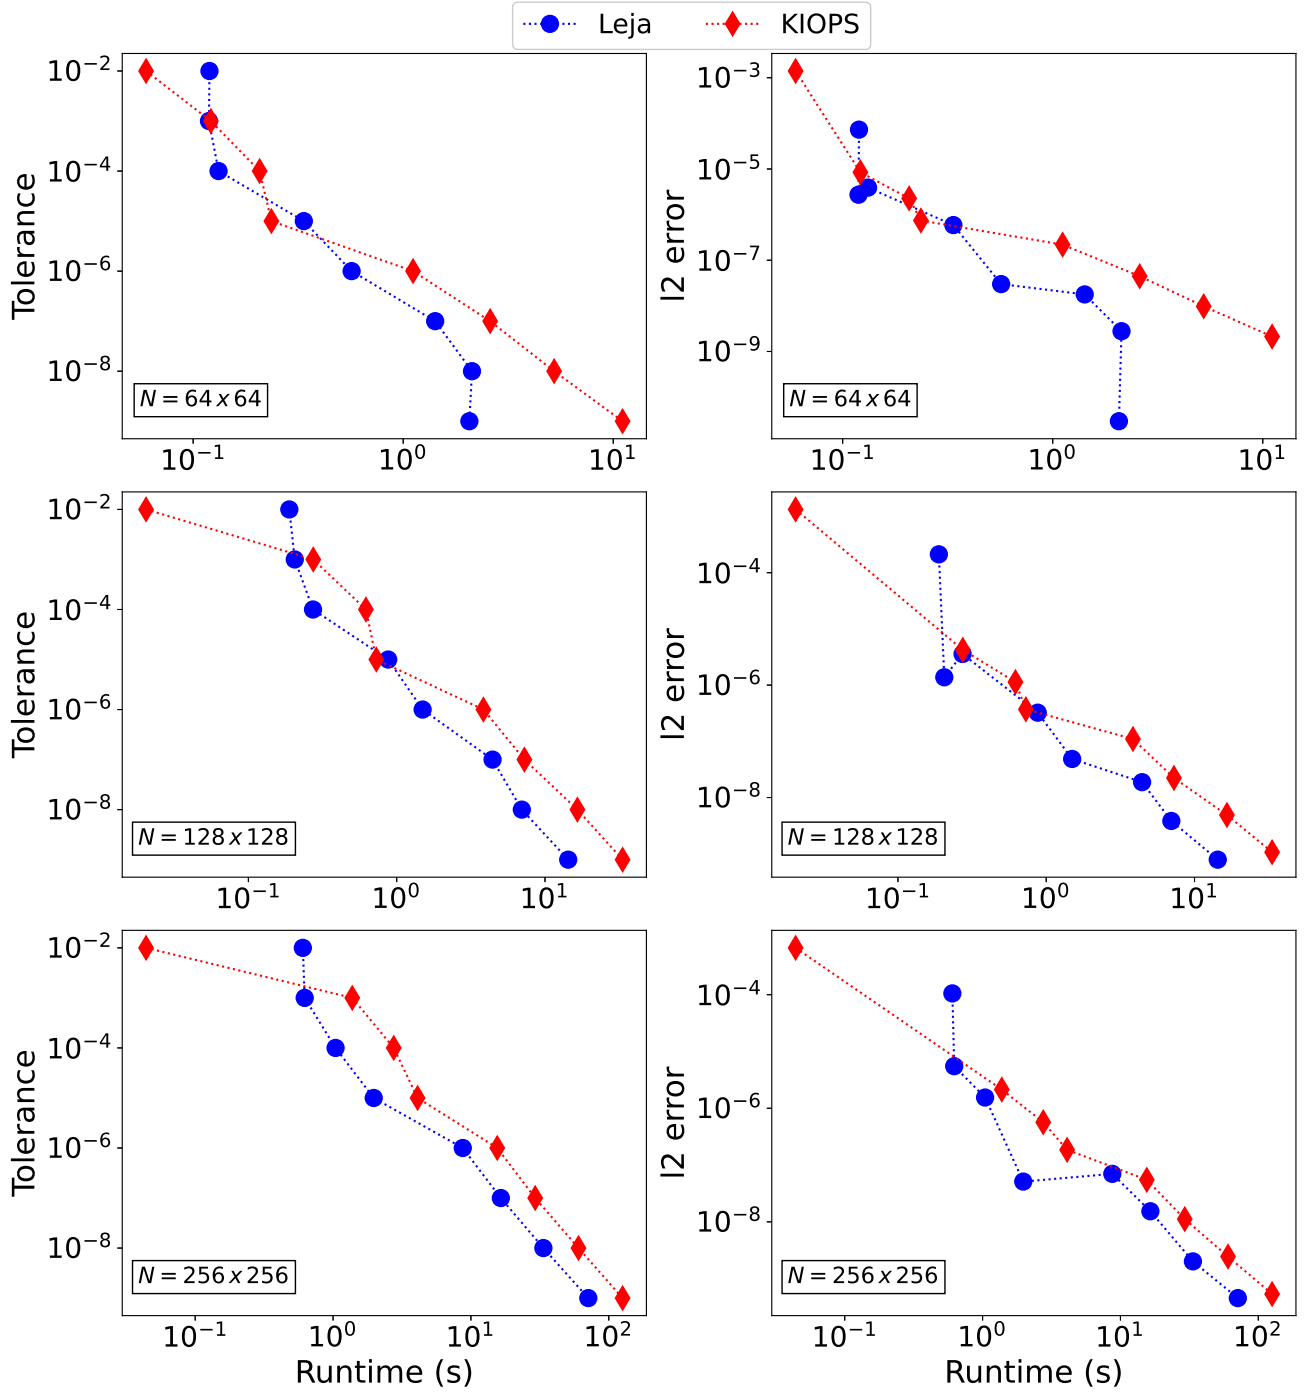

Figure 21: Comparison of the runtimes for a given value of tolerance (left panel) and the l2 norm of the global error incurred (right panel) for Leja (blue circles), LeKry (green pluses), and KIOPS (red diamonds) with the EPIRK5P1 integrator for the Allen-Cahn equation ( $\alpha = 0.1$ ).

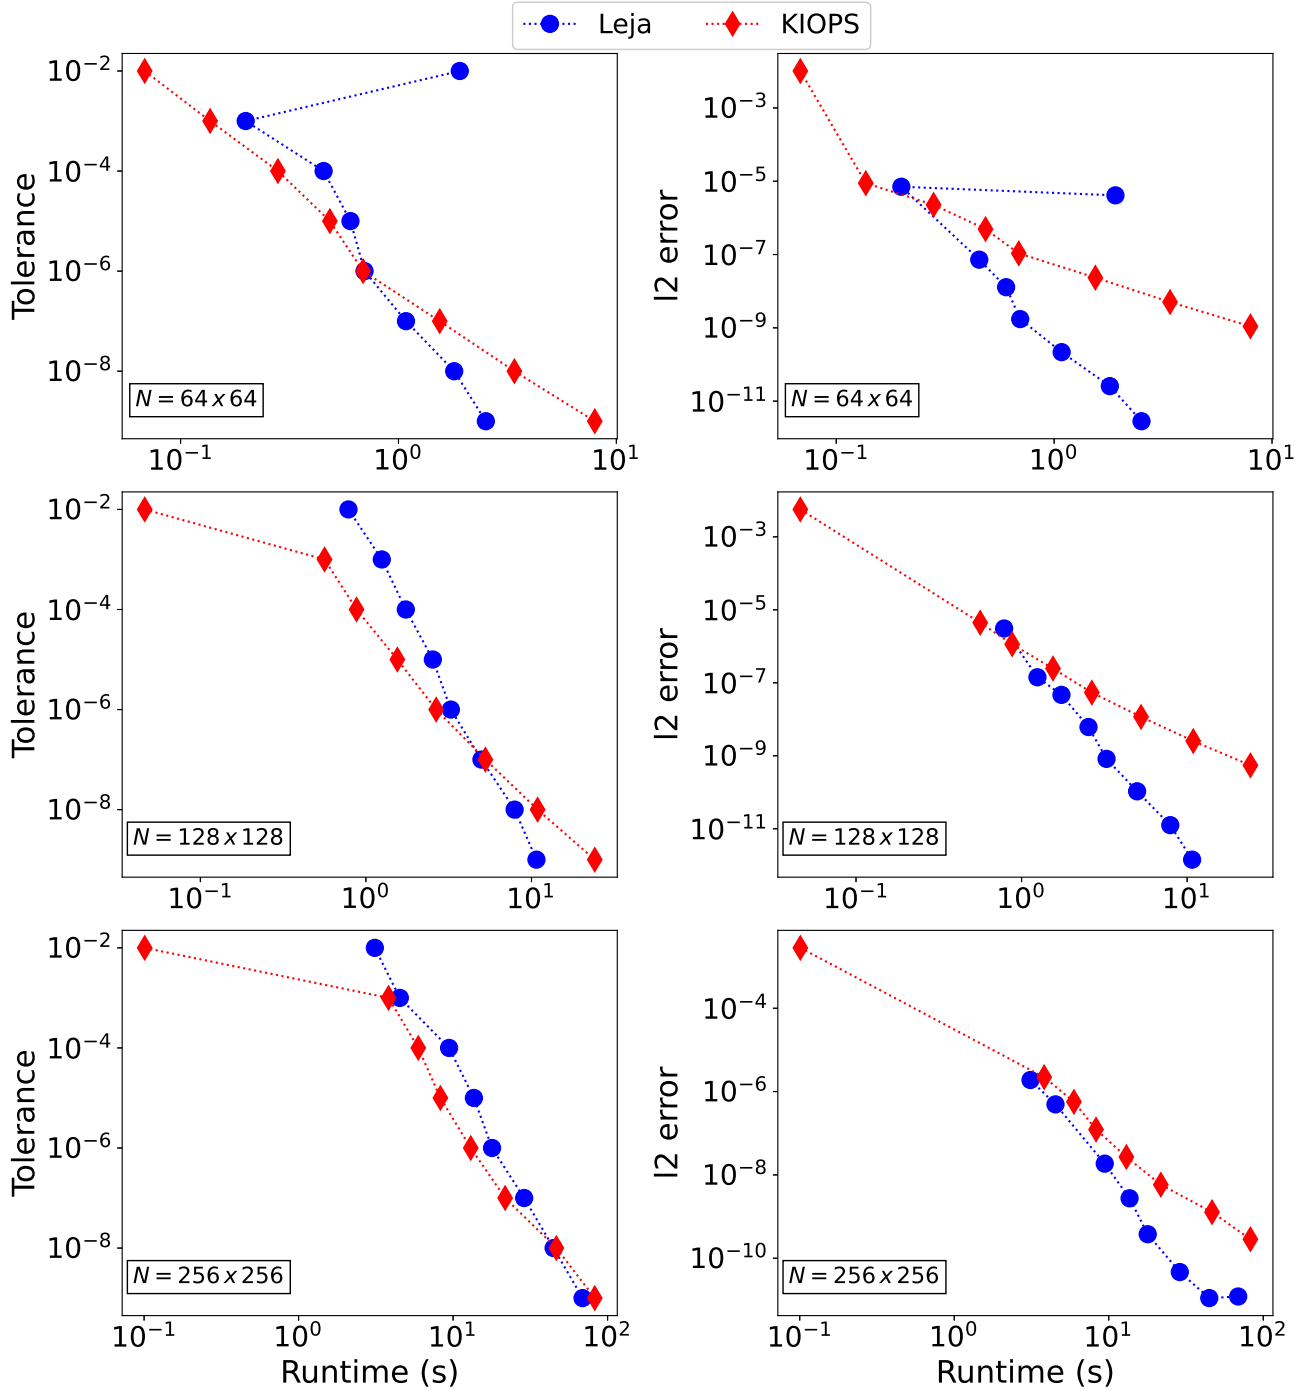

Figure 22: Comparison of the runtimes for a given value of tolerance (left panel) and the l2 norm of the global error incurred (right panel) for Leja (blue circles), LeKry (green pluses), and KIOPS (red diamonds) with the EPIRK5P1 integrator for the Brusselator equation ( $\alpha = 0.01$ ).

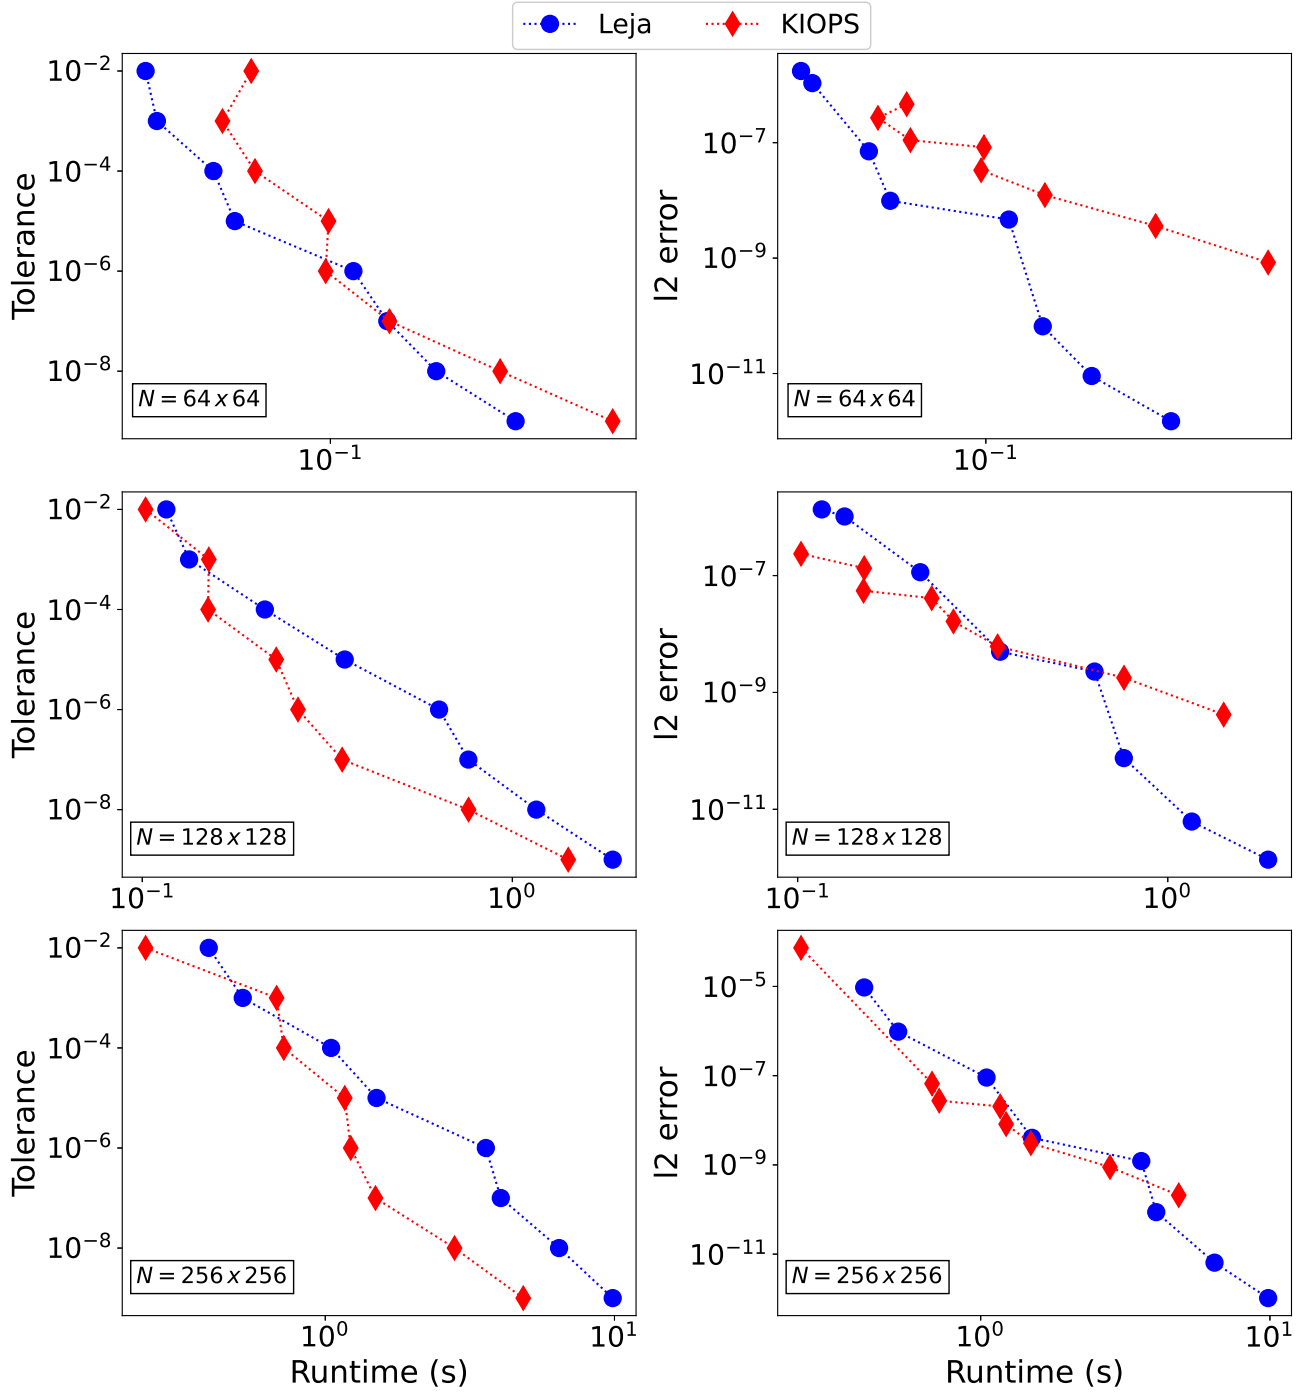

Figure 23: Comparison of the runtimes for a given value of tolerance (left panel) and the  $l_2$  norm of the global error incurred (right panel) for Leja (blue circles), LeKry (green pluses), and KIOPS (red diamonds) with the EPIRK5P1 integrator for the Gray-Scott equation ( $\alpha = 0.01$ ).



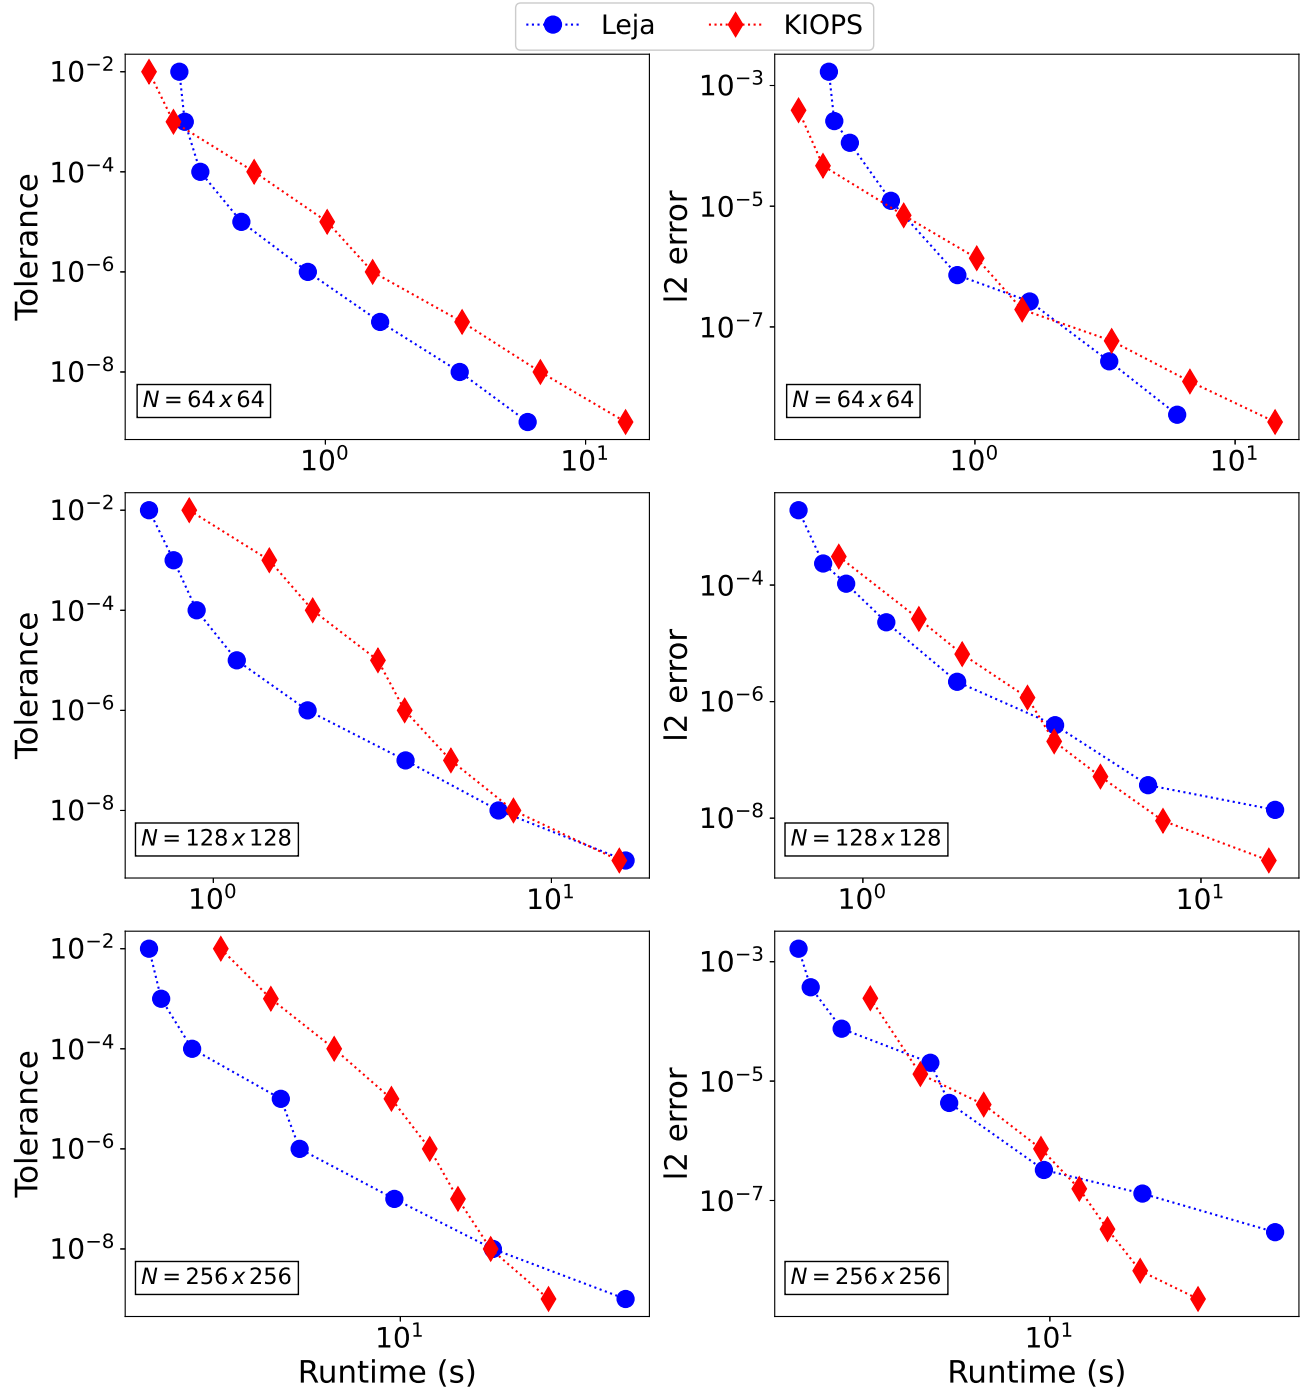

Figure 24: Comparison of the runtimes for a given value of tolerance (left panel) and the l2 norm of the global error incurred (right panel) for Leja (blue circles), LeKry (green pluses), and KIOPS (red diamonds) with the EPIRK5P1 integrator for the semilinear equation.

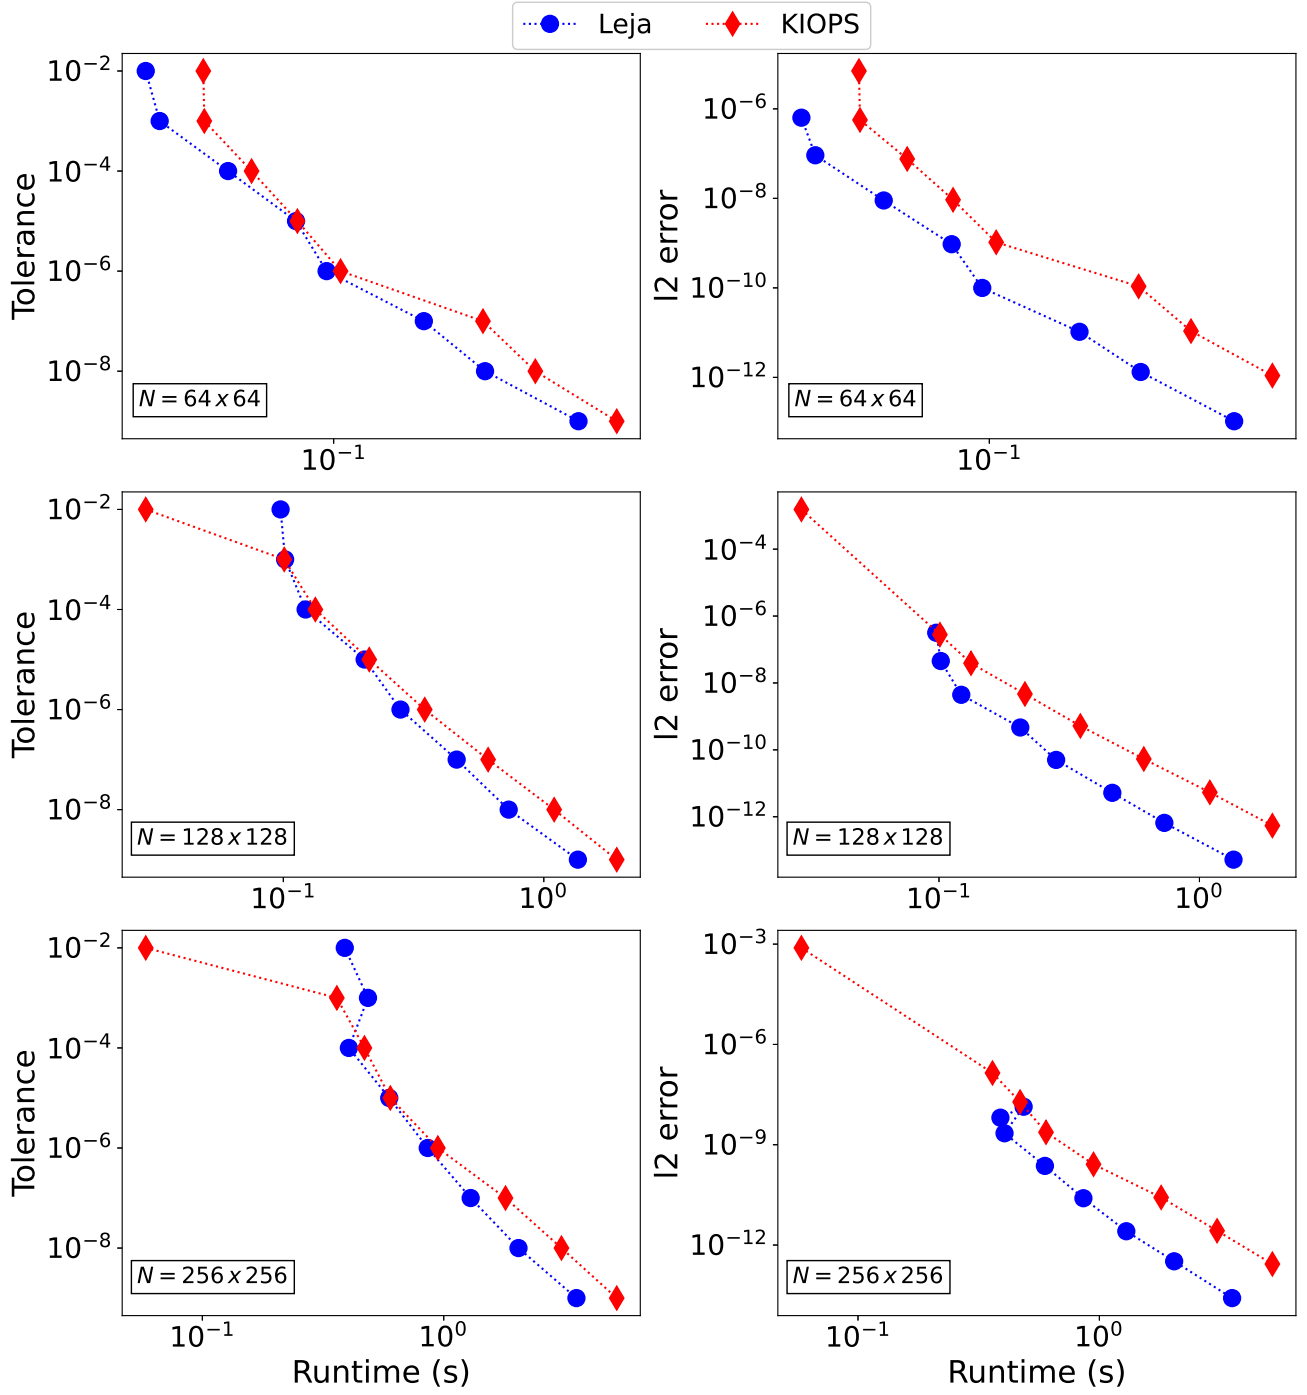

Figure 25: Comparison of the runtimes for a given value of tolerance (left panel) and the l2 norm of the global error incurred (right panel) for Leja (blue circles), LeKry (green pluses), and KIOPS (red diamonds) with the EXPRB43 integrator for the ADR equation ( $\alpha = 0.01$ ).

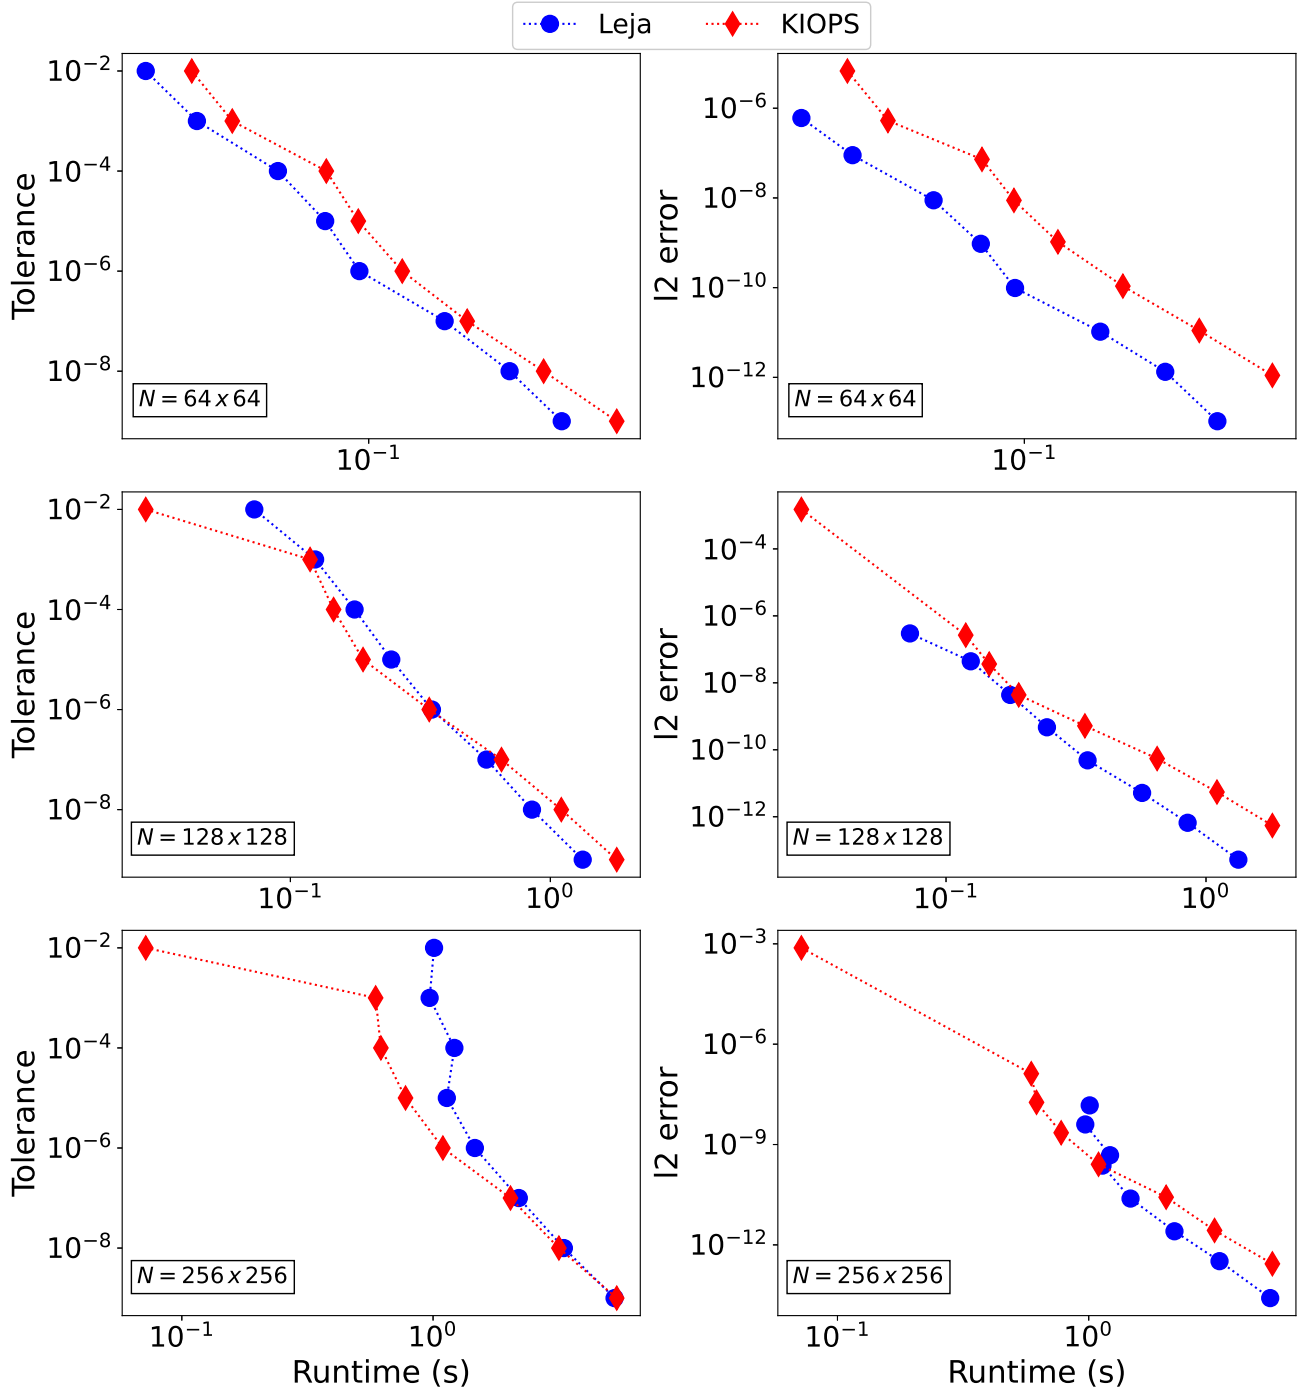

Figure 26: Comparison of the runtimes for a given value of tolerance (left panel) and the  $l_2$  norm of the global error incurred (right panel) for Leja (blue circles), LeKry (green pluses), and KIOPS (red diamonds) with the EXPRB43 integrator for the ADR equation ( $\alpha = 0.1$ ).

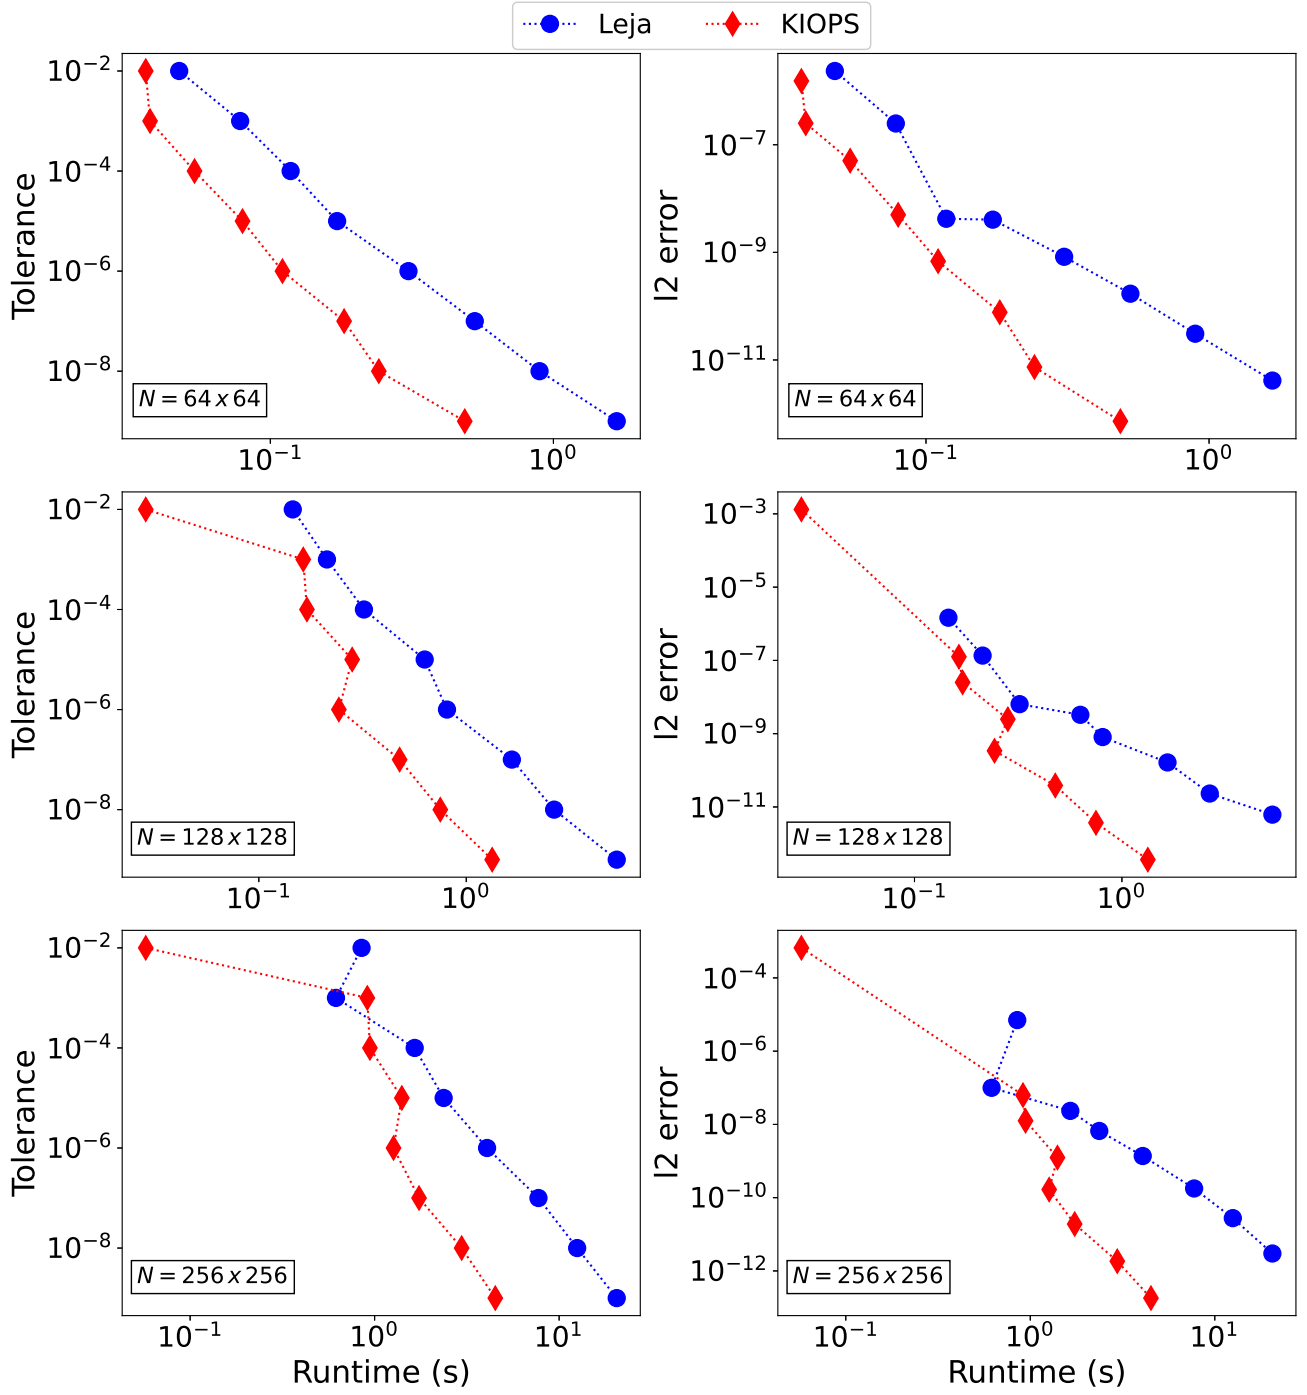

Figure 27: Comparison of the runtimes for a given value of tolerance (left panel) and the  $l_2$  norm of the global error incurred (right panel) for Leja (blue circles), LeKry (green pluses), and KIOPS (red diamonds) with the EXPRB43 integrator for the Allen-Cahn equation ( $\alpha = 0.01$ ).

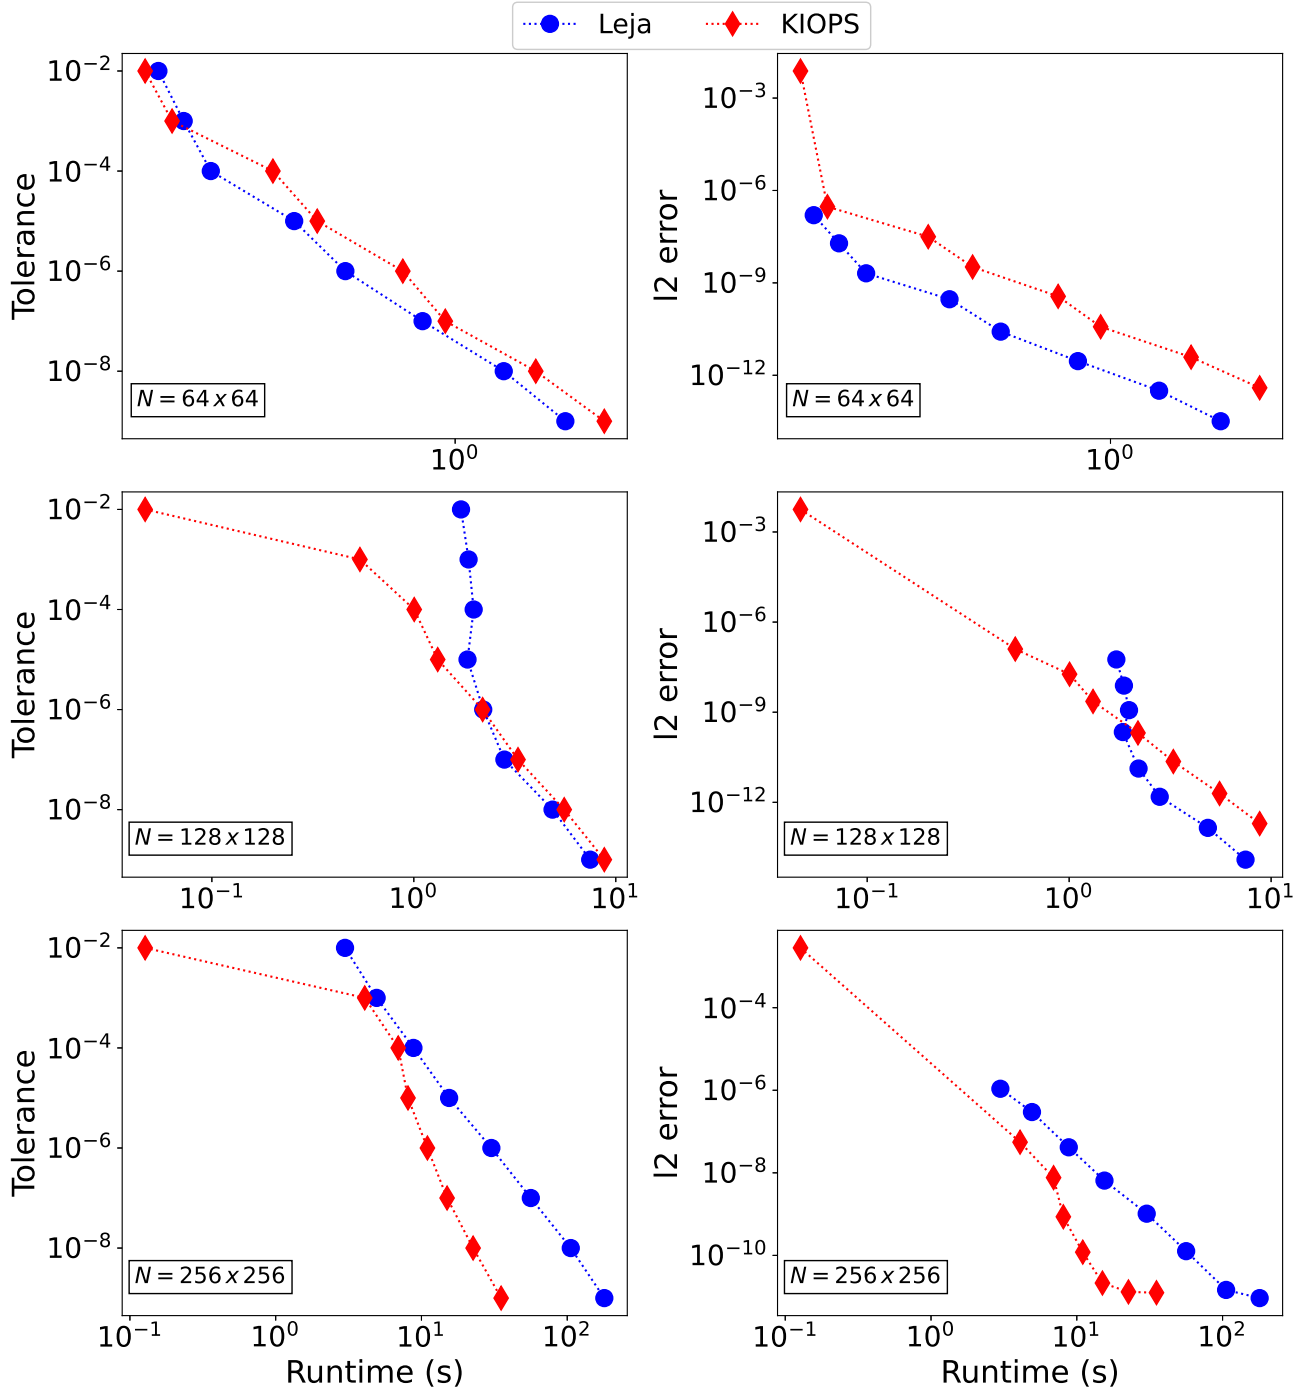

Figure 28: Comparison of the runtimes for a given value of tolerance (left panel) and the l2 norm of the global error incurred (right panel) for Leja (blue circles), LeKry (green pluses), and KIOPS (red diamonds) with the EXPRB43 integrator for the Brusselator equation ( $\alpha = 0.01$ ).

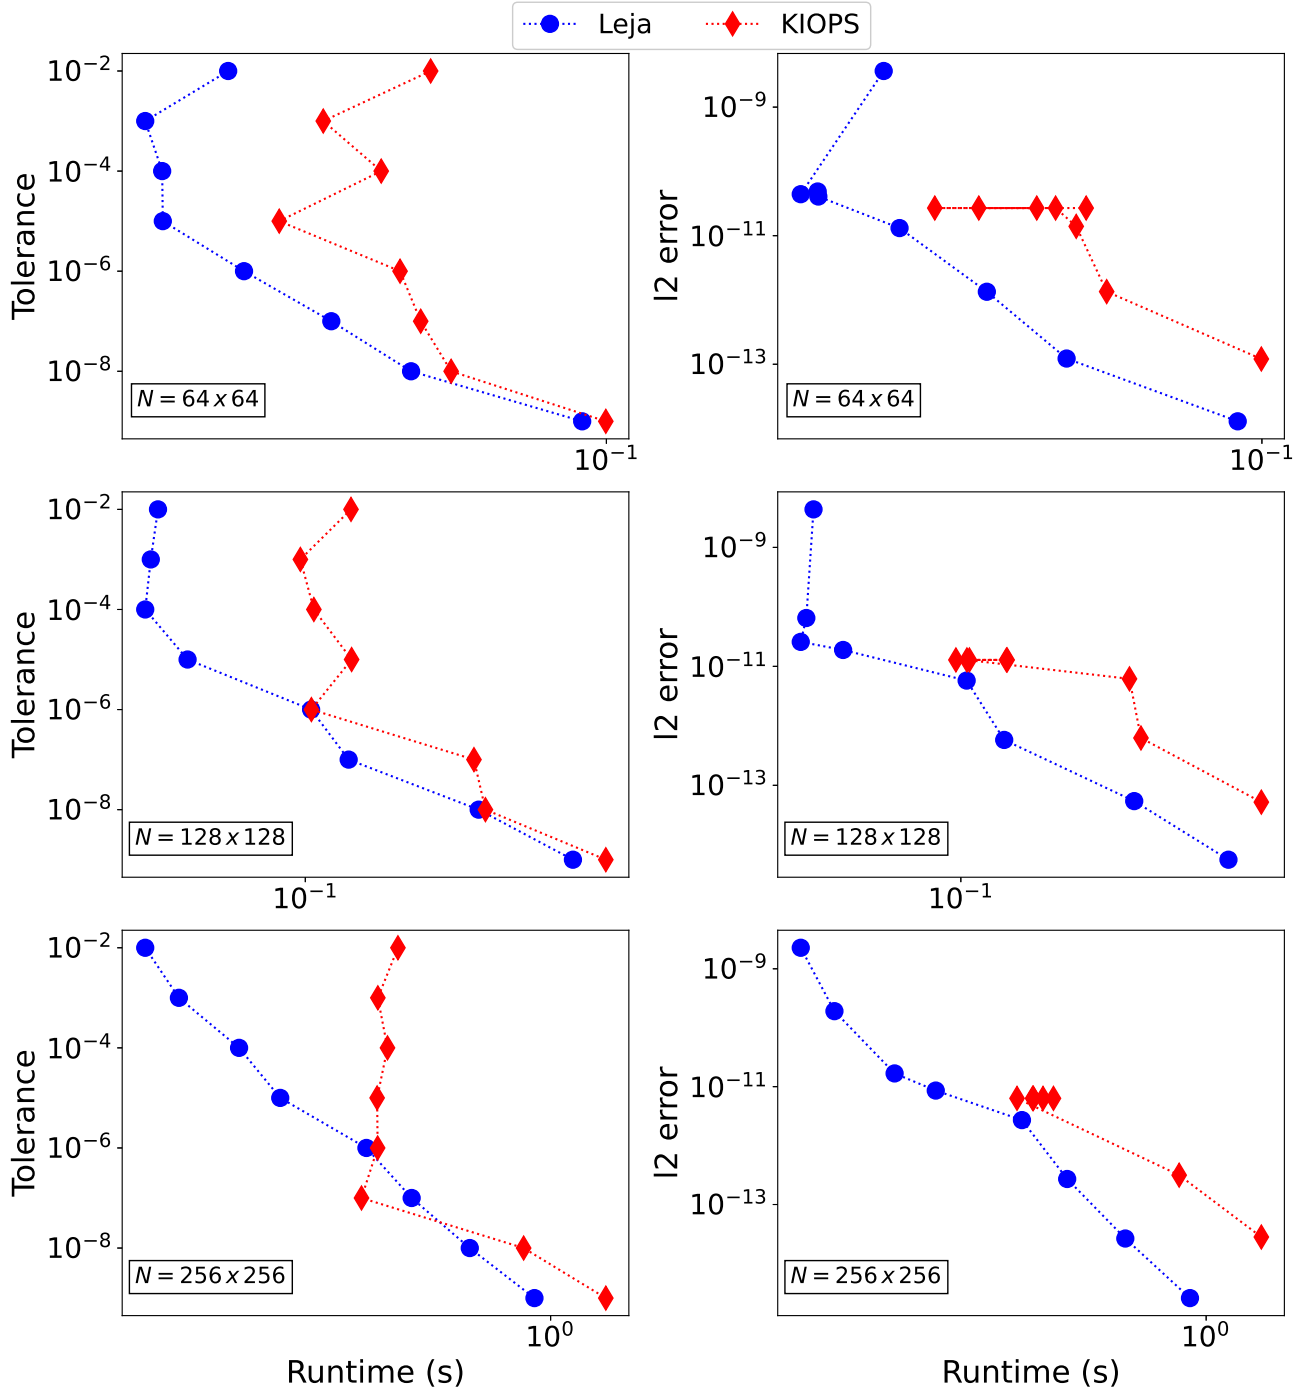

Figure 29: Comparison of the runtimes for a given value of tolerance (left panel) and the  $l_2$  norm of the global error incurred (right panel) for Leja (blue circles), LeKry (green pluses), and KIOPS (red diamonds) with the EXPRB43 integrator for the Gray-Scott equation ( $\alpha = 0.001$ ).

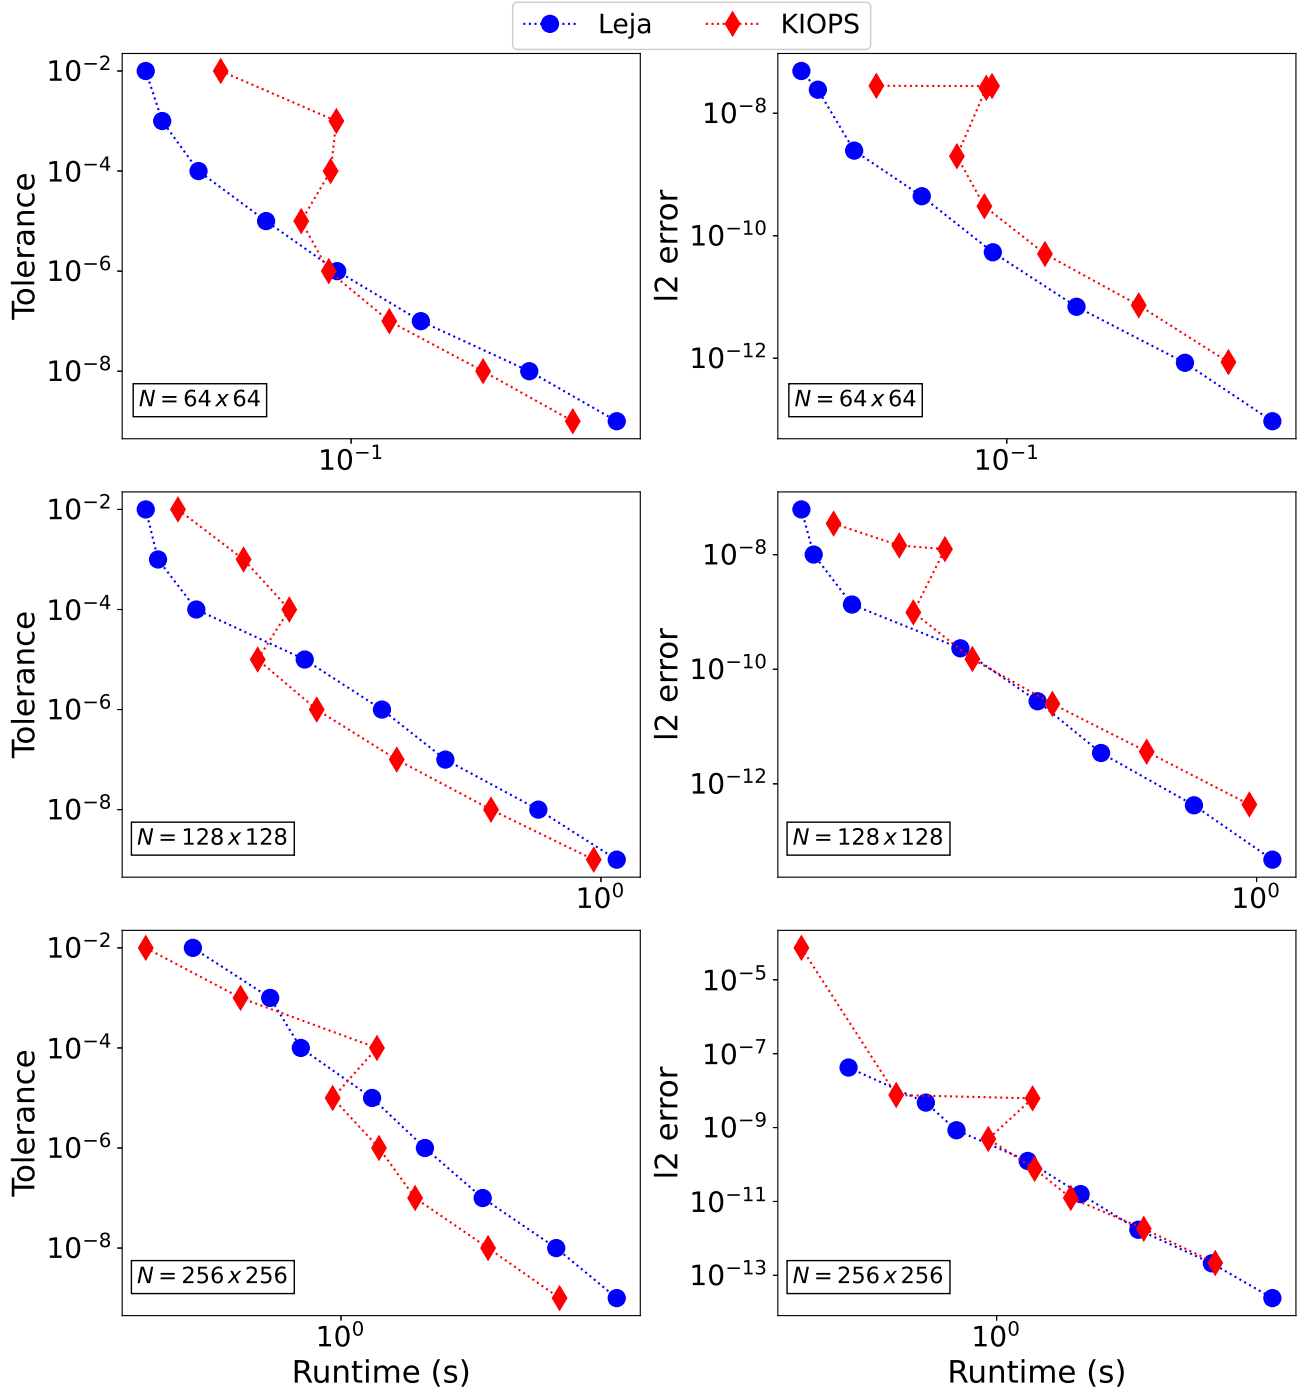

Figure 30: Comparison of the runtimes for a given value of tolerance (left panel) and the  $l_2$  norm of the global error incurred (right panel) for Leja (blue circles), LeKry (green pluses), and KIOPS (red diamonds) with the EXPRB43 integrator for the Gray-Scott equation ( $\alpha = 0.01$ ).

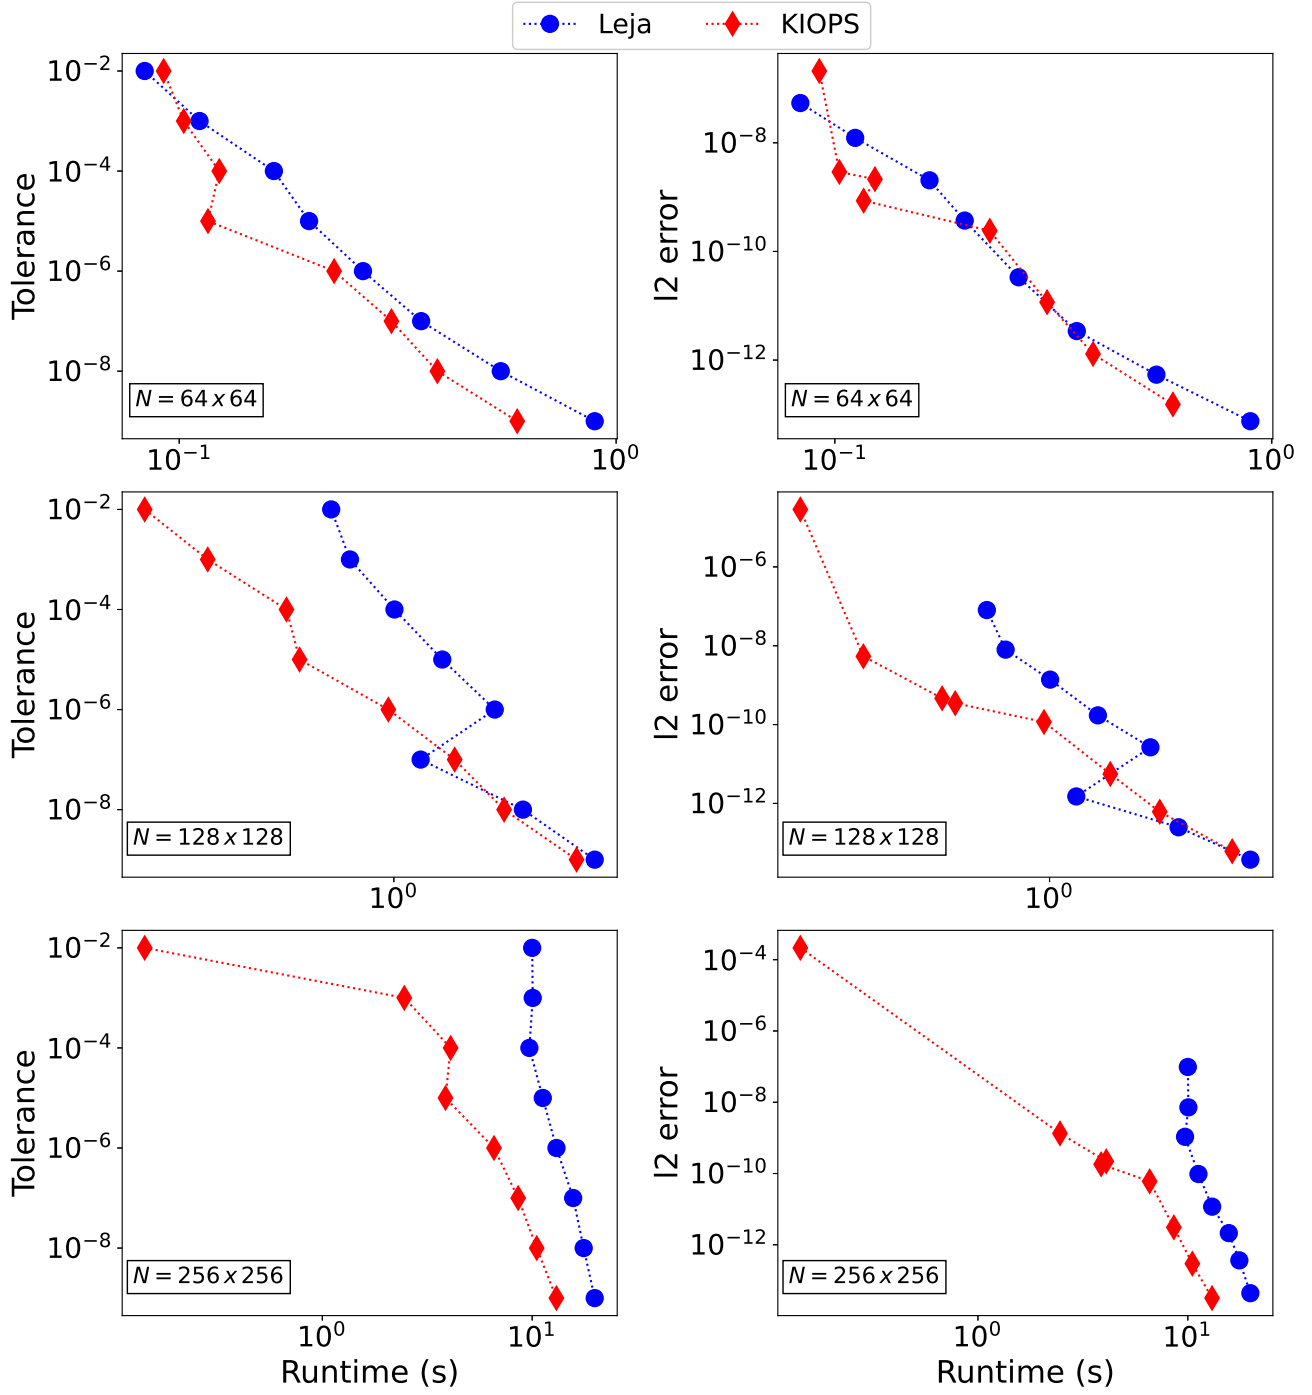

Figure 31: Comparison of the runtimes for a given value of tolerance (left panel) and the l2 norm of the global error incurred (right panel) for Leja (blue circles), LeKry (green pluses), and KIOPS (red diamonds) with the EXPRB43 integrator for the Gray-Scott equation ( $\alpha = 0.1$ ).



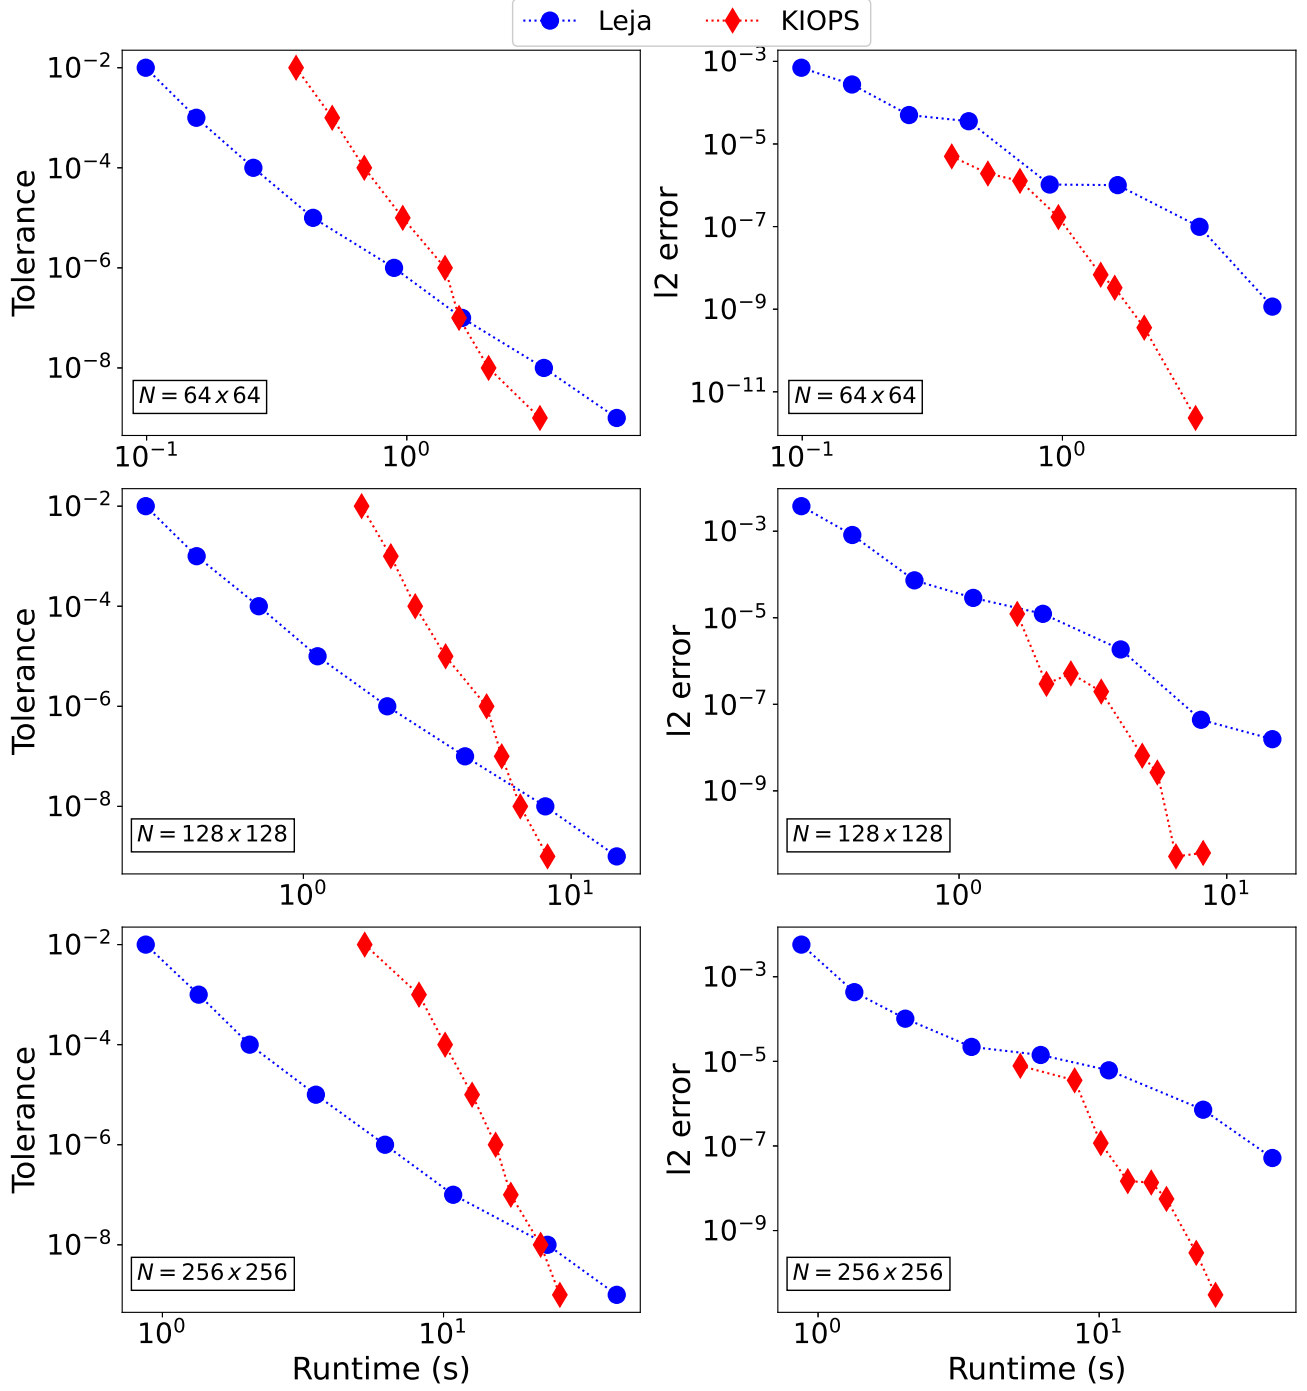

Figure 32: Comparison of the runtimes for a given value of tolerance (left panel) and the l2 norm of the global error incurred (right panel) for Leja (blue circles), LeKry (green pluses), and KIOPS (red diamonds) with the EXPRB43 integrator for the semilinear equation.

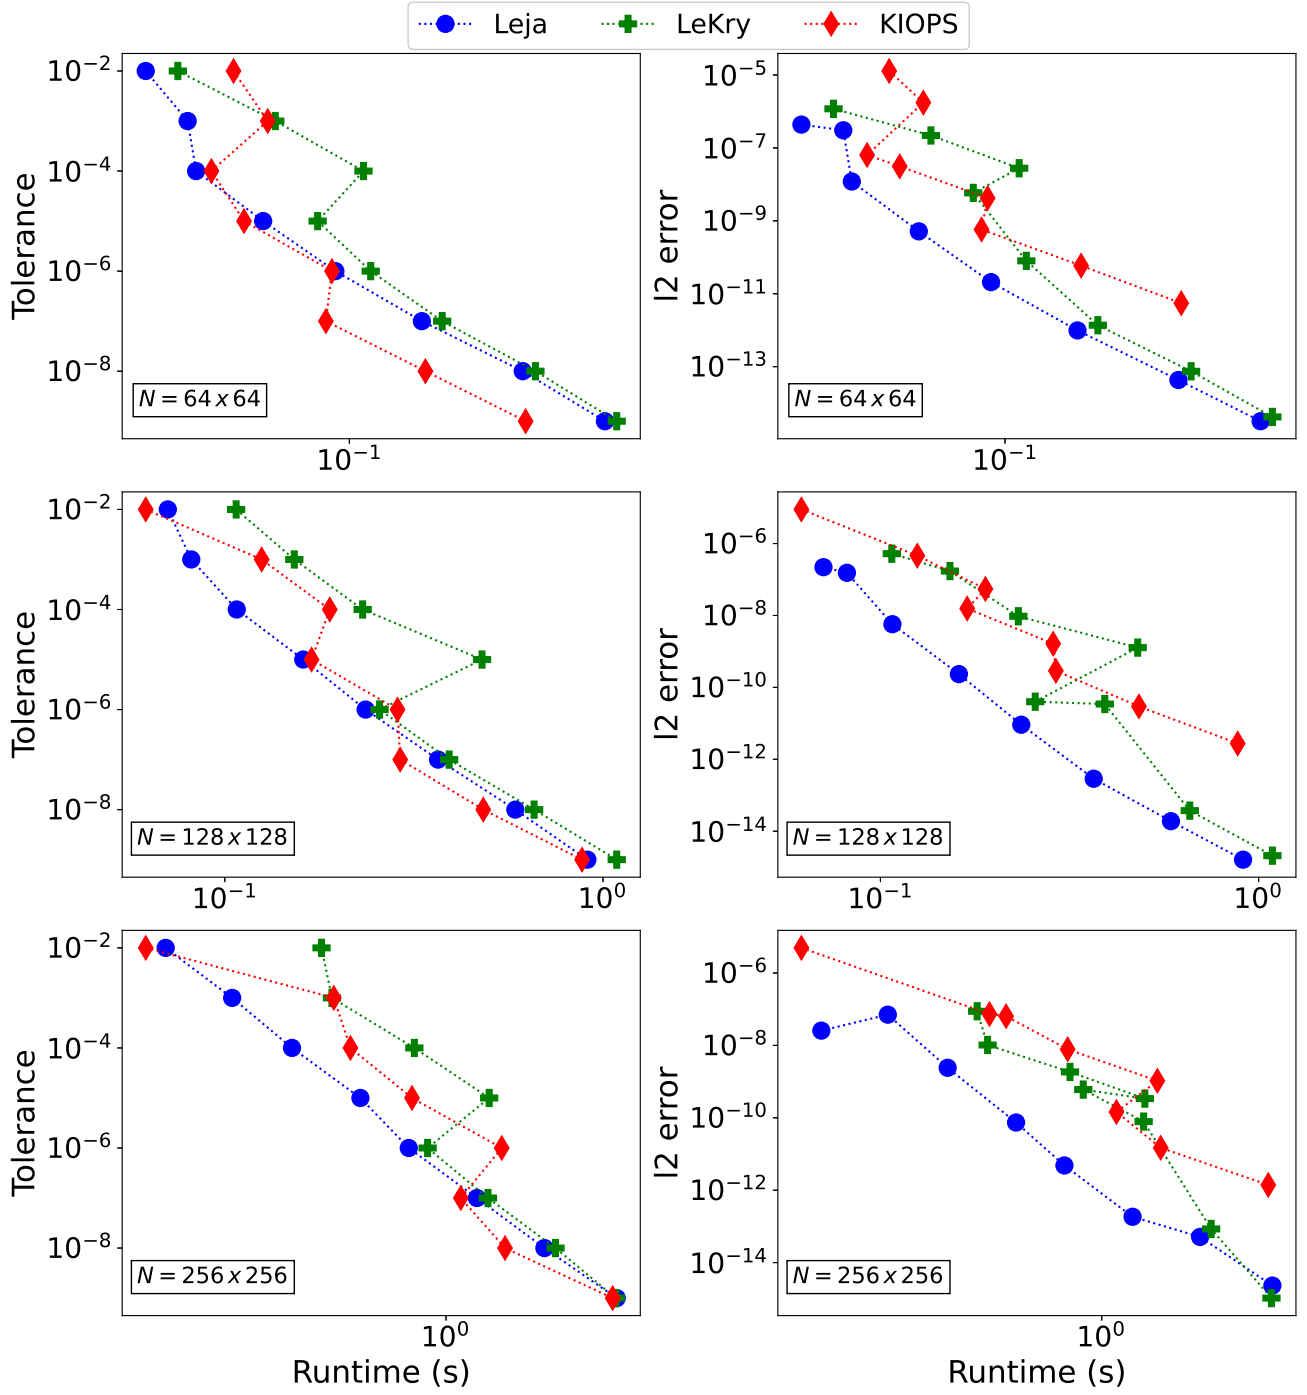

Figure 33: Comparison of the runtimes for a given value of tolerance (left panel) and the l2 norm of the global error incurred (right panel) for Leja (blue circles), LeKry (green pluses), and KIOPS (red diamonds) with the EXPRB53s3 integrator for the Allen-Cahn equation ( $\alpha = 0.001$ ).

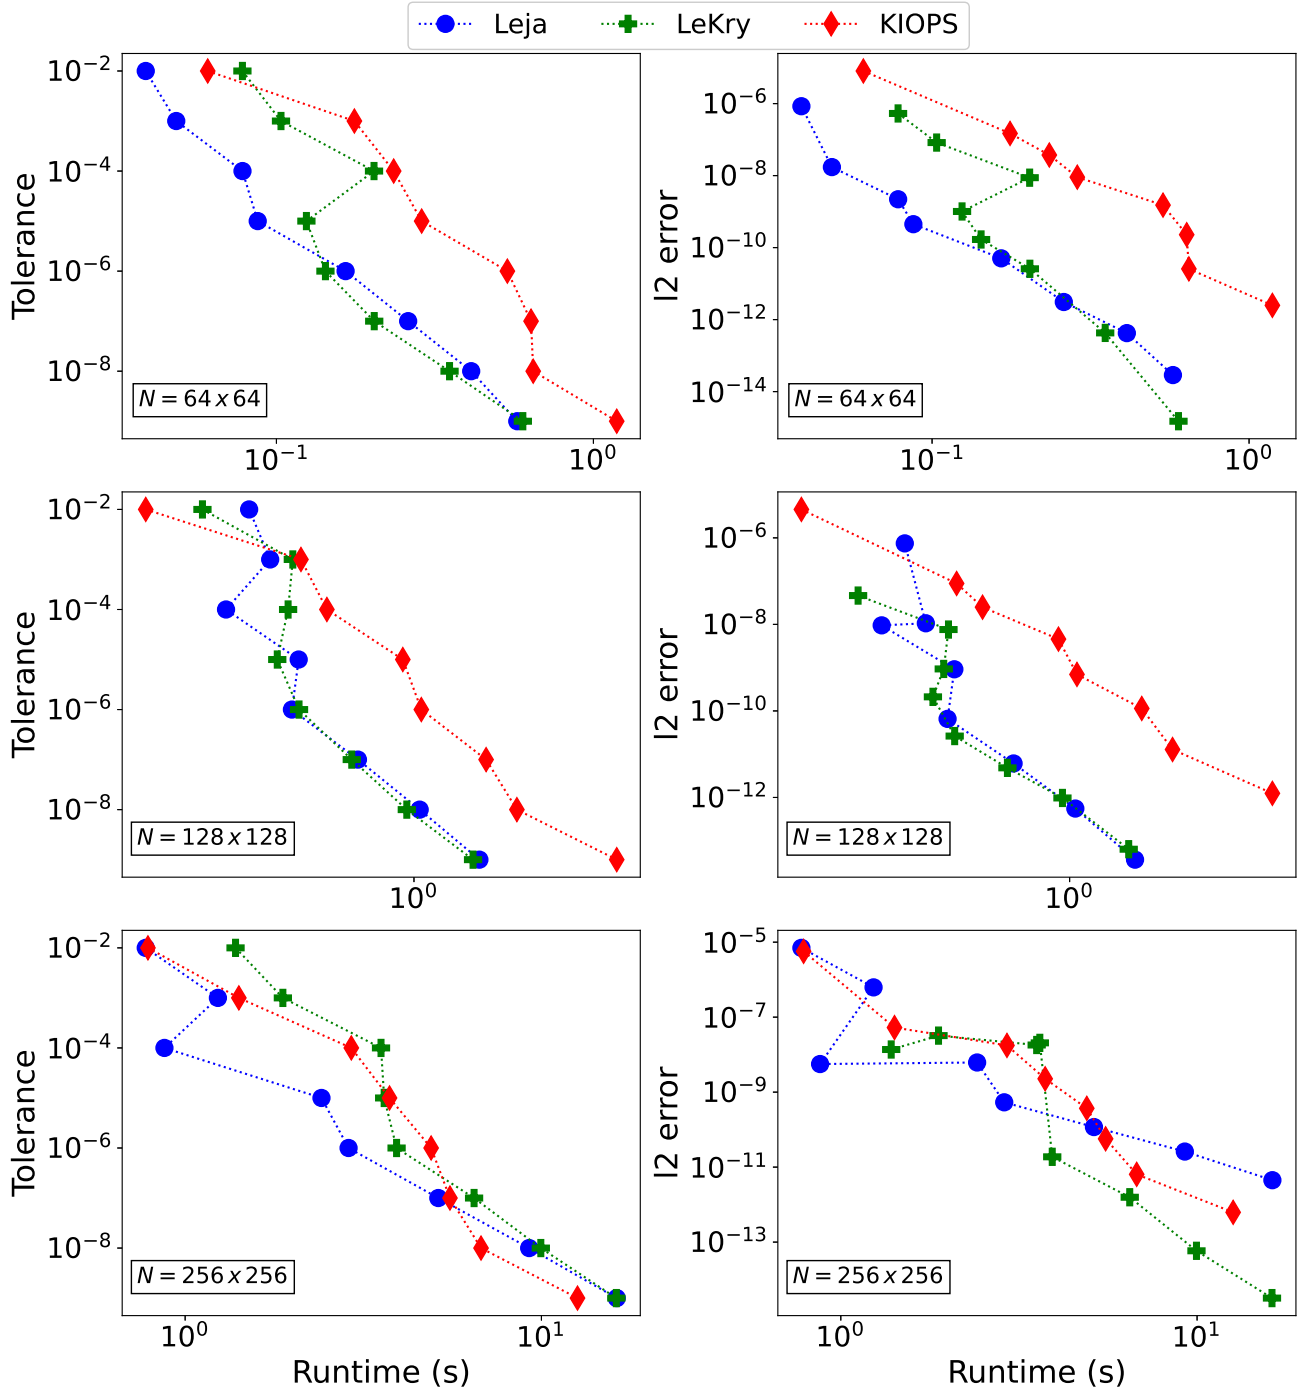

Figure 34: Comparison of the runtimes for a given value of tolerance (left panel) and the  $l_2$  norm of the global error incurred (right panel) for Leja (blue circles), LeKry (green pluses), and KIOPS (red diamonds) with the EXPRB53s3 integrator for the Allen-Cahn equation ( $\alpha = 0.01$ ).

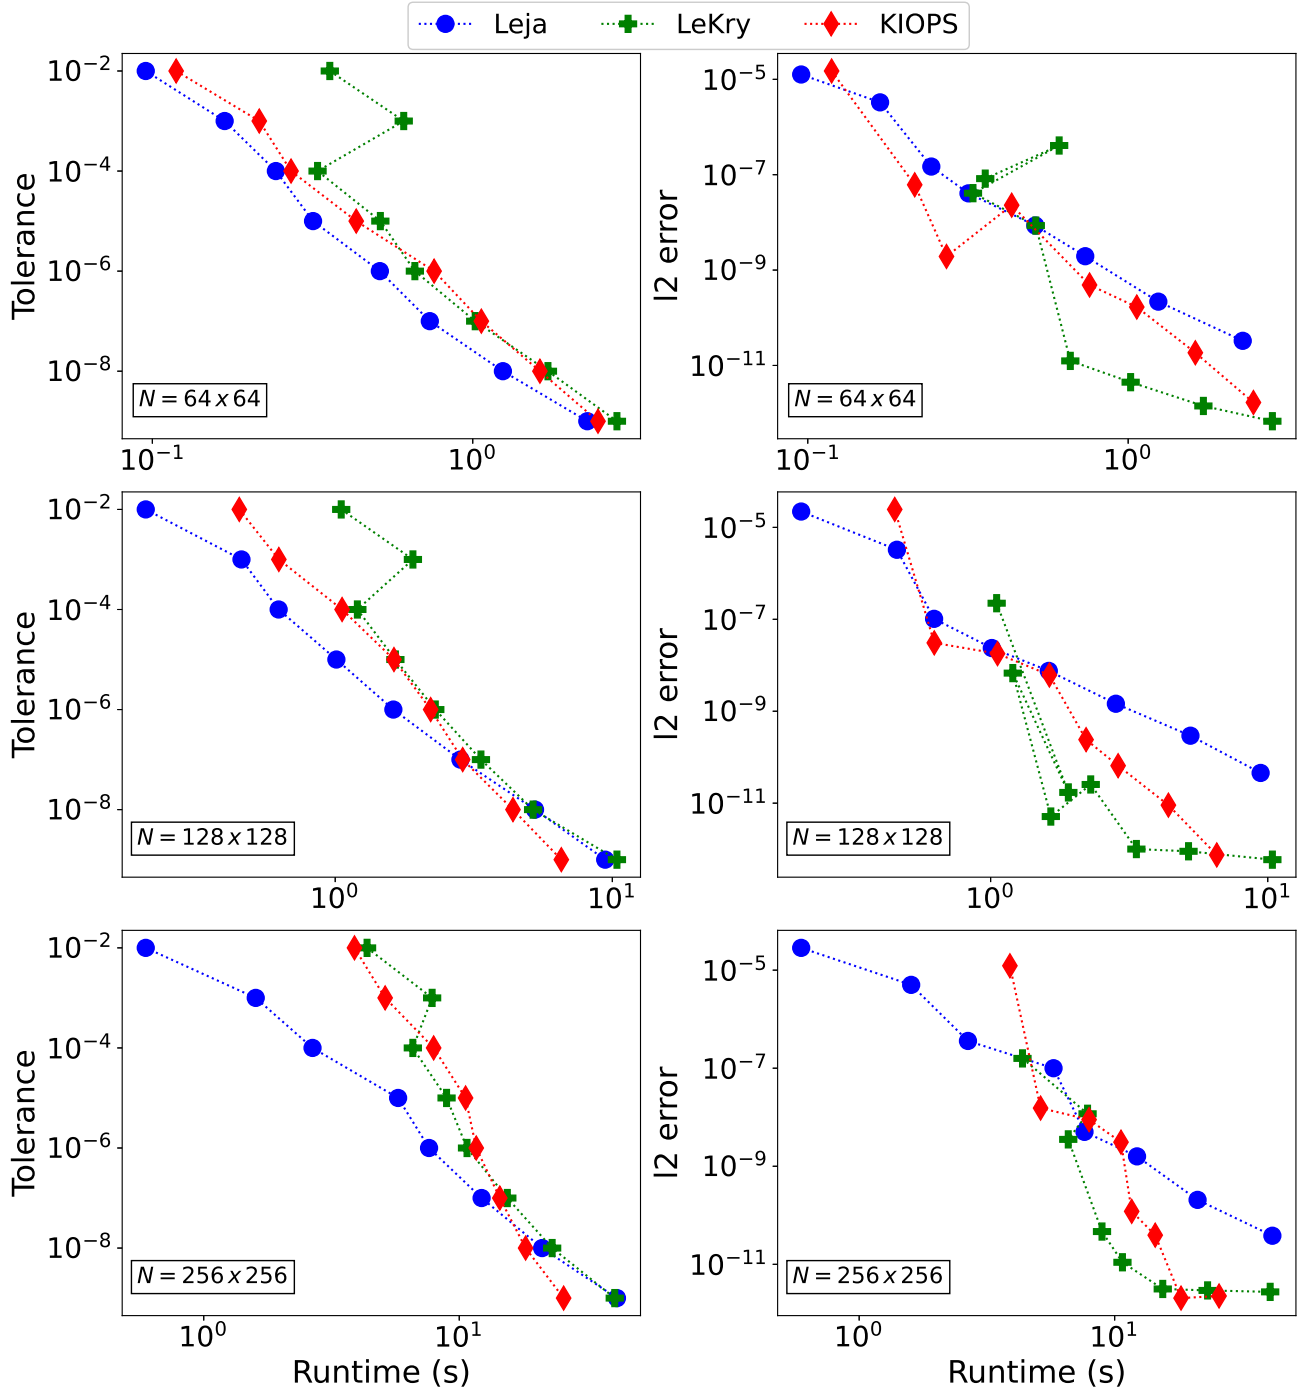

Figure 35: Comparison of the runtimes for a given value of tolerance (left panel) and the l2 norm of the global error incurred (right panel) for Leja (blue circles), LeKry (green pluses), and KIOPS (red diamonds) with the EXPRB53s3 integrator for the Allen–Cahn equation ( $\alpha = 0.1$ ).

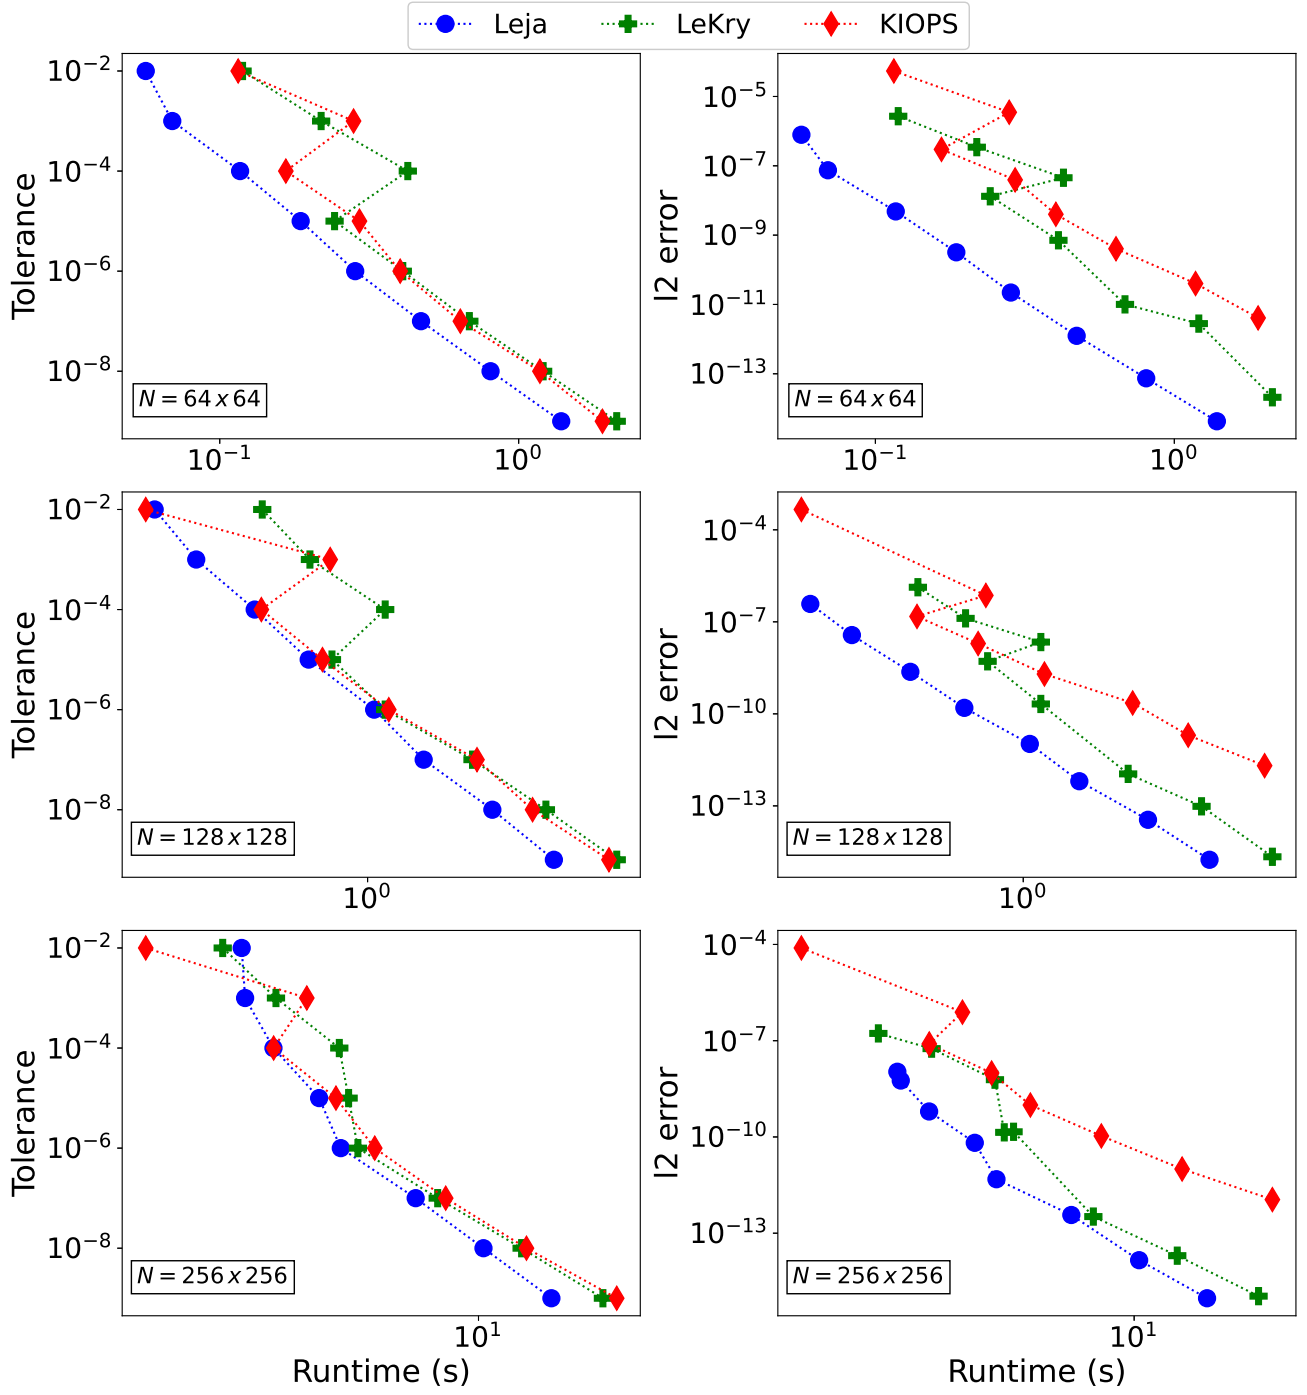

Figure 36: Comparison of the runtimes for a given value of tolerance (left panel) and the l2 norm of the global error incurred (right panel) for Leja (blue circles), LeKry (green pluses), and KIOPS (red diamonds) with the EXPRB53s3 integrator for the Brusselator equation ( $\alpha = 0.001$ ).

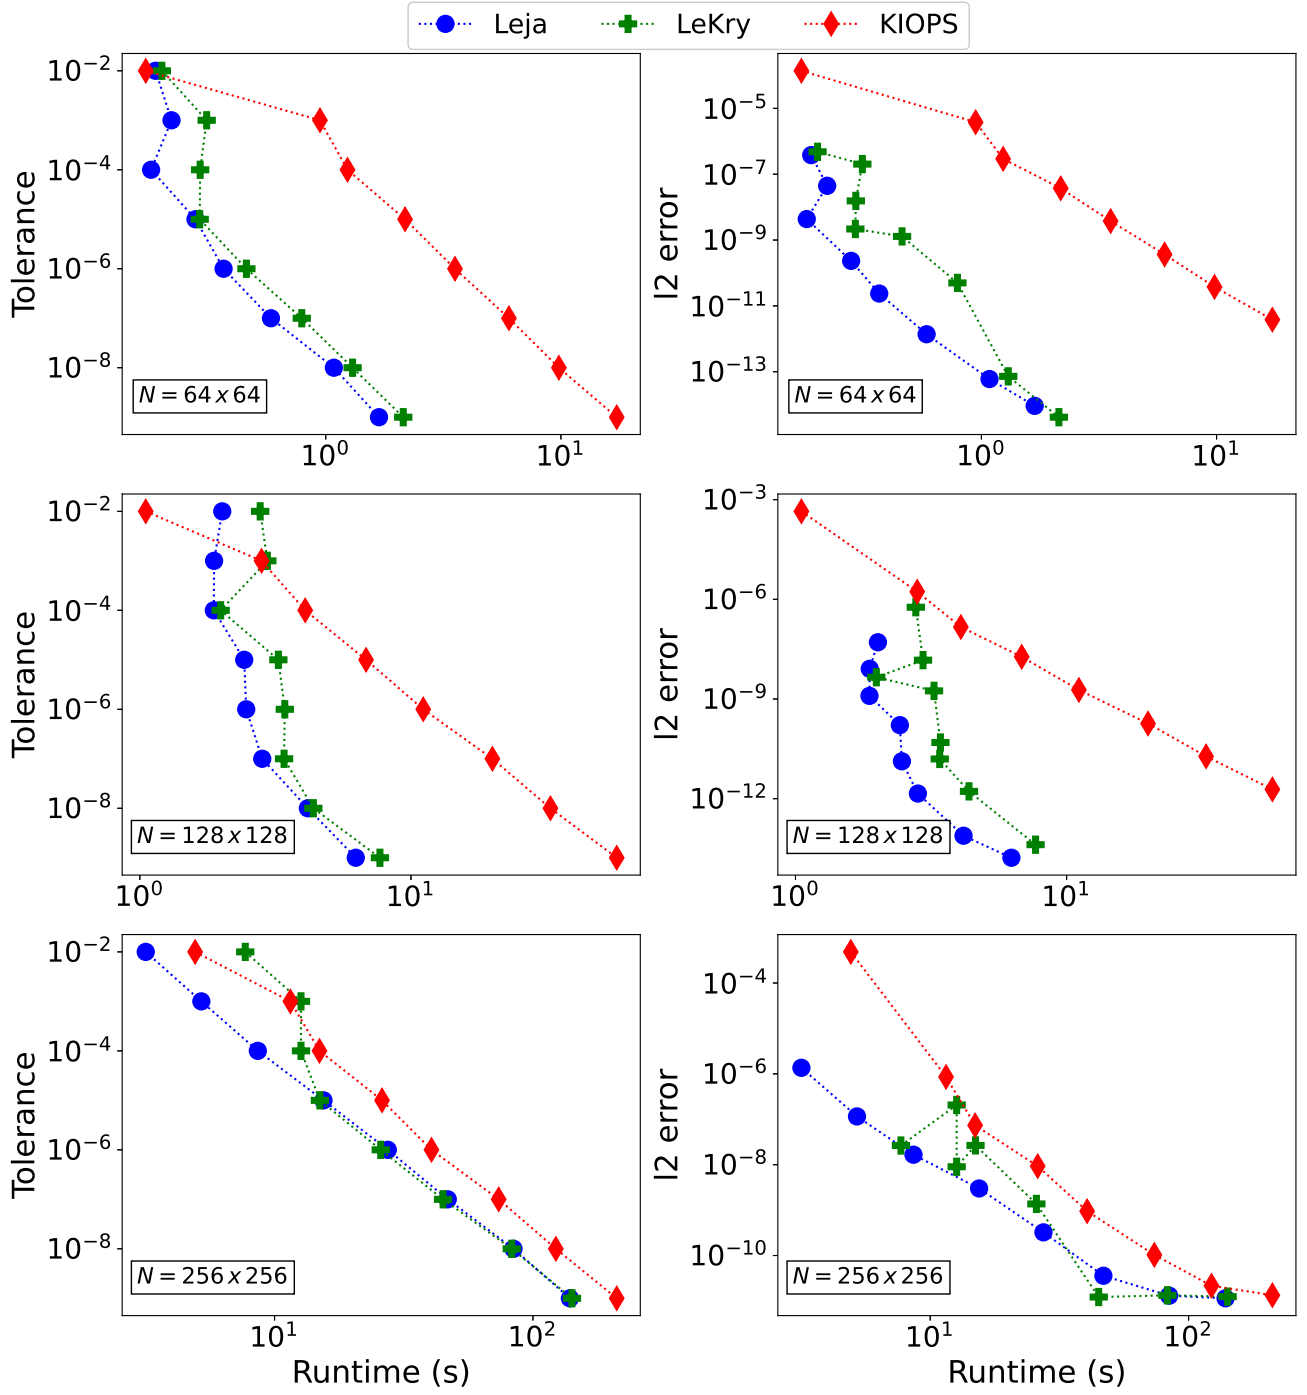

Figure 37: Comparison of the runtimes for a given value of tolerance (left panel) and the l2 norm of the global error incurred (right panel) for Leja (blue circles), LeKry (green pluses), and KIOPS (red diamonds) with the EXPRB53s3 integrator for the Brusselator equation ( $\alpha = 0.01$ ).

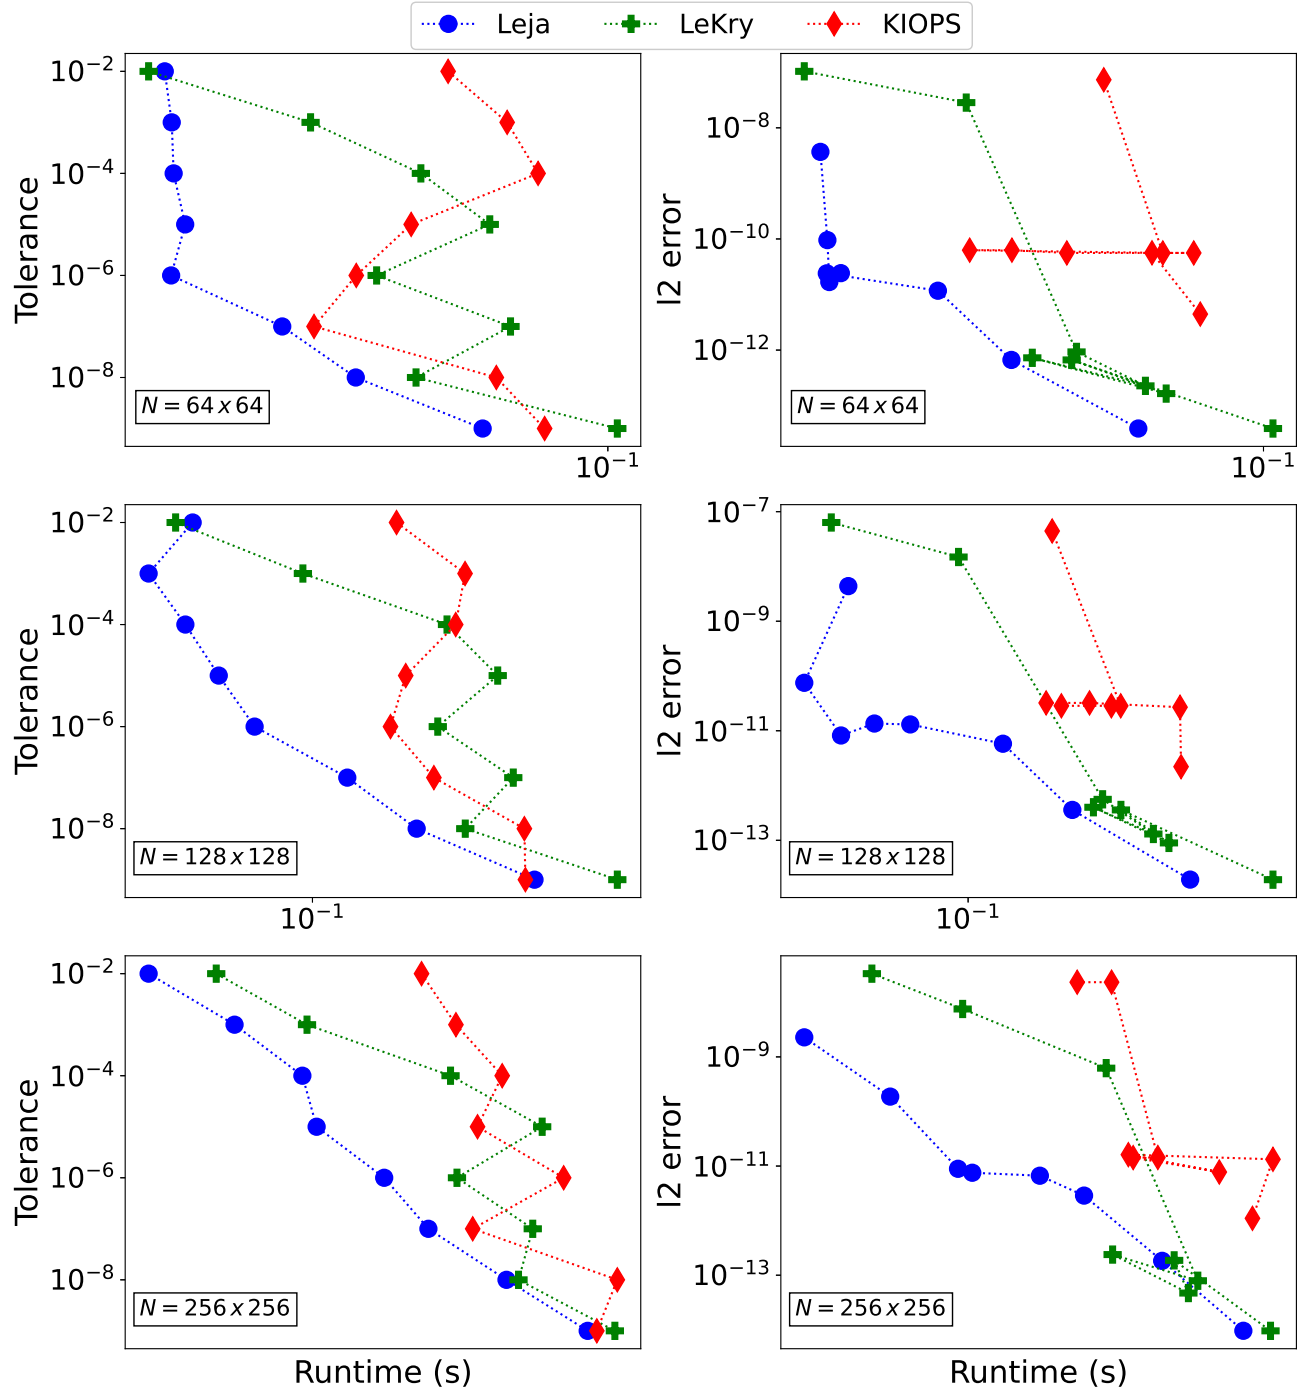

Figure 38: Comparison of the runtimes for a given value of tolerance (left panel) and the l2 norm of the global error incurred (right panel) for Leja (blue circles), LeKry (green pluses), and KIOPS (red diamonds) with the EXPRB53s3 integrator for the Gray-Scott equation ( $\alpha = 0.001$ ).

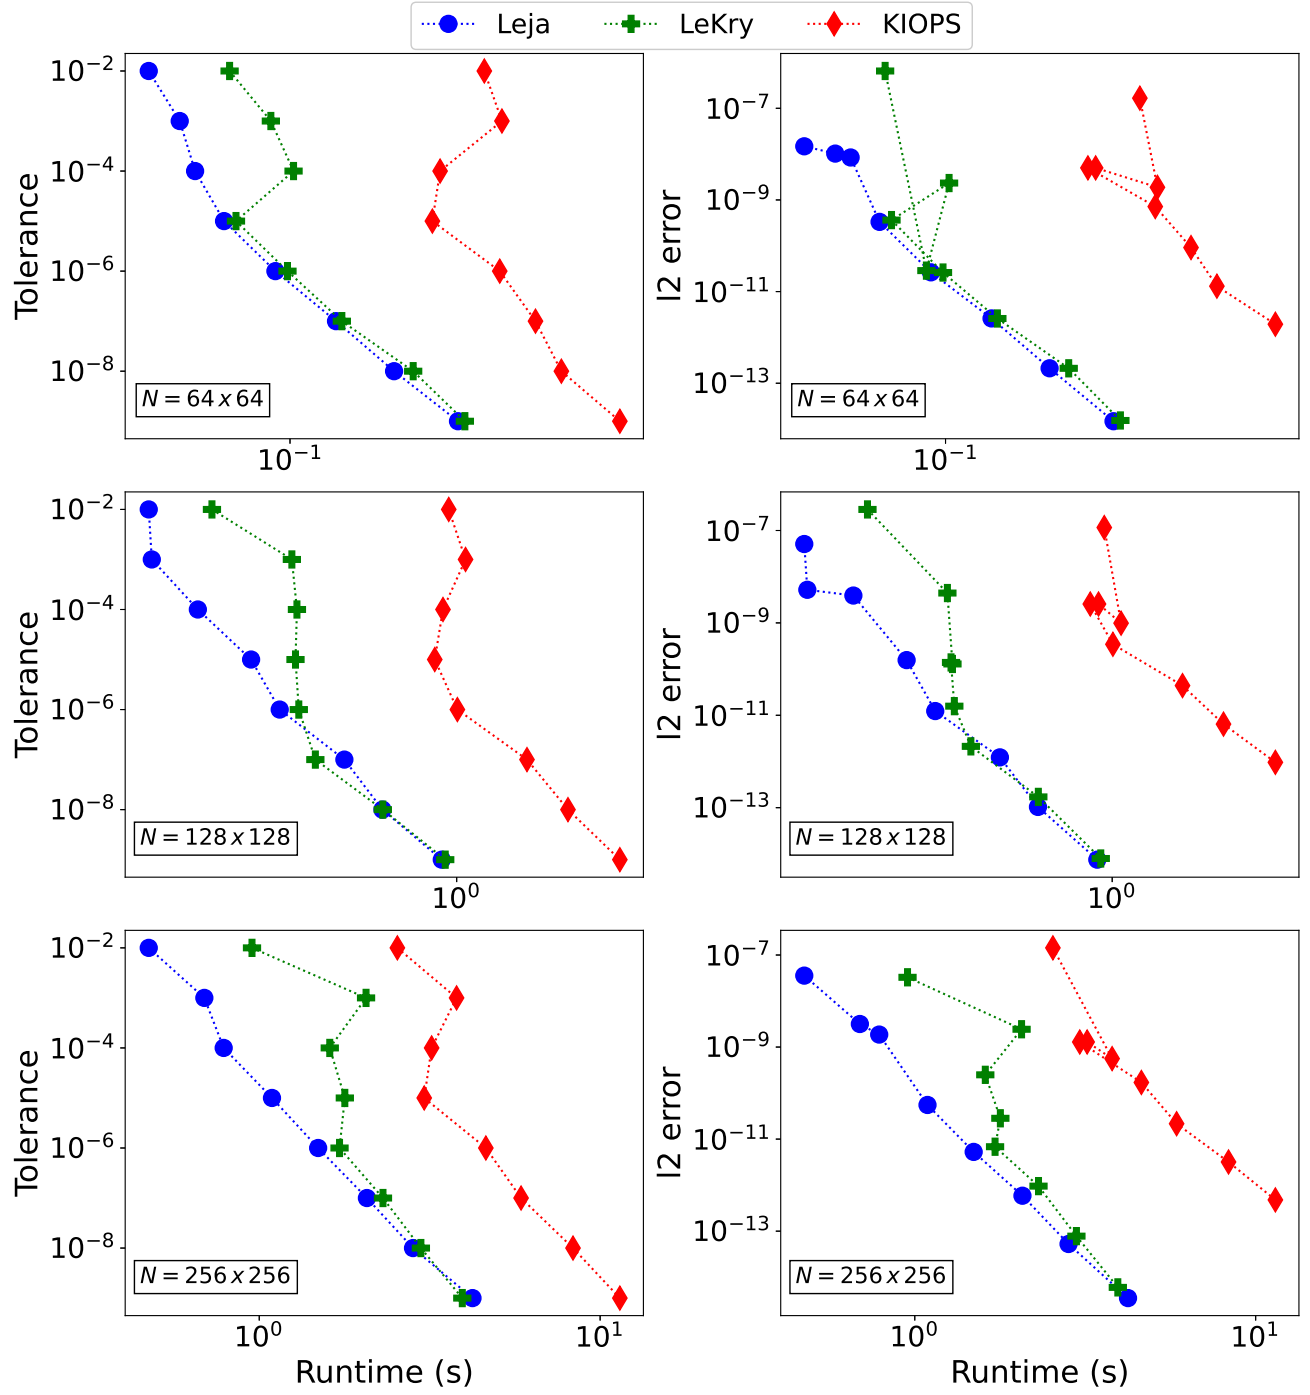

Figure 39: Comparison of the runtimes for a given value of tolerance (left panel) and the l2 norm of the global error incurred (right panel) for Leja (blue circles), LeKry (green pluses), and KIOPS (red diamonds) with the EXPRB53s3 integrator for the Gray-Scott equation ( $\alpha = 0.01$ ).



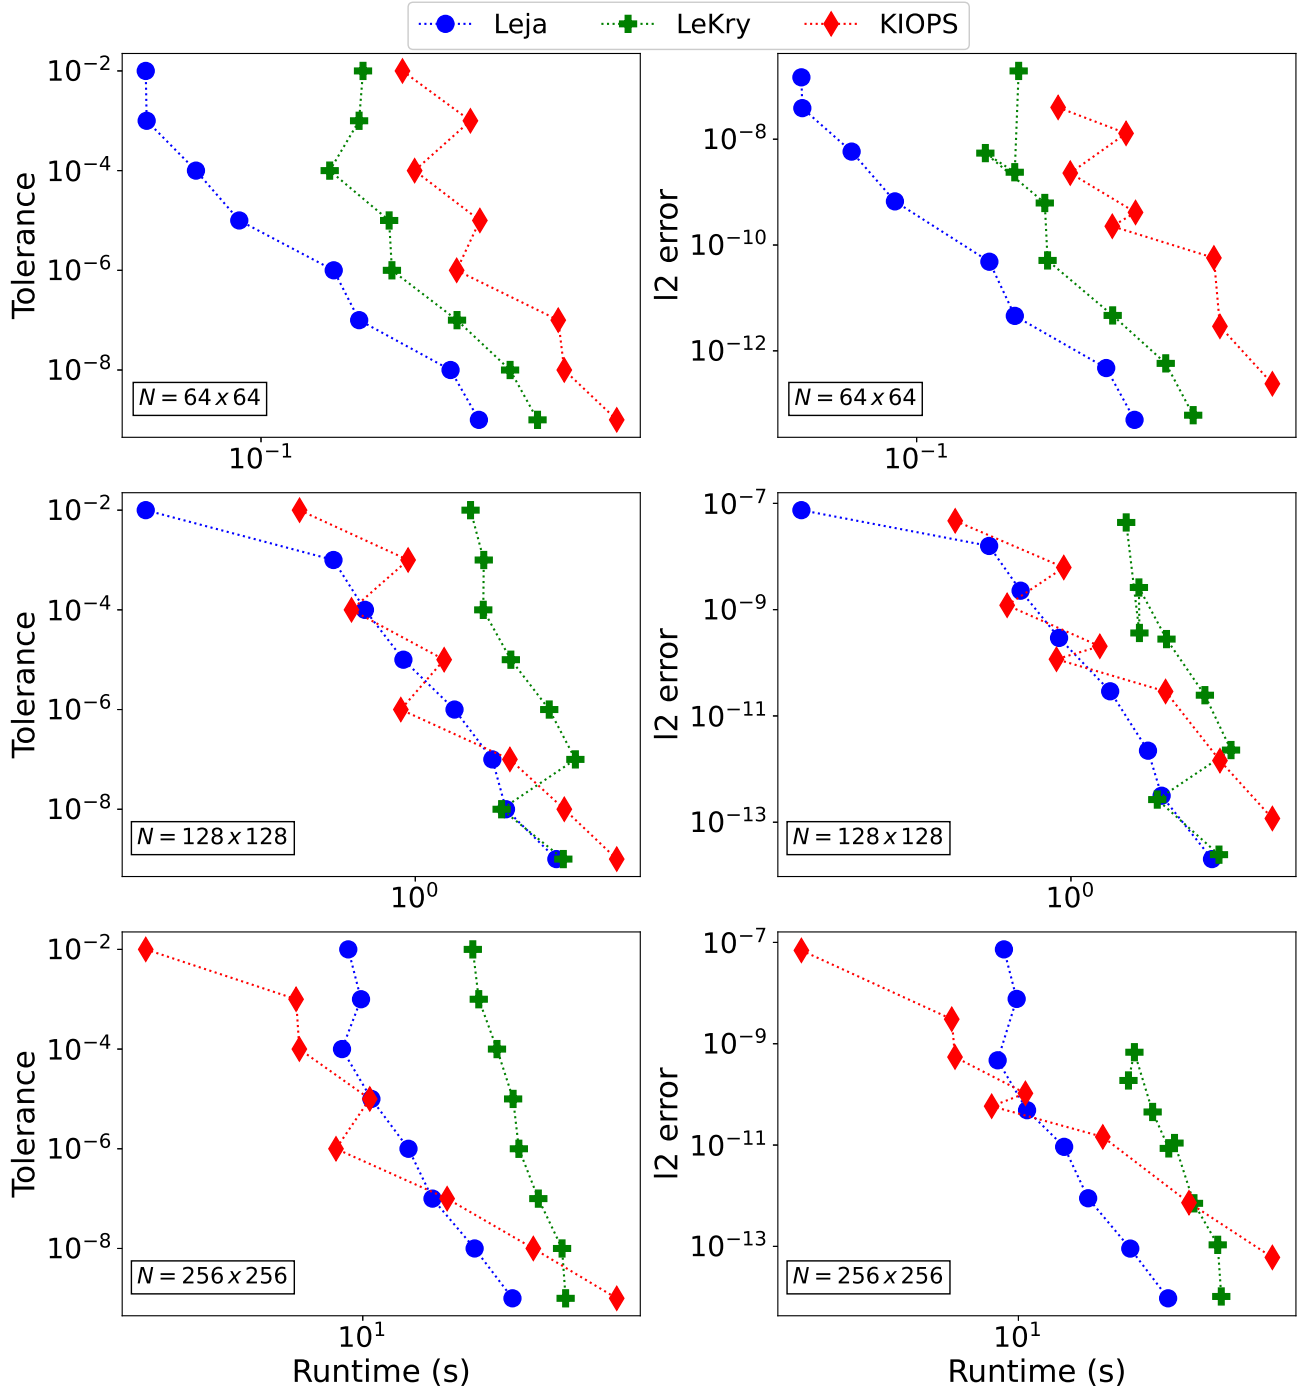

Figure 40: Comparison of the runtimes for a given value of tolerance (left panel) and the l2 norm of the global error incurred (right panel) for Leja (blue circles), LeKry (green pluses), and KIOPS (red diamonds) with the EXPRB53s3 integrator for the Gray-Scott equation ( $\alpha = 0.1$ ).
